# Supplementary material for: A Theory of Localized Excitations in Supercooled Liquids
Source: arXiv:2103.03015 ancillary file (2021-09-28)
Supplement: Supplementary file 1 [file SM_Excitations.pdf]

# Supplemental Material

## A Theory of Localized Excitations in Supercooled Liquids

Muhammad R. Hasyim<sup>1,†</sup>

Kranthi K. Mandadapu<sup>1,2,‡</sup>

<sup>1</sup>Department of Chemical & Biomolecular Engineering, University of California, Berkeley, CA 94720

<sup>2</sup>Chemical Sciences Division, Lawrence Berkeley National Laboratory, Berkeley, CA, USA

### Contents

|                   |                                                                             |           |
|-------------------|-----------------------------------------------------------------------------|-----------|
| <b>1</b>          | <b>Elasticity of Inherent States in Supercooled Liquids</b>                 | <b>1</b>  |
| 1.1               | Obtaining a Field Theory of Elastic Fluctuations . . . . .                  | 1         |
| 1.2               | Deriving the Elasticity Tensor $C_{ijkl}$ . . . . .                         | 8         |
| <b>2</b>          | <b>A Rate Theory for Elastic Dipole Excitations</b>                         | <b>15</b> |
| 2.1               | Review of Force Dipoles in Elasticity Theory . . . . .                      | 15        |
| 2.2               | Computing the Energy Barrier for a Configuration of Force Dipoles . . . . . | 21        |
| <b>3</b>          | <b>Connecting Excitations to Local Structure</b>                            | <b>23</b> |
| 3.1               | The Eigenstrain and T1 Transition . . . . .                                 | 24        |
| 3.2               | Determining $u^\ddagger$ from Radial Distribution Functions . . . . .       | 27        |
| <b>4</b>          | <b>Testing the Theory and Computational Methods</b>                         | <b>31</b> |
| 4.1               | Swap Monte Carlo Simulation . . . . .                                       | 32        |
| 4.2               | Inherent-State Sampling . . . . .                                           | 34        |
| 4.3               | Shear Modulus Calculation . . . . .                                         | 35        |
| 4.4               | Inherent-State RDF Calculation . . . . .                                    | 38        |
| 4.5               | MD Simulations and $\tau_{\text{eq}}(T)$ calculation . . . . .              | 38        |
| 4.6               | DF Theory Trajectory Analysis . . . . .                                     | 40        |
| <b>References</b> |                                                                             | <b>44</b> |

---

<sup>†</sup> muhammad\_hasyim@berkeley.edu

<sup>‡</sup> kranthi@berkeley.edu

# 1 Elasticity of Inherent States in Supercooled Liquids

A field theory for elastic fluctuations about inherent states is derived in Section 1.1 by analyzing the canonical partition function and coarse-graining the microscopic degrees of freedom into continuous fields. This theory provides an elastic strain energy, whose elasticity tensor  $C_{ijkl}$  is computable from sampled inherent-state configurations  $\{\mathbf{R}^\alpha\}$ . The explicit formula for  $C_{ijkl}$  is derived in Section 1.2.

## 1.1 Obtaining a Field Theory of Elastic Fluctuations

We start from the canonical partition function  $Z$  for  $N$ -many indistinguishable particles in  $d$ -dimensions

$$Z = \frac{1}{\lambda^{Nd} N!} \int \prod_{\alpha=1}^N d^d \mathbf{r}^\alpha e^{-\beta U(\{\mathbf{r}^\alpha\})} \quad (1)$$

where  $\lambda$  is the thermal de Broglie wavelength. In a multi-component system, the factor  $N!$  in  $Z$  can be replaced by  $\prod_{i=1}^M N_i!$ , where  $M$  is the number of components and  $N_i$  is the total number of particles in the  $i$ -th component. The potential energy is

$$U(\{\mathbf{r}^\alpha\}) = \sum_{\alpha, \beta} \phi(r^{\alpha\beta}) \quad (2)$$

where  $\phi(r^{\alpha\beta})$  is the pair potential, and  $r^{\alpha\beta} = |\mathbf{r}^\alpha - \mathbf{r}^\beta|$  is the pair distance between  $\alpha$ -th and  $\beta$ -th particle<sup>‡</sup>. Using Eq. (2), we can define an inherent-state configuration  $\{\mathbf{R}^\alpha\}$  as the configuration which minimizes the potential energy:

$$-\left. \frac{\partial U(\{\mathbf{r}^\alpha\})}{\partial \mathbf{r}^\alpha} \right|_{\{\mathbf{R}^\alpha\}} \equiv \mathbf{F}^\alpha(\{\mathbf{R}^\alpha\}) = 0 \quad (3)$$

where  $\mathbf{F}^\alpha(\{\mathbf{r}^\alpha\})$  is the total force on the  $\alpha$ -th particle. Note that in a deeply supercooled liquid, configurations  $\mathbf{r}^\alpha$  has a corresponding inherent state  $\mathbf{R}^\alpha$  obtained by finding the minimum energy configuration [1]; see Figure 1 in the main text.

Equation (1) encodes all fluctuations of the liquid, including elastic fluctuations about inherent states. To bring these fluctuations explicitly into  $Z$ , the integral  $\int \prod_{\alpha=1}^N d^d \mathbf{r}^\alpha$  can be broken into  $N_{\text{IS}}$ -many integrals where  $N_{\text{IS}}$  is the total number of inherent states [2]. As illustrated in Fig. S.1, the trick is to divide the total phase space into  $N_{\text{IS}}$ -many Voronoi cells, each of which has a unique inherent state at its center. Letting  $\mathcal{C}$  be the collection of all inherent states and  $\mathcal{P}(\{\mathbf{R}^\alpha\})$  be a Voronoi cell centered at  $\{\mathbf{R}^\alpha\} \in \mathcal{C}$ ,  $Z$  can be computed by integrating the Boltzmann factor  $e^{-\beta U(\{\mathbf{r}^\alpha\})}$  in every  $\mathcal{P}(\{\mathbf{R}^\alpha\})$  and summing these integrals over all inherent states  $\{\mathbf{R}^\alpha\} \in \mathcal{C}$ :

$$Z = \frac{1}{\lambda^{Nd} N!} \sum_{\{\mathbf{R}^\alpha\} \in \mathcal{C}} \int_{\mathcal{P}(\{\mathbf{R}^\alpha\})} \prod_{\alpha=1}^N d^d \mathbf{r}^\alpha e^{-\beta U(\{\mathbf{r}^\alpha\})}. \quad (4)$$

The potential energy in Eq. (2) can be decomposed into two parts

$$U(\{\mathbf{r}^\alpha\}; \{\mathbf{R}^\alpha\}) = U(\{\mathbf{R}^\alpha\}) + \Delta U(\{\mathbf{r}^\alpha\}; \{\mathbf{R}^\alpha\}) \quad (5)$$

where  $U(\{\mathbf{R}^\alpha\})$  is the reference energy corresponding to the inherent state of  $\mathbf{r}^\alpha$ , and  $\Delta U(\{\mathbf{r}^\alpha\}; \{\mathbf{R}^\alpha\})$  is the difference that contains both harmonic and anharmonic terms. Using this decomposition,

---

<sup>‡</sup>Herein, the summation over  $\alpha$  and  $\beta$  includes only a pair-wise sum where  $\alpha$  and  $\beta$  are not repeated.

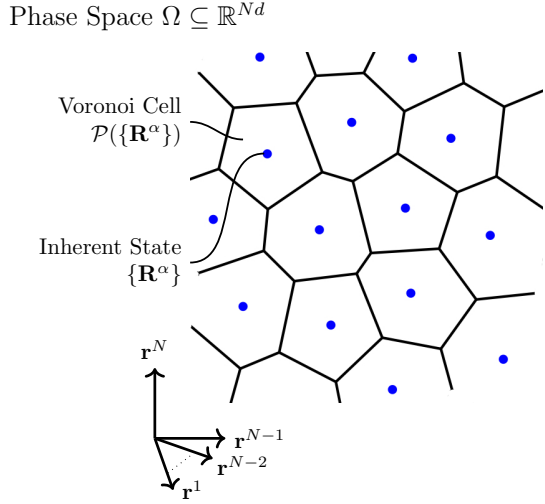

Figure S.1: An illustration of the phase space tessellated by a Voronoi network, which is constructed from available inherent states. The union of all Voronoi cells gives back the phase space. Thus, one can integrate over the phase space by integrating over every cell, and summing the result together.

Eq. (4) can be rearranged into

$$Z = \frac{1}{\lambda^{Nd} N!} \sum_{\{\mathbf{R}^\alpha\} \in \mathcal{C}} \left[ \int_{\mathcal{P}(\{\mathbf{R}^\alpha\})} \prod_{\alpha=1}^N d^d \mathbf{r}^\alpha e^{-\beta \Delta U(\{\mathbf{r}^\alpha\}; \{\mathbf{R}^\alpha\})} \right] e^{-\beta U(\{\mathbf{R}^\alpha\})}. \quad (6)$$

Introducing a new partition function  $Q_{\text{IS}}$  and its ensemble average  $\langle \dots \rangle_{\text{IS}}$  given by

$$Q_{\text{IS}} = \sum_{\{\mathbf{R}^\alpha\} \in \mathcal{C}} e^{-\beta U(\{\mathbf{R}^\alpha\})}; \quad \langle \dots \rangle_{\text{IS}} = \frac{1}{Q_{\text{IS}}} \sum_{\{\mathbf{R}^\alpha\} \in \mathcal{C}} \dots e^{-\beta U(\{\mathbf{R}^\alpha\})}, \quad (7)$$

Eq. (6) can be further simplified into

$$Z = \frac{Q_{\text{IS}}}{\lambda^{Nd} N!} \frac{1}{Q_{\text{IS}}} \sum_{\{\mathbf{R}^\alpha\} \in \mathcal{C}} \left[ \int_{\mathcal{P}(\{\mathbf{R}^\alpha\})} \prod_{\alpha=1}^N d^d \mathbf{r}^\alpha e^{-\beta \Delta U(\{\mathbf{r}^\alpha\}; \{\mathbf{R}^\alpha\})} \right] e^{-\beta U(\{\mathbf{R}^\alpha\})} \quad (8)$$

$$= \frac{Q_{\text{IS}}}{\lambda^{Nd} N!} \left\langle \int_{\mathcal{P}(\{\mathbf{R}^\alpha\})} \prod_{\alpha=1}^N d^d \mathbf{r}^\alpha e^{-\beta \Delta U(\{\mathbf{r}^\alpha\}; \{\mathbf{R}^\alpha\})} \right\rangle_{\text{IS}} \quad (9)$$

$$= \frac{1}{\lambda^{Nd} N!} Q_{\text{IS}} \overline{Q}_{\text{fln}} \quad (10)$$

where  $\overline{Q}_{\text{fln}}$  is a partition function that sums over fluctuations about all possible inherent states:

$$\overline{Q}_{\text{fln}} = \left\langle \int_{\mathcal{P}(\{\mathbf{R}^\alpha\})} \prod_{\alpha=1}^N d^d \mathbf{r}^\alpha e^{-\beta \Delta U(\{\mathbf{r}^\alpha\}; \{\mathbf{R}^\alpha\})} \right\rangle_{\text{IS}}. \quad (11)$$

Using Eq. (10), the free energy  $F \equiv -k_B T \ln Z$  of the system can be written as

$$F = k_B T \ln \left[ \lambda^{Nd} / N! \right] - k_B T \ln Q_{\text{IS}} - k_B T \ln \overline{Q}_{\text{fln}}. \quad (12)$$

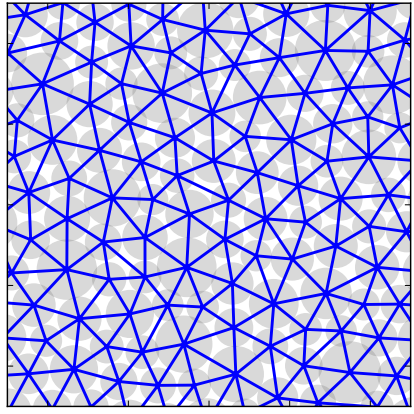

Figure S.2: A schematic of Delaunay triangulation of an inherent-state configuration providing a connection between particle displacements and the displacement field.

Ignoring the kinetic contribution ( $k_B T \ln [\lambda^{N_d}/N!]$ ), one can see that Eq. (12) is a sum of two parts. The first one ( $-k_B T \ln Q_{\text{IS}}$ ) emerges from the distribution of energy-well depths or inherent states while the second one ( $-k_B T \ln \bar{Q}_{\text{fln}}$ ) emerges from the effect of fluctuations about inherent states. At lower temperature, the latter can be used as a starting point for constructing a field theory of elastic fluctuations by applying a harmonic approximation with suitable coarse-graining. Such a field theory is useful as it brings insights from the theory of elasticity to understand the nature of localized excitations, and compute their energy barrier  $J_\sigma$  from elastic properties of inherent states.

The harmonic approximation allows us to replace the Boltzmann factor in Eq. (11) with a mixture of Gaussian distributions centered at every  $\{\mathbf{R}^\alpha\} \in \mathcal{C}$ . This along with larger stiffnesses around inherent state and lower temperatures further allow us to approximate the integration over the Voronoi cells in Eq. (11) with an unconstrained integration over the entire phase space. To this end, let  $\mathbf{u}^\alpha \equiv \mathbf{r}^\alpha - \mathbf{R}^\alpha$  be the particle displacement. Then applying the harmonic approximation to Eq. (11) yields

$$\bar{Q}_{\text{fln}} \approx \left\langle \int \prod_{\alpha=1}^N d^d \mathbf{u}^\alpha e^{-\beta \Delta U(\{\mathbf{u}^\alpha\}; \{\mathbf{R}^\alpha\})} \right\rangle_{\text{IS}} \quad (13)$$

where  $\Delta U(\{\mathbf{u}^\alpha\}; \{\mathbf{R}^\alpha\})$  contains only harmonic terms and the integral is over the entire phase space. Since the integral leading to Eq. (13) is now independent of  $\{\mathbf{R}^\alpha\}$ , one may move the ensemble average into the integrand:

$$\bar{Q}_{\text{fln}} \approx \int \prod_{\alpha=1}^N d^d \mathbf{u}^\alpha \left\langle e^{-\beta \Delta U(\{\mathbf{u}^\alpha\}; \{\mathbf{R}^\alpha\})} \right\rangle_{\text{IS}} \quad (14)$$

where  $\mathbf{u}^\alpha$  can be integrated irrespective of the choice of inherent-state configuration. In fact, one must average the Boltzmann factor  $e^{-\beta \Delta U(\{\mathbf{u}^\alpha\}; \{\mathbf{R}^\alpha\})}$  over all possible inherent states before integrating over  $\mathbf{u}^\alpha$ .

With the harmonic approximation in place, we now provide an idea for the coarse-graining process by which Eq. (14) can be turned into a field-theoretic partition function, whose degrees of freedom are a set of continuous displacement fields  $\mathbf{u}(\mathbf{x})$ , given by

$$\bar{Q}_{\text{fln}} \approx \int \mathcal{D}\mathbf{u} e^{-\beta \Delta F[\mathbf{u}]}, \quad (15)$$

where  $\mathcal{D}\mathbf{u}$  is the functional measure. The free energy functional  $\Delta F[\mathbf{u}]$  serves as an effective Hamiltonian for elastic field fluctuations about all inherent states sampled at thermal equilibrium. This

field-theoretic Hamiltonian  $\Delta F[\mathbf{u}]$  is suitable for obtaining analytical solutions for the energy barrier corresponding to excitations. The elastic constants emanating from the field theory will be connected to the particle description in Section 1.2.

The first coarse-graining step can be performed by computing  $\mathbf{u}(\mathbf{x})$  from  $\mathbf{u}^\alpha$  by constructing a mesh from the triangulation of inherent-state configurations, as illustrated in Fig. S.2, and choosing an interpolating function  $\hat{N}_\alpha(\mathbf{x})$  such that  $\hat{N}_\alpha(\mathbf{R}^\beta) = \delta_{\alpha\beta}$ . In this case,  $\mathbf{u}(\mathbf{x})$  can be computed as

$$\mathbf{u}(\mathbf{x}) \equiv \sum_{\alpha=1}^N \mathbf{u}^\alpha \hat{N}_\alpha(\mathbf{x}). \quad (16)$$

In this case, the functional measure, defined as  $\mathcal{D}\mathbf{u} \equiv \prod_{\alpha=1}^N d^d \mathbf{u}(\mathbf{R}^\alpha)$ , can be rewritten in terms of  $\mathbf{u}^\alpha$  by applying Eq. (16):

$$\mathcal{D}\mathbf{u} = \prod_{\alpha=1}^N d^d \mathbf{u}^\alpha \quad (17)$$

and thus, no extra Jacobian factor is introduced when changing the integration variables in Eq. (14) from  $\mathbf{u}^\alpha$  to  $\mathbf{u}(\mathbf{x} = \mathbf{R}^\alpha)$ . The second coarse-graining step can be performed by introducing the strain tensor field  $\epsilon \equiv \frac{1}{2} [\nabla \mathbf{u} + (\nabla \mathbf{u})^T]$  into the potential energy  $U(\{\mathbf{r}^\alpha\})$ . To see this, note that  $U(\{\mathbf{r}^\alpha\})$  in Eq. (2) is a function of only the pair distance  $r^{\alpha\beta}$ , which is computable from the corresponding pair distance in inherent state  $R^{\alpha\beta} \equiv |\mathbf{R}^\beta - \mathbf{R}^\alpha|$  and  $\epsilon$ . For small deformations, line segments in the current configuration  $d\mathbf{r}$  can be computed from line segments in the reference configuration  $d\mathbf{R}$  through the following expression

$$d\mathbf{r} \cdot d\mathbf{r} = d\mathbf{R} \cdot (2\epsilon + \mathbf{I}) d\mathbf{R} \quad (18)$$

where  $\mathbf{I}$  is the identity. Integrating Eq. (18) from  $\mathbf{R}^\alpha$  to  $\mathbf{R}^\beta$ , one can compute  $r^{\alpha\beta}$  given a strain tensor field  $\epsilon(\mathbf{x})$ . This was done in [3] by using Eq. (18) as a basis for an arc-length formula

$$r^{\alpha\beta} \approx \int_0^1 \sqrt{\frac{d\mathbf{c}}{ds} \cdot [2\epsilon(\mathbf{c}(s)) + \mathbf{I}] \frac{d\mathbf{c}}{ds}} ds, \quad (19)$$

and choosing the parametrizing curve  $\mathbf{c}(s)$  to be a straight line  $\mathbf{c}(s) = s\mathbf{R}^\beta + (1-s)\mathbf{R}^\alpha$  connecting two particles in the inherent state, so that

$$r^{\alpha\beta} \approx \int_0^1 \sqrt{\mathbf{R}^{\alpha\beta} \cdot [2\epsilon(s\mathbf{R}^\alpha + (1-s)\mathbf{R}^\beta) + \mathbf{I}] \mathbf{R}^{\alpha\beta}} ds \quad (20)$$

where  $\mathbf{R}^{\alpha\beta} = \mathbf{R}^\beta - \mathbf{R}^\alpha$ . Equation (20) formally indicates that the relative difference in potential energy  $\Delta U$  entering Eq. (14) can be computed from two equivalent representations with one being in the particle picture and another as a field picture, i.e.,

$$\Delta U(\{\mathbf{u}^\alpha\}; \{\mathbf{R}^\alpha\}) \longleftrightarrow \Delta \tilde{U}[\epsilon_{ij}; \{\mathbf{R}^\alpha\}]. \quad (21)$$

are two representations with  $\epsilon_{ij} = \frac{1}{2} [u_{i,j} + u_{j,i}]$  the strain tensor in index notation<sup>§</sup>. Alternatively, one may propose that there exists a field-theoretic description at the outset for the potential energy difference in terms of the strain field; in this case, one must connect the field theory with the particle picture to be able to compute quantities from molecular simulations, which is provided in Section 1.2 for the harmonic approximation.

---

<sup>§</sup>Herein, the Greek indices denote particle labels, and roman letters enumerate Cartesian components

Upon choosing the strain tensor representation (the RHS of Eq. (21)), one may arrive at its harmonic approximation through a functional Taylor series expansion of  $\Delta\tilde{U}[\epsilon_{ij}; \{\mathbf{R}^\alpha\}]$  around  $\epsilon_{ij} = 0$  truncated at quadratic order:

$$\Delta\tilde{U}[\epsilon_{ij}; \{\mathbf{R}^\alpha\}] \approx \int d^d\mathbf{x} \frac{\delta\Delta\tilde{U}}{\delta\epsilon_{ij}(\mathbf{x})} \epsilon_{ij}(\mathbf{x}) + \frac{1}{2} \int d^d\mathbf{x} \int d^d\mathbf{x}' \epsilon_{ij}(\mathbf{x}) \frac{\delta^2\Delta\tilde{U}}{\delta\epsilon_{ij}(\mathbf{x})\delta\epsilon_{ij}(\mathbf{x}')} \epsilon_{kl}(\mathbf{x}'). \quad (22)$$

To simplify Eq. (22), note that  $\frac{\delta\Delta\tilde{U}}{\delta\epsilon_{ij}(\mathbf{x})} \equiv T_{ij}^{\text{IS}}(\mathbf{x})$  is the residual stress in the inherent-state configuration and thus, the first-order term becomes

$$\int d^d\mathbf{x} \frac{\delta\Delta\tilde{U}}{\delta\epsilon_{ij}(\mathbf{x})} \epsilon_{ij}(\mathbf{x}) = \int d^d\mathbf{x} T_{ij}^{\text{IS}}(\mathbf{x}) \epsilon_{ij}(\mathbf{x}) = \frac{1}{2} \int d^d\mathbf{x} T_{ij}^{\text{IS}}(\mathbf{x}) [u_{i,j}(\mathbf{x}) + u_{j,i}(\mathbf{x})] \quad (23)$$

and using divergence theorem and integration by parts,

$$\begin{aligned} \int d^d\mathbf{x} \frac{\delta\Delta\tilde{U}}{\delta\epsilon_{ij}(\mathbf{x})} \epsilon_{ij}(\mathbf{x}) &= -\frac{1}{2} \int d^d\mathbf{x} [T_{ij,j}^{\text{IS}}(\mathbf{x}) u_i(\mathbf{x}) + T_{ij,i}^{\text{IS}}(\mathbf{x}) u_j(\mathbf{x})] \\ &\quad + \frac{1}{2} \int dS T_{ij}^{\text{IS}}(\mathbf{x}) [u_i(\mathbf{x}) n_j(\mathbf{x}) + u_j(\mathbf{x}) n_i(\mathbf{x})]. \end{aligned} \quad (24)$$

At mechanical equilibrium, stress is divergence-free ( $T_{ij,j}^{\text{IS}}(\mathbf{x}) = T_{ji,j}^{\text{IS}}(\mathbf{x}) = 0$ ) and suitable boundary conditions also erase the surface integral terms. This implies that the RHS of Eq. (24) vanishes and

$$\int d^d\mathbf{x} \frac{\delta\Delta\tilde{U}}{\delta\epsilon_{ij}(\mathbf{x})} \epsilon_{ij}(\mathbf{x}) = 0, \quad (25)$$

for any inherent state. Using Eq. (25), the quadratic expansion Eq. (22) becomes

$$\Delta\tilde{U}[\epsilon_{ij}; \{\mathbf{R}^\alpha\}] \approx \frac{1}{2} \int d^d\mathbf{x} \int d^d\mathbf{x}' \epsilon_{ij}(\mathbf{x}) \frac{\delta^2\Delta\tilde{U}}{\delta\epsilon_{ij}(\mathbf{x})\delta\epsilon_{ij}(\mathbf{x}')} \epsilon_{kl}(\mathbf{x}'). \quad (26)$$

By definition, the elasticity tensor  $C_{ijkl}(\mathbf{x}, \mathbf{x}') \equiv \frac{\delta^2\Delta\tilde{U}}{\delta\epsilon_{ij}(\mathbf{x})\delta\epsilon_{kl}(\mathbf{x}')}$  is non-local as the expansion also considers interactions at very short length scales  $|\mathbf{x} - \mathbf{x}'| \ll O(\sigma)$ . In what follows, we only account for interactions at length-scales of  $O(\sigma)$  and consider the elasticity tensor to be local, i.e.,

$$C_{ijkl}(\mathbf{x}, \mathbf{x}') \approx C_{ijkl} \delta(\mathbf{x} - \mathbf{x}') \quad (27)$$

where  $C_{ijkl} = \frac{1}{V} \frac{\partial^2 U}{\partial\epsilon_{ij}\partial\epsilon_{kl}}$  are elastic constants of a particular inherent state, whose analytical expressions are provided in Section 1.2. Combining Eq. (26) with Eq. (27), we obtain

$$\Delta\tilde{U}[\epsilon_{ij}; \{\mathbf{R}^\alpha\}] \approx \frac{1}{2} \int d^d\mathbf{x} \epsilon_{ij}(\mathbf{x}) C_{ijkl} \epsilon_{kl}(\mathbf{x}) \quad (28)$$

leading to an elastic strain energy about an inherent state. The energy functional or the effective Hamiltonian entering the field-theoretic partition function in Eq. (15) can be related to the elastic strain energy Eq. (28) as

$$\Delta F[\epsilon_{ij}] \equiv -k_B T \ln \left\langle e^{-\beta \Delta\tilde{U}[\epsilon_{ij}; \{\mathbf{R}^\alpha\}]} \right\rangle_{\text{IS}}. \quad (29)$$

For small strains around  $\epsilon_{ij} = 0$  one may approximate  $\Delta F[\epsilon_{ij}]$  as an averaged elastic strain energy for inherent states sampled at thermal equilibrium, i.e.,

$$\Delta F[\epsilon_{ij}] = -k_B T \ln \left\langle e^{-\frac{\beta}{2} \int d^d\mathbf{x} \epsilon_{ij} C_{ijkl} \epsilon_{kl}} \right\rangle_{\text{IS}} \quad (30)$$

$$= -k_B T \ln \left\langle 1 - \frac{\beta}{2} \int d^d \mathbf{x} \epsilon_{ij} C_{ijkl} \epsilon_{kl} + \dots \right\rangle_{\text{IS}} \quad (31)$$

$$\approx \frac{1}{2} \int d^d \mathbf{x} \epsilon_{ij} C_{ijkl}^{\text{IS}} \epsilon_{kl} \quad (32)$$

where  $C_{ijkl}^{\text{IS}} = \langle C_{ijkl} \rangle_{\text{IS}}$  is the inherent-state ensemble averaged elasticity tensor. Using Eq. (16) and the energy functional in Eq. (32), the partition function  $\bar{Q}_{\text{fin}}$  in Eq. (14) can be transformed into a partition function for a Gaussian field theory of elastic fluctuations

$$\bar{Q}_{\text{fin}} = \int \mathcal{D}\mathbf{u} e^{-\beta \Delta F}; \quad \Delta F[\epsilon_{ij}] = \frac{1}{2} \int d^d \mathbf{x} \epsilon_{ij} C_{ijkl}^{\text{IS}} \epsilon_{kl}. \quad (33)$$

The energy functional  $\Delta F$  in Eq. (33) can be further simplified for isotropic systems. First, note that the linear constitutive law relating the stress and strain fields can be obtained by defining the elastic stress  $\mathbf{T} = T_{ij} \mathbf{e}_i \otimes \mathbf{e}_j$  as

$$T_{mn}(\mathbf{x}) \equiv \frac{\delta \Delta F[\epsilon_{ij}]}{\delta \epsilon_{mn}(\mathbf{x})} = \int d^d \mathbf{x}' \frac{\delta}{\delta \epsilon_{ij}(\mathbf{x})} \left( \frac{1}{2} \epsilon_{ij}(\mathbf{x}') C_{ijkl}^{\text{IS}} \epsilon_{kl}(\mathbf{x}') \right) \quad (34)$$

$$= \int d^d \mathbf{x}' \frac{1}{2} \left( \frac{\delta \epsilon_{ij}(\mathbf{x}')}{\delta \epsilon_{mn}(\mathbf{x})} C_{ijkl}^{\text{IS}} \epsilon_{kl} + \epsilon_{ij} C_{ijkl}^{\text{IS}} \frac{\delta \epsilon_{kl}(\mathbf{x}')}{\delta \epsilon_{mn}(\mathbf{x})} \right) \quad (35)$$

$$= \frac{1}{2} (\delta_{im} \delta_{jn} C_{ijkl}^{\text{IS}} \epsilon_{kl}(\mathbf{x}) + \epsilon_{ij}(\mathbf{x}) C_{ijkl}^{\text{IS}} \delta_{km} \delta_{ln}) \quad (36)$$

$$= C_{mnkl}^{\text{IS}} \epsilon_{kl}(\mathbf{x}) \quad (37)$$

where going from the third to the fourth line, we have made use of the major symmetry,  $C_{ijkl} = C_{klij}$ . Second, the structural disorder in inherent states gives rise to an isotropic solid, whose elasticity tensor is known to be a function of only two elastic constants

$$C_{ijkl}^{\text{IS}} = \lambda^{\text{IS}} \delta_{ij} \delta_{kl} + G^{\text{IS}} (\delta_{ik} \delta_{jl} + \delta_{il} \delta_{jk}) \quad (38)$$

where  $\lambda^{\text{IS}}$  is the first Lamé constant and  $G^{\text{IS}}$  is the shear modulus. Note that the relationship between  $\lambda^{\text{IS}}$  and  $G^{\text{IS}}$  with other elastic constants, e.g., the bulk modulus  $B^{\text{IS}}$  and the Poisson's ratio  $\nu^{\text{IS}}$ , are dimension-dependent. Since all subsequent works will be focused on two-dimensional (2D) polydisperse systems, only the 2D relations are given:

$$B^{\text{IS}} \equiv \lambda^{\text{IS}} + G^{\text{IS}}; \quad \nu^{\text{IS}} \equiv \frac{B^{\text{IS}} - G^{\text{IS}}}{B^{\text{IS}} + G^{\text{IS}}}. \quad (39)$$

Replacing  $\lambda^{\text{IS}}$  with  $B^{\text{IS}}$  in Eq. (38),

$$C_{ijkl}^{\text{IS}} = B^{\text{IS}} \delta_{ij} \delta_{kl} + G^{\text{IS}} (\delta_{ik} \delta_{jl} + \delta_{il} \delta_{jk} - \delta_{ij} \delta_{kl}) \quad (40)$$

and the constitutive law Eq. (37) becomes

$$T_{ij} = B^{\text{IS}} \epsilon_{kk} \delta_{ij} + 2G^{\text{IS}} \left( \epsilon_{ij} - \frac{1}{2} \epsilon_{kk} \delta_{ij} \right). \quad (41)$$

Substituting Eq. (41) into the elastic strain energy in Eq. (33) yields

$$\Delta F[\epsilon_{ij}] = \frac{1}{2} \int d^2 \mathbf{x} \epsilon_{ij} \left[ B^{\text{IS}} \epsilon_{kk} \delta_{ij} + 2G^{\text{IS}} \left( \epsilon_{ij} - \frac{1}{2} \epsilon_{kk} \delta_{ij} \right) \right] \quad (42)$$

$$= \frac{1}{2} \int d^2\mathbf{x} \left[ B^{\text{IS}} \epsilon_{kk}^2 + 2G^{\text{IS}} \left( \epsilon_{ij} \epsilon_{ij} - \frac{1}{2} \epsilon_{kk}^2 \right) \right]. \quad (43)$$

Equation (43) can also be rewritten as a function of stress. This will be an advantageous formulation when computing the excitation energy barrier  $J_\sigma$  in Section 2. To this end, let us write the constitutive law in vector notation

$$\begin{bmatrix} T_{xx} \\ T_{yy} \\ T_{xy} \end{bmatrix} = \begin{bmatrix} B^{\text{IS}} + G^{\text{IS}} & B^{\text{IS}} - G^{\text{IS}} & 0 \\ B^{\text{IS}} - G^{\text{IS}} & B^{\text{IS}} + G^{\text{IS}} & 0 \\ 0 & 0 & 2G^{\text{IS}} \end{bmatrix} \begin{bmatrix} \epsilon_{xx} \\ \epsilon_{yy} \\ \epsilon_{xy} \end{bmatrix}. \quad (44)$$

Taking the inverse of the elastic constant matrix, we obtain

$$\begin{bmatrix} \epsilon_{xx} \\ \epsilon_{yy} \\ \epsilon_{xy} \end{bmatrix} = \begin{bmatrix} \frac{1}{4} \left( \frac{1}{B^{\text{IS}}} + \frac{1}{G^{\text{IS}}} \right) & \frac{1}{4} \left( \frac{1}{B^{\text{IS}}} - \frac{1}{G^{\text{IS}}} \right) & 0 \\ \frac{1}{4} \left( \frac{1}{B^{\text{IS}}} - \frac{1}{G^{\text{IS}}} \right) & \frac{1}{4} \left( \frac{1}{B^{\text{IS}}} + \frac{1}{G^{\text{IS}}} \right) & 0 \\ 0 & 0 & \frac{1}{2G^{\text{IS}}} \end{bmatrix} \begin{bmatrix} T_{xx} \\ T_{yy} \\ T_{xy} \end{bmatrix}. \quad (45)$$

Upon diagonalizing the matrix, we also obtain

$$\begin{bmatrix} \epsilon_{xx} \\ \epsilon_{yy} \\ \epsilon_{xy} \end{bmatrix} = \underbrace{\begin{bmatrix} 1 & 1 & 0 \\ -1 & 1 & 0 \\ 0 & 0 & 1 \end{bmatrix}^{-1}}_{\mathbf{P}^{-1}} \underbrace{\begin{bmatrix} \frac{1}{2B^{\text{IS}}} & 0 & 0 \\ 0 & \frac{1}{2G^{\text{IS}}} & 0 \\ 0 & 0 & \frac{1}{2G^{\text{IS}}} \end{bmatrix}}_{\mathbf{\Lambda}} \underbrace{\begin{bmatrix} 1 & 1 & 0 \\ -1 & 1 & 0 \\ 0 & 0 & 1 \end{bmatrix}}_{\mathbf{P}} \begin{bmatrix} T_{xx} \\ T_{yy} \\ T_{xy} \end{bmatrix} \quad (46)$$

$$= \begin{bmatrix} 1 & 1 & 0 \\ -1 & 1 & 0 \\ 0 & 0 & 1 \end{bmatrix}^{-1} \begin{bmatrix} \frac{1}{2B^{\text{IS}}} & 0 & 0 \\ 0 & \frac{1}{2G^{\text{IS}}} & 0 \\ 0 & 0 & \frac{1}{2G^{\text{IS}}} \end{bmatrix} \begin{bmatrix} T_{xx} + T_{yy} \\ T_{yy} - T_{xx} \\ T_{xy} \end{bmatrix} \quad (47)$$

where  $\mathbf{\Lambda}$  is the eigenvalue matrix and  $\mathbf{P}$  is the column-eigenvector matrix. Multiplying with  $\mathbf{P}$  on both sides of Eq. (47) eliminates the  $\mathbf{P}^{-1}$  matrix yielding

$$\begin{bmatrix} \epsilon_{xx} + \epsilon_{yy} \\ \epsilon_{yy} - \epsilon_{xx} \\ \epsilon_{xy} \end{bmatrix} = \begin{bmatrix} \frac{1}{B^{\text{IS}}} & 0 & 0 \\ 0 & \frac{1}{G^{\text{IS}}} & 0 \\ 0 & 0 & \frac{1}{2G^{\text{IS}}} \end{bmatrix} \begin{bmatrix} \frac{T_{xx} + T_{yy}}{2} \\ \frac{T_{yy} - T_{xx}}{2} \\ T_{xy} \end{bmatrix}. \quad (48)$$

Note that  $\epsilon_{xx} + \epsilon_{yy} \equiv \epsilon_{kk}$  in index notation and hence

$$\epsilon_{ij} \epsilon_{ij} - \frac{1}{2} \epsilon_{kk}^2 = \epsilon_{xx} \epsilon_{xx} + \epsilon_{yy} \epsilon_{yy} + 2\epsilon_{xy} \epsilon_{xy} - \frac{1}{2} (\epsilon_{xx}^2 + \epsilon_{yy}^2 + 2\epsilon_{xx} \epsilon_{yy}) \quad (49)$$

$$= \frac{1}{2} (\epsilon_{xx} \epsilon_{xx} + \epsilon_{yy} \epsilon_{yy} - 2\epsilon_{xx} \epsilon_{yy}) + 2\epsilon_{xy} \epsilon_{xy} \quad (50)$$

$$= \frac{1}{2} (\epsilon_{xx} - \epsilon_{yy})^2 + 2\epsilon_{xy}^2, \quad (51)$$

which means that the elastic strain energy can also be rewritten as

$$\Delta F[\epsilon_{xx}, \epsilon_{yy}, \epsilon_{xy}] = \frac{1}{2} \int d^2\mathbf{x} \left[ B^{\text{IS}} (\epsilon_{xx} + \epsilon_{yy})^2 + 2G^{\text{IS}} \left( \frac{1}{2} (\epsilon_{xx} - \epsilon_{yy})^2 + 2\epsilon_{xy}^2 \right) \right]. \quad (52)$$

Defining the principal components of stress as  $T_1 = -\frac{1}{2} [T_{xx} + T_{yy}]$ ,  $T_2 = \frac{1}{2} [T_{yy} - T_{xx}]$ , and  $T_3 = T_{xy}$  and using Eqs. (48) and (52), we obtain a quadratic expression for the elastic strain energy in terms of stresses:

$$\Delta F = \frac{1}{2} \int d^2\mathbf{x} \left( \frac{1}{B^{\text{IS}}} \left( \frac{T_{xx} + T_{yy}}{2} \right)^2 + \frac{1}{G^{\text{IS}}} \left[ \left( \frac{T_{yy} - T_{xx}}{2} \right)^2 + T_{xy}^2 \right] \right) \quad (53)$$

$$= \int d^2\mathbf{x} \left( \frac{1}{2B^{\text{IS}}} (T_1)^2 + \frac{1}{2G^{\text{IS}}} [(T_2)^2 + (T_3)^2] \right). \quad (54)$$

## 1.2 Deriving the Elasticity Tensor $C_{ijkl}$

The elasticity tensor  $C_{ijkl}$  entering the Gaussian field theory can be computed from partial derivatives of the potential energy  $U$  given in Eq. (2) with respect to a constant strain  $\epsilon_{ij}$  applied to a given inherent state  $R_i^\alpha$ . This derivation of  $C_{ijkl}$  is inspired from and closely follows [4] with few inputs from [5]. Primarily, we would like the elastic constants to model elastic response of a molecular system at mechanical equilibrium, when subjected to strain. To this end, let  $R_i^\alpha$  be the reference configuration. Suppose that the system is subjected to an affine transformation (or a deformation gradient)  $A_{ij}$ , which is related to the strain tensor as  $\epsilon_{ij} = \frac{1}{2} (A_{ik}^T A_{kj} - \delta_{ij})$  [4]. Given this deformation, the system elastically responds by attaining a final configuration  $r_i^\alpha$  that is also at mechanical equilibrium, i.e.,

$$\mathbf{F}^\alpha(\{\mathbf{r}^\alpha\}) = 0, \text{ for non-zero strain.} \quad (55)$$

One may decompose  $r_i^\alpha$  into two parts:

$$r_i^\alpha = A_{ij} R_j^\alpha + X_i^\alpha \quad (56)$$

where the first term is the affine motion and  $X_i^\alpha$  is the non-affine displacement that must be solved self-consistently from Eq. (55). Note that  $R_i^\alpha$  is fixed while  $\epsilon_{ij}$  (through  $A_{ij}$ ) is given. As a result of Eq. (55) and Eq. (56),  $X_i^\alpha$  implicitly depends on  $\epsilon_{ij}$ .

To obtain the elastic constants in terms of the potential, let us begin with the total differential of  $U(\{\mathbf{r}^\alpha\})$  with respect to both  $\epsilon_{ij}$  and  $X_i^\alpha$  given Eq. (56):

$$dU = \left. \frac{\partial U}{\partial \epsilon_{ij}} \right|_{\mathbf{X}^\alpha} d\epsilon_{ij} + \left. \frac{\partial U}{\partial X_l^\beta} \right|_{\epsilon_{ij}} dX_l^\beta. \quad (57)$$

Studying variations of  $U$  subjected to the constraint  $\mathbf{F}^\alpha = 0$  in Eq. (55), then by multivariable calculus we obtain

$$\frac{\partial U}{\partial \epsilon_{ij}} = \left. \frac{\partial U}{\partial \epsilon_{ij}} \right|_{\mathbf{X}^\alpha} + \left. \frac{\partial U}{\partial X_l^\beta} \right|_{\epsilon_{ij}} \frac{\partial X_l^\beta}{\partial \epsilon_{ij}} \quad (58)$$

where  $\frac{\partial X_l^\beta}{\partial \epsilon_{ij}}$  is non-zero as  $X_i^\alpha$  depends on  $\epsilon_{ij}$  through Eq. (55). We denote the partial derivative  $\frac{\partial}{\partial \epsilon_{ij}}$  such that  $\mathbf{F}^\alpha = 0$  as  $\left. \frac{\partial}{\partial \epsilon_{ij}} \right|_{\mathbf{F}^\alpha}$  to rewrite the relation as

$$\left. \frac{\partial U}{\partial \epsilon_{ij}} \right|_{\mathbf{F}^\alpha} = \left. \frac{\partial U}{\partial \epsilon_{ij}} \right|_{\mathbf{X}^\alpha} + \left. \frac{\partial U}{\partial X_l^\beta} \right|_{\epsilon_{ij}} \left. \frac{\partial X_l^\beta}{\partial \epsilon_{ij}} \right|_{\mathbf{F}^\alpha}. \quad (59)$$

The change in potential energy due to elastic response at mechanical equilibrium can be written as

$$U(\{\mathbf{r}^\alpha\}) - U(\{\mathbf{R}^\alpha\}) \approx \left. \frac{\partial U}{\partial \epsilon_{ij}} \right|_{\mathbf{F}^\alpha} \epsilon_{ij} + \epsilon_{ij} \left. \frac{\partial}{\partial \epsilon_{ij}} \right|_{\mathbf{F}^\alpha} \left( \left. \frac{\partial U}{\partial \epsilon_{kl}} \right|_{\mathbf{F}^\alpha} \right) \epsilon_{kl} \quad (60)$$

where the partial derivatives are evaluated at  $\epsilon_{ij} = 0$ . We denote the 2nd order derivative as

$$\left. \frac{\partial}{\partial \epsilon_{ij}} \right|_{\mathbf{F}^\alpha} \left( \left. \frac{\partial U}{\partial \epsilon_{kl}} \right|_{\mathbf{F}^\alpha} \right) = \left. \frac{\partial^2 U}{\partial \epsilon_{ij} \partial \epsilon_{kl}} \right|_{\mathbf{F}^\alpha} \quad (61)$$

and define the elastic constants as

$$C_{ijkl} = \frac{1}{V} \frac{\partial^2 U}{\partial \epsilon_{ij} \partial \epsilon_{kl}} \Big|_{\mathbf{F}^\alpha} \text{ at } \epsilon_{ij} = 0. \quad (62)$$

Note that  $X_l^\beta$  can't be solved explicitly from Eq. (55), but its derivative  $\frac{\partial X_l^\beta}{\partial \epsilon_{ij}} \Big|_{\mathbf{F}^\alpha}$  can be evaluated via the following equation:

$$\frac{\partial F_k^\alpha}{\partial \epsilon_{ij}} \Big|_{\mathbf{F}^\alpha} = 0 = \frac{\partial F_k^\alpha}{\partial \epsilon_{ij}} \Big|_{\mathbf{X}^\alpha} + \frac{\partial F_k^\alpha}{\partial X_l^\beta} \Big|_{\epsilon_{ij}} \frac{\partial X_l^\beta}{\partial \epsilon_{ij}} \Big|_{\mathbf{F}^\alpha} \quad (63)$$

obtained by differentiating Eq. (55). Let us define a new variable  $\Xi_{ijk}^\alpha$  as

$$\Xi_{ijk}^\alpha = - \frac{\partial F_k^\alpha}{\partial \epsilon_{ij}} \Big|_{\mathbf{X}^\alpha}, \quad (64)$$

which allows us to rewrite Eq. (63) as

$$0 = -\Xi_{ijk}^\alpha + \frac{\partial F_k^\alpha}{\partial X_l^\beta} \Big|_{\epsilon_{ij}} \frac{\partial X_l^\beta}{\partial \epsilon_{ij}} \Big|_{\mathbf{F}^\alpha}. \quad (65)$$

To simplify the factor  $\frac{\partial F_k^\alpha}{\partial X_l^\beta} \Big|_{\epsilon_{ij}}$  in Eq. (65), note from the formula for final configuration  $r_i^\alpha$  in Eq. (56) that

$$\frac{\partial r_i^\alpha}{\partial X_j^\beta} \Big|_{\epsilon_{ij}} = \frac{\partial X_i^\alpha}{\partial X_j^\beta} \Big|_{\epsilon_{ij}} = \delta_{ij} \delta^{\alpha\beta}, \quad (66)$$

which implies that

$$\frac{\partial F_k^\alpha}{\partial X_l^\beta} \Big|_{\epsilon_{ij}} = \frac{\partial F_k^\alpha}{\partial r_m^\gamma} \frac{\partial r_m^\gamma}{\partial X_l^\beta} \Big|_{\epsilon_{ij}} = \frac{\partial F_k^\alpha}{\partial r_m^\gamma} \delta_{ml} \delta^{\gamma\beta} = \frac{\partial F_k^\alpha}{\partial r_l^\beta} = - \frac{\partial^2 U}{\partial r_l^\beta \partial r_k^\alpha}. \quad (67)$$

The last equality is the negative of the Hessian  $\mathbf{H}$ , evaluated at  $r_i^\alpha = H_{ij} R_j^\alpha + X_i^\alpha$ , where the Hessian is defined by

$$H_{lk}^{\beta\alpha} = \frac{\partial^2 U(\{\mathbf{r}^\alpha\})}{\partial r_l^\beta \partial r_k^\alpha}. \quad (68)$$

Using these simplifications, we can rewrite Eq. (65) as

$$0 = -\Xi_{ijk}^\alpha - H_{lk}^{\beta\alpha} \frac{\partial X_l^\beta}{\partial \epsilon_{ij}} \Big|_{\mathbf{F}^\alpha} = \Xi_{ijk}^\alpha + H_{kl}^{\alpha\beta} \frac{\partial X_l^\beta}{\partial \epsilon_{ij}} \Big|_{\mathbf{F}^\alpha} \quad (69)$$

where use is made of the symmetry of the Hessian in the second equality, i.e.,  $H_{lk}^{\beta\alpha} = H_{kl}^{\alpha\beta}$ . Let the pseudo-inverse of the Hessian be  $\mathbf{H}^+$  or  $(H_{kl}^{\alpha\beta})^+$  in indicial notation. It has the property  $\mathbf{H}\mathbf{H}^+\mathbf{H} = \mathbf{H}$ , or in indicial notation

$$H_{mn}^{\mu\nu} (H_{nk}^{\nu\alpha})^+ H_{kl}^{\alpha\beta} = H_{ml}^{\mu\beta}. \quad (70)$$

Multiplying  $H_{mn}^{\mu\nu}(H_{nk}^{\nu\alpha})^+$  to Eq. (69) gives

$$0 = H_{mn}^{\mu\nu}(H_{nk}^{\nu\alpha})^+ \Xi_{ijk}^\alpha + H_{mn}^{\mu\nu}(H_{nk}^{\nu\alpha})^+ H_{kl}^{\alpha\beta} \frac{\partial X_l^\beta}{\partial \epsilon_{ij}} \Big|_{\mathbf{F}^\alpha} \quad (71)$$

$$= H_{mn}^{\mu\nu}(H_{nk}^{\nu\alpha})^+ \Xi_{ijk}^\alpha + H_{ml}^{\mu\beta} \frac{\partial X_l^\beta}{\partial \epsilon_{ij}} \Big|_{\mathbf{F}^\alpha} \quad (72)$$

$$= H_{ml}^{\mu\beta} \left[ (H_{lk}^{\beta\alpha})^+ \Xi_{ijk}^\alpha + \frac{\partial X_l^\beta}{\partial \epsilon_{ij}} \Big|_{\mathbf{F}^\alpha} \right] \quad (73)$$

where use is made of Eq. (70) in the second equality, and dummy indices in the first term are switched from  $\nu \rightarrow \beta$  and  $n \rightarrow l$  to obtain the third equality. Since the Hessian is non-zero, Eq. (73) dictates

$$\frac{\partial X_l^\beta}{\partial \epsilon_{ij}} \Big|_{\mathbf{F}^\alpha} = -(H_{lk}^{\beta\alpha})^+ \Xi_{ijk}^\alpha = -\Xi_{ijk}^\alpha (H_{kl}^{\alpha\beta})^+ \quad (74)$$

using the symmetry of the pseudo-inverse of the Hessian, thereby evaluating the derivative of  $X_l^\beta$  with respect to strain  $\epsilon_{ij}$ .

Using Eq. (74), the strain derivatives of the potential energy in Eq. (59) can now be written as

$$\frac{\partial U}{\partial \epsilon_{ij}} \Big|_{\mathbf{F}^\alpha} = \frac{\partial U}{\partial \epsilon_{ij}} \Big|_{\mathbf{X}^\alpha} - \Xi_{ijk}^\alpha (H_{kl}^{\alpha\beta})^+ \frac{\partial U}{\partial X_l^\beta} \Big|_{\epsilon_{ij}}. \quad (75)$$

Note that Eq. (75) is true for any function  $h(\epsilon_{ij}, X_i^\alpha)$ . We can further simplify the second term in Eq. (75) using Eq. (66):

$$\frac{\partial U}{\partial X_l^\beta} \Big|_{\epsilon_{ij}} = \frac{\partial U}{\partial r_m^\gamma} \frac{\partial r_m^\gamma}{\partial X_l^\beta} \Big|_{\epsilon_{ij}} = \frac{\partial U}{\partial r_m^\gamma} \delta_{ml} \delta^{\gamma\beta} = \frac{\partial U}{\partial r_l^\beta}. \quad (76)$$

Note that  $\frac{\partial U}{\partial r_l^\beta} = -F_l^\beta$  is the force evaluated at the final configuration, and is zero for any non-zero strain according to Eq. (55). This implies that Eq. (75) reduces to

$$\frac{\partial U}{\partial \epsilon_{ij}} \Big|_{\mathbf{F}^\alpha} = \frac{\partial U}{\partial \epsilon_{ij}} \Big|_{\mathbf{X}^\alpha} - \Xi_{ijk}^\alpha (H_{kl}^{\alpha\beta})^+ \frac{\partial U}{\partial r_l^\beta} = \frac{\partial U}{\partial \epsilon_{ij}} \Big|_{\mathbf{X}^\alpha}. \quad (77)$$

Next, we move towards computing the 2nd order derivative:

$$\frac{\partial^2 U}{\partial \epsilon_{ij} \partial \epsilon_{kl}} \Big|_{\mathbf{F}^\alpha} = \frac{\partial}{\partial \epsilon_{ij}} \Big|_{\mathbf{F}^\alpha} \left( \frac{\partial U}{\partial \epsilon_{kl}} \Big|_{\mathbf{X}^\alpha} \right) = \frac{\partial^2 U}{\partial \epsilon_{ij} \partial \epsilon_{kl}} \Big|_{\mathbf{X}^\alpha} - \Xi_{ijm}^\alpha (H_{mn}^{\alpha\beta})^+ \frac{\partial}{\partial X_n^\beta} \Big|_{\epsilon_{ij}} \left( \frac{\partial U}{\partial \epsilon_{kl}} \Big|_{\mathbf{X}^\alpha} \right) \quad (78)$$

using Eq. (75) as an identity for any function  $h(\epsilon_{ij}, X_i^\alpha)$ . The mixed partial derivatives in the second term of last equality in Eq. (78) can be exchanged, i.e.,

$$\frac{\partial}{\partial X_n^\beta} \Big|_{\epsilon_{ij}} \left( \frac{\partial U}{\partial \epsilon_{kl}} \Big|_{\mathbf{X}^\alpha} \right) = \frac{\partial}{\partial \epsilon_{kl}} \Big|_{\mathbf{X}^\alpha} \left( \frac{\partial U}{\partial X_n^\beta} \Big|_{\epsilon_{ij}} \right), \quad (79)$$

which can be further simplified using Eq. (66) as

$$\frac{\partial}{\partial \epsilon_{kl}} \Big|_{\mathbf{X}^\alpha} \left( \frac{\partial U}{\partial X_n^\beta} \Big|_{\epsilon_{ij}} \right) = \frac{\partial}{\partial \epsilon_{kl}} \Big|_{\mathbf{X}^\alpha} \left( \frac{\partial U}{\partial r_m^\alpha} \frac{\partial r_m^\alpha}{\partial X_n^\beta} \Big|_{\epsilon_{ij}} \right) \quad (80)$$

$$= \frac{\partial}{\partial \epsilon_{kl}} \Big|_{\mathbf{X}^\alpha} \left( \frac{\partial U}{\partial r_m^\alpha} \delta_{mn} \delta^{\alpha\beta} \right) \quad (81)$$

$$= \frac{\partial}{\partial \epsilon_{kl}} \Big|_{\mathbf{X}^\alpha} \left( \frac{\partial U}{\partial r_n^\beta} \right) \quad (82)$$

$$= - \frac{\partial}{\partial \epsilon_{kl}} \Big|_{\mathbf{X}^\alpha} \left( F_n^\beta \right) = \Xi_{kl n}^\beta \quad (83)$$

where use is made of the definition for  $\Xi_{kl n}^\beta$  (Eq. (64)). Using this result, we can write the 2nd order derivative in Eq. (78) as

$$\frac{\partial^2 U}{\partial \epsilon_{ij} \partial \epsilon_{kl}} \Big|_{\mathbf{F}^\alpha} = \frac{\partial^2 U}{\partial \epsilon_{ij} \partial \epsilon_{kl}} \Big|_{\mathbf{X}^\alpha} - \Xi_{ij m}^\alpha (H_{mn}^{\alpha\beta})^+ \Xi_{kl n}^\beta; \quad (84)$$

when evaluated at  $\epsilon_{ij} = 0$ , the first term on the right-hand side corresponds to the Born or affine contribution to the elasticity tensor, and the second corresponds to non-affine contributions.

In what follows, we now derive expressions for  $\frac{\partial^2 U}{\partial \epsilon_{ij} \partial \epsilon_{kl}} \Big|_{\mathbf{X}^\alpha}$ ,  $\Xi_{ij m}^\alpha$ , and  $H_{mn}^{\alpha\beta}$  in terms of the reference or inherent state configurations when evaluated at the strain of zero. Note that a zero strain implies that the non-affine displacement  $\mathbf{X}^\alpha$  is also zero. We limit our derivations to potential energies in Eq. (2) of the form of a sum of pair potentials. This is relevant when testing our theory on a variety of 2D polydisperse systems. To this end, from Eq. (56), we can compute the pair-wise distance from  $r_i^{\alpha\beta}$  in terms of  $A_{ij}$  and  $X_i^\alpha$  as

$$r_i^{\alpha\beta} := r_i^\beta - r_i^\alpha = A_{ij} R_j^{\alpha\beta} + X_i^{\alpha\beta} \quad (85)$$

where  $R_j^{\alpha\beta} = R_j^\beta - R_j^\alpha$  and  $X_i^{\alpha\beta} = X_i^\beta - X_i^\alpha$ . Also, the pair distance  $r^{\alpha\beta} = \|\mathbf{r}^\alpha - \mathbf{r}^\beta\|$  is given by

$$r^{\alpha\beta} = \sqrt{R_i^{\alpha\beta} (2\epsilon_{ij} + \delta_{ij}) R_j^{\alpha\beta} + 2X_i^{\alpha\beta} A_{ij} R_j^{\alpha\beta} + X_i^{\alpha\beta} X_i^{\alpha\beta}}. \quad (86)$$

We begin by evaluating the Born or affine contributions in Eq. (84) by taking a strain derivative of the potential energy  $U$  of the form in Eq. (2) at constant  $\mathbf{X}^\alpha$ :

$$\frac{\partial U}{\partial \epsilon_{ij}} \Big|_{\mathbf{X}^\alpha} = \frac{\partial}{\partial \epsilon_{ij}} \Big|_{\mathbf{X}^\alpha} \left( \sum_{\alpha, \beta} \phi(r^{\alpha\beta}) \right) = \sum_{\alpha, \beta} \phi_r(r^{\alpha\beta}) \frac{\partial r^{\alpha\beta}}{\partial \epsilon_{ij}} \Big|_{\mathbf{X}^\alpha} \quad (87)$$

where  $\phi_r(r^{\alpha\beta}) = \frac{d\phi(r=r^{\alpha\beta})}{dr}$ . The remaining partial derivative can be computed from Eq. (86) as

$$\frac{\partial r^{\alpha\beta}}{\partial \epsilon_{ij}} \Big|_{\mathbf{X}^\alpha} = \frac{1}{2r^{\alpha\beta}} \frac{\partial}{\partial \epsilon_{ij}} \Big|_{\mathbf{X}^\alpha} \left( R_k^{\alpha\beta} (2\epsilon_{kl} + \delta_{kl}) R_l^{\alpha\beta} + 2X_k^{\alpha\beta} A_{kl} R_l^{\alpha\beta} + X_k^{\alpha\beta} X_l^{\alpha\beta} \right) \quad (88)$$

$$= \frac{1}{r^{\alpha\beta}} \left( R_i^{\alpha\beta} R_j^{\alpha\beta} + X_k^{\alpha\beta} R_l^{\alpha\beta} \frac{\partial A_{kl}}{\partial \epsilon_{ij}} \Big|_{\mathbf{X}^\alpha} \right). \quad (89)$$

Substituting Eq. (89) into Eq. (87) yields

$$\frac{\partial U}{\partial \epsilon_{ij}} \Big|_{\mathbf{X}^\alpha} = \sum_{\alpha, \beta} \frac{\phi_r(r^{\alpha\beta})}{r^{\alpha\beta}} \left( R_i^{\alpha\beta} R_j^{\alpha\beta} + X_k^{\alpha\beta} R_l^{\alpha\beta} \frac{\partial A_{kl}}{\partial \epsilon_{ij}} \Big|_{\mathbf{X}^\alpha} \right). \quad (90)$$

Using Eq. (90), we compute the 2nd order derivative at constant  $\mathbf{X}^\alpha$

$$\left. \frac{\partial^2 U}{\partial \epsilon_{ij} \partial \epsilon_{kl}} \right|_{\mathbf{X}^\alpha} = \left. \frac{\partial}{\partial \epsilon_{ij}} \right|_{\mathbf{X}^\alpha} \left[ \sum_{\alpha, \beta} \frac{\phi_r(r^{\alpha\beta})}{r^{\alpha\beta}} \left( R_k^{\alpha\beta} R_l^{\alpha\beta} + X_m^{\alpha\beta} R_n^{\alpha\beta} \frac{\partial A_{mn}}{\partial \epsilon_{kl}} \right) \right] \quad (91)$$

$$= \sum_{\alpha, \beta} \left( R_k^{\alpha\beta} R_l^{\alpha\beta} + X_m^{\alpha\beta} R_n^{\alpha\beta} \frac{\partial A_{mn}}{\partial \epsilon_{kl}} \right) \left. \frac{\partial}{\partial \epsilon_{ij}} \right|_{\mathbf{X}^\alpha} \left( \frac{\phi_r(r^{\alpha\beta})}{r^{\alpha\beta}} \right) + \sum_{\alpha, \beta} \frac{\phi_r(r^{\alpha\beta})}{r^{\alpha\beta}} \left( X_m^{\alpha\beta} R_n^{\alpha\beta} \frac{\partial^2 A_{mn}}{\partial \epsilon_{ij} \partial \epsilon_{kl}} \right) \quad (92)$$

$$= \sum_{\alpha, \beta} \left( R_k^{\alpha\beta} R_l^{\alpha\beta} + X_m^{\alpha\beta} R_n^{\alpha\beta} \frac{\partial A_{mn}}{\partial \epsilon_{kl}} \right) \left( \frac{\phi_{rr}(r^{\alpha\beta})}{r^{\alpha\beta}} - \frac{\phi_r(r^{\alpha\beta})}{(r^{\alpha\beta})^2} \right) \left. \frac{\partial r^{\alpha\beta}}{\partial \epsilon_{ij}} \right|_{\mathbf{X}^\alpha} + \sum_{\alpha, \beta} \frac{\phi_r(r^{\alpha\beta})}{r^{\alpha\beta}} \left( X_m^{\alpha\beta} R_n^{\alpha\beta} \frac{\partial^2 A_{mn}}{\partial \epsilon_{ij} \partial \epsilon_{kl}} \right) \quad (93)$$

where the factor  $\left. \frac{\partial r^{\alpha\beta}}{\partial \epsilon_{ij}} \right|_{\mathbf{X}^\alpha}$  can be evaluated from Eq. (89). As mentioned before, we need to evaluate the derivatives as the strain goes to zero. Noting that any term proportional to  $X_m^{\alpha\beta}$  vanishes when  $\epsilon_{ij} = 0$ , Eq. (93) reduces to

$$\left. \frac{\partial^2 U}{\partial \epsilon_{ij} \partial \epsilon_{kl}} \right|_{\mathbf{X}^\alpha} = \sum_{\alpha, \beta} \left( \phi_{rr}(R^{\alpha\beta}) R^{\alpha\beta} - \phi_r(R^{\alpha\beta}) \right) \frac{R_i^{\alpha\beta} R_j^{\alpha\beta} R_k^{\alpha\beta} R_l^{\alpha\beta}}{(R^{\alpha\beta})^3} \quad (94)$$

where  $\phi_r$  and  $\phi_{rr}$  are evaluated at  $R^{\alpha\beta}$ , thus yielding the Born or affine contributions to the elasticity tensor in terms of just the inherent state configurations.

We now evaluate the non-affine contributions in Eq. (84). Given the definition  $\Xi_{ijk}^\gamma = -\left. \frac{\partial F_k^\gamma}{\partial \epsilon_{ij}} \right|_{\mathbf{X}^\alpha}$ , and Eqs. (79) to (83) and Eq. (90), we have

$$\Xi_{ijk}^\gamma = \left. \frac{\partial}{\partial X_k^\gamma} \right|_{\epsilon_{ij}} \left( \left. \frac{\partial U}{\partial \epsilon_{ij}} \right|_{\mathbf{X}^\alpha} \right) \quad (95)$$

$$= \left. \frac{\partial}{\partial X_k^\gamma} \right|_{\epsilon_{ij}} \left[ \sum_{\alpha, \beta} \frac{\phi_r(r^{\alpha\beta})}{r^{\alpha\beta}} \left( R_i^{\alpha\beta} R_j^{\alpha\beta} + X_k^{\alpha\beta} R_l^{\alpha\beta} \frac{\partial A_{kl}}{\partial \epsilon_{ij}} \right) \right] \quad (96)$$

$$= \sum_{\alpha, \beta} \left( R_i^{\alpha\beta} R_j^{\alpha\beta} + X_m^{\alpha\beta} R_n^{\alpha\beta} \frac{\partial A_{mn}}{\partial \epsilon_{ij}} \right) \left. \frac{\partial}{\partial X_k^\gamma} \right|_{\epsilon_{ij}} \left( \frac{\phi_r(r^{\alpha\beta})}{r^{\alpha\beta}} \right) + \sum_{\alpha, \beta} \frac{\phi_r(r^{\alpha\beta})}{r^{\alpha\beta}} \left( \left. \frac{\partial X_m^{\alpha\beta}}{\partial X_k^\gamma} \right|_{\epsilon_{ij}} R_n^{\alpha\beta} \frac{\partial A_{mn}}{\partial \epsilon_{ij}} \right) \quad (97)$$

The second term of last equality can be simplified by noting that

$$\left. \frac{\partial X_m^{\alpha\beta}}{\partial X_k^\gamma} \right|_{\epsilon_{ij}} = \left. \frac{\partial (X_m^\beta - X_m^\alpha)}{\partial X_k^\gamma} \right|_{\epsilon_{ij}} = \delta_{mk} (\delta^{\beta\gamma} - \delta^{\alpha\gamma}) \quad (98)$$

and thus,

$$\sum_{\alpha, \beta} \frac{\phi_r(r^{\alpha\beta})}{r^{\alpha\beta}} \left( \left. \frac{\partial X_m^{\alpha\beta}}{\partial X_k^\gamma} \right|_{\epsilon_{ij}} R_n^{\alpha\beta} \frac{\partial A_{mn}}{\partial \epsilon_{ij}} \right) = \sum_{\alpha, \beta} \frac{\phi_r(r^{\alpha\beta})}{r^{\alpha\beta}} \left( (\delta^{\beta\gamma} - \delta^{\alpha\gamma}) R_n^{\alpha\beta} \frac{\partial A_{kn}}{\partial \epsilon_{ij}} \right) \quad (99)$$

$$= \sum_{\alpha \neq \gamma} \frac{\phi_r(r^{\alpha\gamma})}{r^{\alpha\gamma}} R_n^{\alpha\gamma} \left( \frac{\partial A_{kn}}{\partial \epsilon_{ij}} \Big|_{\mathbf{X}^\alpha} \right). \quad (100)$$

Substituting Eq. (100) into Eq. (97), we obtain

$$\begin{aligned} \Xi_{ijk}^\gamma &= \sum_{\alpha, \beta} \left( R_i^{\alpha\beta} R_j^{\alpha\beta} + X_m^{\alpha\beta} R_n^{\alpha\beta} \frac{\partial A_{mn}}{\partial \epsilon_{ij}} \Big|_{\mathbf{X}^\alpha} \right) \frac{\partial}{\partial X_k^\gamma} \Big|_{\epsilon_{ij}} \left( \frac{\phi_r(r^{\alpha\beta})}{r^{\alpha\beta}} \right) \\ &\quad + \sum_{\alpha \neq \gamma} \frac{\phi_r(r^{\alpha\gamma})}{r^{\alpha\gamma}} R_n^{\alpha\gamma} \left( \frac{\partial A_{kn}}{\partial \epsilon_{ij}} \Big|_{\mathbf{X}^\alpha} \right) \end{aligned} \quad (101)$$

To simplify the first term, note that

$$\frac{\partial}{\partial X_k^\gamma} \Big|_{\epsilon_{ij}} \left( \frac{\phi_r(r^{\alpha\beta})}{r^{\alpha\beta}} \right) = \left( \frac{\phi_{rr}(r^{\alpha\beta})}{r^{\alpha\beta}} - \frac{\phi_r(r^{\alpha\beta})}{(r^{\alpha\beta})^2} \right) \frac{\partial r^{\alpha\beta}}{\partial X_k^\gamma} \Big|_{\epsilon_{ij}} \quad (102)$$

$$= \left( \frac{\phi_{rr}(r^{\alpha\beta})}{r^{\alpha\beta}} - \frac{\phi_r(r^{\alpha\beta})}{(r^{\alpha\beta})^2} \right) \frac{\partial r^{\alpha\beta}}{\partial r_l^{\alpha\beta}} \frac{\partial r_l^{\alpha\beta}}{\partial X_k^\gamma} \quad (103)$$

$$= \left( \frac{\phi_{rr}(r^{\alpha\beta})}{r^{\alpha\beta}} - \frac{\phi_r(r^{\alpha\beta})}{(r^{\alpha\beta})^2} \right) \frac{r_k^{\alpha\beta}}{r^{\alpha\beta}} (\delta^{\beta\gamma} - \delta^{\alpha\gamma}) \quad (104)$$

where use is made of Eq. (66) in the third equality. Using Eq. (104), we can write Eq. (101) as

$$\begin{aligned} \Xi_{ijk}^\gamma &= \sum_{\alpha, \beta} \left( R_i^{\alpha\beta} R_j^{\alpha\beta} + X_m^{\alpha\beta} R_n^{\alpha\beta} \frac{\partial A_{mn}}{\partial \epsilon_{ij}} \Big|_{\mathbf{X}^\alpha} \right) \left( \frac{\phi_{rr}(r^{\alpha\beta})}{r^{\alpha\beta}} - \frac{\phi_r(r^{\alpha\beta})}{(r^{\alpha\beta})^2} \right) \frac{r_k^{\alpha\beta}}{r^{\alpha\beta}} (\delta^{\beta\gamma} - \delta^{\alpha\gamma}) \\ &\quad + \sum_{\alpha \neq \gamma} \frac{\phi_r(r^{\alpha\gamma})}{r^{\alpha\gamma}} R_n^{\alpha\gamma} \left( \frac{\partial A_{kn}}{\partial \epsilon_{ij}} \Big|_{\mathbf{X}^\alpha} \right) \end{aligned} \quad (105)$$

$$\begin{aligned} &= \sum_{\alpha \neq \gamma} \left( R_i^{\alpha\gamma} R_j^{\alpha\gamma} + X_m^{\alpha\gamma} R_n^{\alpha\gamma} \frac{\partial A_{mn}}{\partial \epsilon_{ij}} \Big|_{\mathbf{X}^\alpha} \right) \left( \frac{\phi_{rr}(r^{\alpha\gamma})}{r^{\alpha\gamma}} - \frac{\phi_r(r^{\alpha\gamma})}{(r^{\alpha\gamma})^2} \right) \frac{r_k^{\alpha\gamma}}{r^{\alpha\gamma}} \\ &\quad + \sum_{\alpha \neq \gamma} \frac{\phi_r(r^{\alpha\gamma})}{r^{\alpha\gamma}} R_n^{\alpha\gamma} \left( \frac{\partial A_{kn}}{\partial \epsilon_{ij}} \Big|_{\mathbf{X}^\alpha} \right). \end{aligned} \quad (106)$$

We now evaluate Eq. (106) at  $\epsilon_{ij} = 0$ , which makes any term proportional to  $X_m^{\alpha\beta}$  vanishes and  $r_i^\alpha = R_i^\alpha$ . The second term in Eq. (106) also vanishes as it is proportional to the force evaluated at the reference configuration when  $\epsilon_{ij} = 0$ , which by definition also vanishes, i.e.,

$$\sum_{\alpha \neq \gamma} \frac{\phi_r(R^{\alpha\gamma})}{R^{\alpha\gamma}} R_n^{\alpha\gamma} \left( \frac{\partial A_{kn}}{\partial \epsilon_{ij}} \Big|_{\mathbf{X}^\alpha} \right) = \left( \frac{\partial A_{kn}}{\partial \epsilon_{ij}} \Big|_{\mathbf{X}^\alpha} \right) \sum_{\alpha \neq \gamma} \frac{\phi_r(R^{\alpha\gamma})}{R^{\alpha\gamma}} R_n^{\alpha\gamma} = - \left( \frac{\partial A_{kn}}{\partial \epsilon_{ij}} \Big|_{\mathbf{X}^\alpha} \right) F_n^\gamma(R^{\alpha\gamma}) = 0. \quad (107)$$

Thus, from Eq. (106), we are left with the following expression

$$\Xi_{ijk}^\gamma = \sum_{\alpha \neq \gamma} (\phi_{rr}(R^{\alpha\gamma}) R^{\alpha\gamma} - \phi_r(R^{\alpha\gamma})) \frac{R_k^{\alpha\gamma} R_i^{\alpha\gamma} R_j^{\alpha\gamma}}{(R^{\alpha\gamma})^3}. \quad (108)$$

Finally, we compute the Hessian  $H_{mn}^{\alpha\beta}$ ,

$$H_{mn}^{\alpha\beta} = \frac{\partial^2 U}{\partial r_m^\alpha \partial r_n^\beta} = \frac{\partial^2 U}{\partial r_n^\beta \partial r_m^\alpha} \quad (109)$$

$$= -\frac{\partial F_m^\alpha}{\partial r_n^\beta} = \frac{\partial}{\partial r_n^\beta} \sum_{\gamma \neq \alpha} \phi_r(r^{\gamma\alpha}) \frac{r_m^{\gamma\alpha}}{r^{\gamma\alpha}} \quad (110)$$

$$= \sum_{\gamma \neq \alpha} \frac{\phi_r(r^{\gamma\alpha})}{r^{\gamma\alpha}} \frac{\partial r_m^{\gamma\alpha}}{\partial r_n^\beta} + \sum_{\gamma \neq \alpha} r_m^{\gamma\alpha} \frac{\partial}{\partial r_n^\beta} \left( \frac{\phi_r(r^{\gamma\alpha})}{r^{\gamma\alpha}} \right) \quad (111)$$

$$= \sum_{\gamma \neq \alpha} \frac{\phi_r(r^{\gamma\alpha})}{r^{\gamma\alpha}} \frac{\partial}{\partial r_n^\beta} (r_m^\alpha - r_m^\gamma) + \sum_{\gamma \neq \alpha} r_m^{\gamma\alpha} \left[ \frac{\phi_{rr}(r^{\gamma\alpha})}{r^{\gamma\alpha}} - \frac{\phi_r(r^{\gamma\alpha})}{(r^{\gamma\alpha})^2} \right] \frac{\partial r^{\gamma\alpha}}{\partial r_n^\beta} \quad (112)$$

$$= \sum_{\gamma \neq \alpha} \frac{\phi_r(r^{\gamma\alpha})}{r^{\gamma\alpha}} \delta_{mn} (\delta^{\alpha\beta} - \delta^{\gamma\beta}) + \sum_{\gamma \neq \alpha} \frac{r_m^{\gamma\alpha} r_n^{\gamma\alpha}}{r^{\gamma\alpha}} \left[ \frac{\phi_{rr}(r^{\gamma\alpha})}{r^{\gamma\alpha}} - \frac{\phi_r(r^{\gamma\alpha})}{(r^{\gamma\alpha})^2} \right] (\delta^{\alpha\beta} - \delta^{\gamma\beta}). \quad (113)$$

Let the off-diagonal term be  $\tilde{H}_{mn}^{\alpha\beta}$  ( $\alpha \neq \beta$ ), then

$$\tilde{H}_{mn}^{\alpha\beta} = \sum_{\gamma \neq \alpha} \frac{\phi_r(r^{\gamma\alpha})}{r^{\gamma\alpha}} \delta_{mn} (0 - \delta^{\gamma\beta}) + \sum_{\gamma \neq \alpha} \frac{r_m^{\gamma\alpha} r_n^{\gamma\alpha}}{r^{\gamma\alpha}} \left[ \frac{\phi_{rr}(r^{\gamma\alpha})}{r^{\gamma\alpha}} - \frac{\phi_r(r^{\gamma\alpha})}{(r^{\gamma\alpha})^2} \right] (0 - \delta^{\gamma\beta}) \quad (114)$$

$$= -\frac{\phi_r(r^{\beta\alpha})}{r^{\beta\alpha}} \delta_{mn} - \frac{r_m^{\beta\alpha} r_n^{\beta\alpha}}{r^{\beta\alpha}} \left[ \frac{\phi_{rr}(r^{\beta\alpha})}{r^{\beta\alpha}} - \frac{\phi_r(r^{\beta\alpha})}{(r^{\beta\alpha})^2} \right] \quad (115)$$

$$= -\frac{\phi_r(r^{\alpha\beta})}{r^{\alpha\beta}} \delta_{mn} - \frac{r_m^{\alpha\beta} r_n^{\alpha\beta}}{(r^{\alpha\beta})^2} \left[ \phi_{rr}(r^{\alpha\beta}) - \frac{\phi_r(r^{\alpha\beta})}{r^{\alpha\beta}} \right]. \quad (116)$$

Next, we look at the diagonal terms ( $\alpha = \beta$ )

$$H_{mn}^{\alpha\alpha} = \sum_{\gamma \neq \alpha} \frac{\phi_r(r^{\gamma\alpha})}{r^{\gamma\alpha}} \delta_{mn} (1 - 0) + \sum_{\gamma \neq \alpha} \frac{r_m^{\gamma\alpha} r_n^{\gamma\alpha}}{r^{\gamma\alpha}} \left[ \frac{\phi_{rr}(r^{\gamma\alpha})}{r^{\gamma\alpha}} - \frac{\phi_r(r^{\gamma\alpha})}{(r^{\gamma\alpha})^2} \right] (1 - 0) \quad (117)$$

$$= \sum_{\gamma \neq \alpha} \frac{\phi_r(r^{\gamma\alpha})}{r^{\gamma\alpha}} \delta_{mn} + \frac{r_m^{\gamma\alpha} r_n^{\gamma\alpha}}{r^{\gamma\alpha}} \left[ \frac{\phi_{rr}(r^{\gamma\alpha})}{r^{\gamma\alpha}} - \frac{\phi_r(r^{\gamma\alpha})}{(r^{\gamma\alpha})^2} \right] = -\sum_{\gamma \neq \alpha} \tilde{H}_{mn}^{\gamma\alpha}. \quad (118)$$

The Hessian when  $\epsilon_{ij} = 0$  can be found by setting  $r_i^\alpha = R_i^\alpha$ ,

$$H_{mn}^{\alpha\beta} = \begin{cases} \tilde{H}_{mn}^{\alpha\beta} & \alpha \neq \beta \\ -\sum_{\gamma \neq \alpha} \tilde{H}_{mn}^{\gamma\alpha} & \alpha = \beta \end{cases} \quad (119)$$

where at zero strain

$$\tilde{H}_{mn}^{\alpha\beta} = -\frac{\phi_r(R^{\alpha\beta})}{R^{\alpha\beta}} \delta_{mn} - \frac{R_m^{\alpha\beta} R_n^{\alpha\beta}}{(R^{\alpha\beta})^2} \left[ \phi_{rr}(R^{\alpha\beta}) - \frac{\phi_r(R^{\alpha\beta})}{R^{\alpha\beta}} \right]. \quad (120)$$

Using Eqs. (84), (94) and (108), we can summarize the elasticity tensor as follows:

$$C_{ijkl} = C_{ijkl}^B + C_{ijkl}^{\text{NA}}, \quad (121)$$

where  $C_{ijkl}^B$  is the Born contribution given by

$$C_{ijkl}^B = \frac{1}{V} \sum_{\alpha, \beta} \left[ \phi_{rr}(R^{\alpha\beta}) R^{\alpha\beta} - \phi_r(R^{\alpha\beta}) \right] \frac{R_i^{\alpha\beta} R_j^{\alpha\beta} R_k^{\alpha\beta} R_l^{\alpha\beta}}{(R^{\alpha\beta})^3}, \quad (122)$$

$C_{ijkl}^{\text{NA}}$  is the non-affine contribution given by

$$C_{ijkl}^{\text{NA}} = -\frac{1}{V} \Xi_{ijm}^\alpha (H_{mn}^{\alpha\beta})^+ \Xi_{kln}^\beta, \quad (123)$$

with  $\Xi_{ijm}^\alpha$  given by Eq. (108), and  $H_{mn}^{\alpha\beta}$  given by Eqs. (119) and (120).

## 2 A Rate Theory for Elastic Dipole Excitations

We now use the field theory described in Section 1.1 to derive an analytical expression for the excitation energy barrier  $J_\sigma$ . To this end, a rate theory of localized excitations was constructed in Section V of the main text by matching the excitation energy barrier  $J_\sigma$  to an energy barrier  $\Delta F^\ddagger$  computed from transition state theory (TST). Combining TST with the field theory presented in Section 1.1, we may compute  $\Delta F^\ddagger$  from the elastic strain energy given by Eq. (33) and by modeling the excitation as a localized form of pure shear induced by force dipoles. The elastic stress field given any force-dipole configuration is derived in Section 2.1, which is then applied to derive an analytical formula for  $\Delta F^\ddagger$  in Section 2.2.

### 2.1 Review of Force Dipoles in Elasticity Theory

For any given force dipole, their elastic fields can be computed through the method of Green's functions. Given a single point force  $\mathbf{f}(\mathbf{x} - \mathbf{a}) = f_i \delta(\mathbf{x} - \mathbf{a}) \mathbf{e}_i$  located at  $\mathbf{x} = \mathbf{a}$ , the induced displacement field is given by a Green's function  $\mathbf{G}(\mathbf{x}) = G_{ij}(\mathbf{x}) \mathbf{e}_i \otimes \mathbf{e}_j$ ,

$$u_i(\mathbf{x}) = \int d^d \mathbf{x}' G_{ij}(\mathbf{x} - \mathbf{x}') f_j(\mathbf{x}' - \mathbf{a}). \quad (124)$$

Let the Fourier transform of any function  $f(\mathbf{x})$  and its inverse be defined as

$$\hat{f}(\mathbf{k}) = \int d^d \mathbf{x} f(\mathbf{x}) e^{-i\mathbf{k} \cdot \mathbf{x}}; \quad f(\mathbf{x}) = \int \frac{d^d \mathbf{k}}{(2\pi)^d} \hat{f}(\mathbf{k}) e^{i\mathbf{k} \cdot \mathbf{x}}. \quad (125)$$

The Green's function in Fourier space  $\hat{\mathbf{G}}(\mathbf{k}) = \int d^d \mathbf{x} \mathbf{G}(\mathbf{x}) e^{-i\mathbf{k} \cdot \mathbf{x}} = \hat{G}_{ij}(\mathbf{k}) \mathbf{e}_i \otimes \mathbf{e}_j$  in any given dimension for an elastic system, which corresponds to elasticity of inherent states, can be written as [6]

$$\hat{G}_{ij}(\mathbf{k}) = \frac{1}{G^{\text{IS}} k^2} \left( \delta_{ij} - \frac{\lambda^{\text{IS}} + G^{\text{IS}}}{\lambda^{\text{IS}} + 2G^{\text{IS}}} \frac{k_i k_j}{k^2} \right) = \frac{1}{G^{\text{IS}} k^2} \left( \delta_{ij} - \frac{\nu^{\text{IS}} + 1}{2} \frac{k_i k_j}{k^2} \right), \quad (126)$$

$$\hat{u}_i(\mathbf{k}) = \hat{G}_{ij}(\mathbf{k}) \hat{f}_j(\mathbf{k}) \quad (127)$$

where  $k = |\mathbf{k}|$ ,  $\hat{f}_j = f_j e^{-i\mathbf{k} \cdot \mathbf{a}}$ , and the second equality in Eq. (126) makes use of the definition for Poisson's ratio in Eq. (39).

From Eq. (126), we can derive a formula relating the stress due to a point force. To this end, we first derive the strain tensor in Fourier space using Eq. (126) as

$$\hat{\epsilon}_{ij} = \frac{i}{2} (k_j u_i + k_i u_j) = \frac{i}{2} (k_j \hat{G}_{ik} + k_i \hat{G}_{jk}) \hat{f}_k \quad (128)$$

$$= \frac{i}{2} \left( \frac{k_j}{G^{\text{IS}} k^2} \left( \delta_{ik} - \frac{\nu^{\text{IS}} + 1}{2} \frac{k_i k_k}{k^2} \right) + \frac{k_i}{G^{\text{IS}} k^2} \left( \delta_{jk} - \frac{\nu^{\text{IS}} + 1}{2} \frac{k_j k_k}{k^2} \right) \right) \hat{f}_k \quad (129)$$

$$= \frac{i}{2G^{\text{IS}} k^2} \left( k_j \delta_{ik} + k_i \delta_{jk} - (\nu^{\text{IS}} + 1) \frac{k_i k_j k_k}{k^2} \right) \hat{f}_k. \quad (130)$$

Since the constitutive law in Eq. (41) is linear, it also holds in Fourier space:

$$\hat{T}_{ij} = 2G^{\text{IS}} \hat{\epsilon}_{ij} + \lambda^{\text{IS}} (\hat{\epsilon}_{kk}) \delta_{ij} = 2G^{\text{IS}} \left( \hat{\epsilon}_{ij} + \frac{\nu^{\text{IS}}}{1 - \nu^{\text{IS}}} \hat{\epsilon}_{kk} \delta_{ij} \right). \quad (131)$$

Substituting Eq. (130) into Eq. (131) yields

$$\hat{T}_{ij} = \frac{i}{k^2} \left( \left( k_j \delta_{ik} + k_i \delta_{jk} - (\nu^{\text{IS}} + 1) \frac{k_i k_k k_j}{k^2} \right) \hat{f}_k + \frac{\nu^{\text{IS}} \delta_{ij}}{1 - \nu^{\text{IS}}} \left( 2k_k \delta_{kl} - (\nu^{\text{IS}} + 1) \frac{k_k k_l k_k}{k^2} \right) \hat{f}_l \right) \quad (132)$$

$$= \frac{i}{k^2} \left( \left( k_j \hat{f}_i + k_i \hat{f}_j - (\nu^{\text{IS}} + 1) \frac{k_i k_k k_j \hat{f}_k}{k^2} \right) + \frac{\nu^{\text{IS}} \delta_{ij}}{1 - \nu^{\text{IS}}} \left( 2k_l \hat{f}_l - (\nu^{\text{IS}} + 1) k_l \hat{f}_l \right) \right) \quad (133)$$

$$= \frac{i}{k^2} \left( \left( k_j \hat{f}_i + k_i \hat{f}_j - (\nu^{\text{IS}} + 1) \frac{k_i k_k k_j \hat{f}_k}{k^2} \right) + \left( \nu^{\text{IS}} k_l \hat{f}_l \right) \delta_{ij} \right) \quad (134)$$

$$= \frac{i}{k^2} \left( k_j \hat{f}_i + k_i \hat{f}_j + k_k \hat{f}_k \left( -(\nu^{\text{IS}} + 1) \frac{k_i k_j}{k^2} + \nu^{\text{IS}} \delta_{ij} \right) \right). \quad (135)$$

where the dummy index is switched from  $l \rightarrow k$  to get to the last equality.

We can also obtain the stress due to a point force in real-space. First, substitute the expression for  $\hat{f}_i = f_i e^{-i\mathbf{k} \cdot \mathbf{a}}$  into Eq. (135) to get

$$\hat{T}_{ij} = \hat{G}_{ijk}(\mathbf{k}) f_k e^{-i\mathbf{k} \cdot \mathbf{a}}, \quad (136)$$

$$\hat{G}_{ijk}(\mathbf{k}) = \frac{i}{k^2} \left( k_j \delta_{ik} + k_i \delta_{jk} + \left( -(\nu^{\text{IS}} + 1) \frac{k_i k_k k_j}{k^2} + \nu^{\text{IS}} k_k \delta_{ij} \right) \right) \quad (137)$$

where  $\hat{G}_{ijk}(\mathbf{k})$  is the Green's function relating a point force at the origin with the elastic stress. Applying inverse Fourier transform to both sides of Eq. (136),

$$T_{ij}(\mathbf{x} - \mathbf{a}; \mathbf{f}) = \left( \int \frac{d^2 \mathbf{k}}{(2\pi)^2} \hat{G}_{ijk}(\mathbf{k}) e^{i\mathbf{k} \cdot (\mathbf{x} - \mathbf{a})} \right) f_k \quad (138)$$

$$\equiv G_{ijk}(\mathbf{x} - \mathbf{a}) f_k \quad (139)$$

where  $T_{ij}(\mathbf{x} - \mathbf{a}; \mathbf{f})$  denotes the stress due to a point force located at  $\mathbf{x} = \mathbf{a}$ . From Eq. (139), we can establish a sign permutation relation:

$$T_{ij}(\mathbf{x} - \mathbf{a}; -\mathbf{f}) = -T_{ij}(\mathbf{x} - \mathbf{a}; \mathbf{f}), \quad (140)$$

which is important in later steps.

Following [6], suppose that we have  $N$ -many point forces and denote the  $q$ -th point force and its location about the origin as  $\mathbf{f}^{(q)}$  and  $\mathbf{a}^{(q)}$  respectively. Using Eq. (139), the total stress can be written as

$$T_{ij} = \sum_{q=1}^N T_{ij}(\mathbf{x} - \mathbf{a}^{(q)}; \mathbf{f}^{(q)}) = \sum_{q=1}^N G_{ijk}(\mathbf{x} - \mathbf{a}^{(q)}) f_k^{(q)}. \quad (141)$$

If the point forces are close to the origin, then a Taylor series expansion around  $\mathbf{a}^{(q)} = 0$  gives

$$T_{ij} \approx \sum_{q=1}^N \left[ G_{ijk}(\mathbf{x}) - G_{ijk,l}(\mathbf{x}) a_l^{(q)} \right] f_k^{(q)} \quad (142)$$

$$\approx G_{ijk}(\mathbf{x}) \left( \sum_{q=1}^N f_k^{(q)} \right) - G_{ijk,l}(\mathbf{x}) \left( \sum_{q=1}^N f_k^{(q)} a_l^{(q)} \right). \quad (143)$$

Let  $p_i \equiv \sum_{q=1}^N f_i^{(q)}$  be the force monopole vector and  $P_{ij} \equiv \sum_{q=1}^N f_i^{(q)} a_j^{(q)}$  be the force dipole tensor. At mechanical equilibrium, sum of forces must be zero, i.e.,  $p_i = 0$ , and thus Eq. (143) retains only its second term

$$T_{ij} \approx -G_{ijk,l} P_{kl} \quad (144)$$

or in Fourier space,

$$\hat{T}_{ij} \approx -i\hat{G}_{ijk} k_l P_{kl} = \hat{G}_{ijkl} P_{kl} \quad (145)$$

where  $\hat{G}_{ijkl}$  is the Green's function relating stress and dipole tensors. In 2D, we can write Eq. (145) in matrix form as

$$\begin{bmatrix} \hat{T}_{xx} \\ \hat{T}_{yy} \\ \hat{T}_{xy} \end{bmatrix} = \begin{bmatrix} \hat{G}_{xxxx} & \hat{G}_{xxyy} & \hat{G}_{xxxy} \\ \hat{G}_{yyxx} & \hat{G}_{yyyy} & \hat{G}_{yyxy} \\ \hat{G}_{xyxx} & \hat{G}_{xyyy} & \hat{G}_{xyxy} \end{bmatrix} \begin{bmatrix} P_{xx} \\ P_{yy} \\ P_{xy} \end{bmatrix}. \quad (146)$$

Note that the strain energy given by the field theory in Eq. (52) is written in terms of the principal components of the stress

$$\hat{T}_1 = -\frac{1}{2} (\hat{T}_{xx} + \hat{T}_{yy}); \quad \hat{T}_2 = \frac{1}{2} (\hat{T}_{yy} - \hat{T}_{xx}); \quad \hat{T}_3 = \hat{T}_{xy}. \quad (147)$$

Thus, we also need to express Eq. (146) in terms of these components. To this end, let the principal components for the force dipole tensor be defined as

$$P_1 = -\frac{1}{2} (P_{xx} + P_{yy}); \quad P_2 = \frac{1}{2} (P_{yy} - P_{xx}); \quad P_3 = P_{xy}. \quad (148)$$

Applying Eq. (147) and Eq. (148) to Eq. (146), we obtain

$$\begin{bmatrix} \hat{T}_1 \\ \hat{T}_2 \\ \hat{T}_3 \end{bmatrix} = \begin{bmatrix} -\frac{1}{2} & -\frac{1}{2} & 0 \\ -\frac{1}{2} & \frac{1}{2} & 0 \\ 0 & 0 & 1 \end{bmatrix} \begin{bmatrix} \hat{G}_{xxxx} & \hat{G}_{xxyy} & \hat{G}_{xxxy} \\ \hat{G}_{yyxx} & \hat{G}_{yyyy} & \hat{G}_{yyxy} \\ \hat{G}_{xyxx} & \hat{G}_{xyyy} & \hat{G}_{xyxy} \end{bmatrix} \begin{bmatrix} -\frac{1}{2} & -\frac{1}{2} & 0 \\ -\frac{1}{2} & \frac{1}{2} & 0 \\ 0 & 0 & 1 \end{bmatrix}^{-1} \begin{bmatrix} P_1 \\ P_2 \\ P_3 \end{bmatrix} \quad (149)$$

$$\equiv \underbrace{\begin{bmatrix} \hat{G}_{11} & \hat{G}_{12} & \hat{G}_{13} \\ \hat{G}_{21} & \hat{G}_{22} & \hat{G}_{23} \\ \hat{G}_{31} & \hat{G}_{32} & \hat{G}_{33} \end{bmatrix}}_{\hat{\mathcal{G}}} \begin{bmatrix} P_1 \\ P_2 \\ P_3 \end{bmatrix} \quad (150)$$

where the  $3 \times 3$  matrix  $\hat{\mathcal{G}}$  is the Green's function relating principal components of stress and dipole tensors. Thus, as long as  $\hat{\mathcal{G}}$  is known, the stress due to any force-dipole configuration can be obtained.

In 2D,  $\hat{\mathcal{G}}$  can be derived using a trick paraphrased in the Supplemental Material of [7]. The trick proceeds by choosing a test dipole, which yields a simple formula as a function of the stress from a point force in Eq. (139). Then, the derived expression can be compared with one based on the  $\hat{\mathcal{G}}$  matrix and force dipole tensor  $P_{ij}$  (in Eq. (150)), and each component of  $\hat{\mathcal{G}}$  will be deduced term-by-term.

The test dipole chosen for this trick is a co-linear force dipole made of a point force  $+\mathbf{f}$  at  $+\mathbf{a}$  and another point force  $-\mathbf{f}$  at  $-\mathbf{a}$  where

$$\mathbf{f} = [f \cos \psi, f \sin \psi]; \quad \mathbf{a} = [a \cos \psi, a \sin \psi] \quad (151)$$

and  $\psi$  is the dipole orientation angle. Its co-linearity allows the stress to be simply computed from Eq. (139) and the sign permutation relation in Eq. (140):

$$T_{ij} = T_{ij}(\mathbf{x} - \mathbf{a}; \mathbf{f}) + T_{ij}(\mathbf{x} + \mathbf{a}; -\mathbf{f}) = T_{ij}(\mathbf{x} - \mathbf{a}; \mathbf{f}) - T_{ij}(\mathbf{x} + \mathbf{a}; \mathbf{f}) = -2a_k T_{ij,k}(\mathbf{x}; \mathbf{f}) + O(|\mathbf{a}|^2) \quad (152)$$

where the last equality is obtained by a Taylor series expansion around  $\mathbf{a} = 0$  truncated at first order. Switching to polar coordinates in Fourier space, where  $\mathbf{k} = [k \cos \phi, k \sin \phi]$ , the stress tensor becomes

$$\hat{T}_{ij} = -2ia_k k_k \hat{T}_{ij}(k, \phi; \mathbf{f}) = -2i(\mathbf{a} \cdot \mathbf{k}) \hat{T}_{ij}(k, \phi; \mathbf{f}) \quad (153)$$

where  $\mathbf{a} \cdot \mathbf{k} = a_k k_k$  and  $\hat{T}_{ij}(k, \phi; \mathbf{f})$  is the point-force stress in Fourier space, whose explicit formula is already given in Eq. (135). Using Eq. (153) and Eq. (147), the principal components of the stress can be written as

$$\hat{T}_1 = i(\mathbf{a} \cdot \mathbf{k}) \left( \hat{T}_{xx}(k, \phi; \mathbf{f}) + \hat{T}_{yy}(k, \phi; \mathbf{f}) \right), \quad (154)$$

$$\hat{T}_2 = -i(\mathbf{a} \cdot \mathbf{k}) \left( \hat{T}_{yy}(k, \phi; \mathbf{f}) - \hat{T}_{xx}(k, \phi; \mathbf{f}) \right), \quad (155)$$

$$\hat{T}_3 = -2i(\mathbf{a} \cdot \mathbf{k}) \hat{T}_{xy}(k, \phi; \mathbf{f}). \quad (156)$$

For the co-linear dipole, the dipole tensor  $P_{ij}$  is given by

$$P_{ij} \mathbf{e}_i \otimes \mathbf{e}_j = \begin{bmatrix} (+f_x)(+a_x) & (+f_x)(+a_y) \\ (+f_y)(+a_x) & (+f_y)(+a_y) \end{bmatrix} + \begin{bmatrix} (-f_x)(-a_x) & (-f_x)(-a_y) \\ (-f_y)(-a_x) & (-f_y)(-a_y) \end{bmatrix} \quad (157)$$

$$= 2af \begin{bmatrix} \cos^2 \psi & \cos \psi \sin \psi \\ \cos \psi \sin \psi & \sin^2 \psi \end{bmatrix}, \quad (158)$$

whose principal components are

$$P_1 = -\frac{1}{2}(P_{xx} + P_{yy}) = -\frac{2af}{2}(\cos^2 \psi + \sin^2 \psi) = -af \quad (159)$$

$$P_2 = \frac{1}{2}(P_{yy} - P_{xx}) = af(\sin^2 \psi - \cos^2 \psi) = -af \cos 2\psi \quad (160)$$

$$P_3 = P_{xy} = 2af \cos \psi \sin \psi = af \sin 2\psi. \quad (161)$$

Thus, using Eq. (150), we obtain an alternative expression for the dipole's stress

$$\begin{bmatrix} \hat{T}_1 \\ \hat{T}_2 \\ \hat{T}_3 \end{bmatrix} = \begin{bmatrix} \hat{\mathcal{G}}_{11}P_1 + \hat{\mathcal{G}}_{12}P_2 + \hat{\mathcal{G}}_{13}P_3 \\ \hat{\mathcal{G}}_{21}P_1 + \hat{\mathcal{G}}_{22}P_2 + \hat{\mathcal{G}}_{23}P_3 \\ \hat{\mathcal{G}}_{31}P_1 + \hat{\mathcal{G}}_{32}P_2 + \hat{\mathcal{G}}_{33}P_3 \end{bmatrix} = af \begin{bmatrix} -\hat{\mathcal{G}}_{11} - \hat{\mathcal{G}}_{12} \cos 2\psi + \hat{\mathcal{G}}_{13} \sin 2\psi \\ -\hat{\mathcal{G}}_{21} - \hat{\mathcal{G}}_{22} \cos 2\psi + \hat{\mathcal{G}}_{23} \sin 2\psi \\ -\hat{\mathcal{G}}_{31} - \hat{\mathcal{G}}_{32} \cos 2\psi + \hat{\mathcal{G}}_{33} \sin 2\psi \end{bmatrix}. \quad (162)$$

At this stage, we may deduce each component of  $\hat{\mathcal{G}}$  by computing every stress component in Eqs. (154) to (156) using the point-force stress formula given in Eq. (135) and compare those expressions with Eq. (162). For the next steps, the following trigonometric identities will be useful

$$(\cos \phi \cos \psi + \sin \phi \sin \psi)^2 = \frac{1}{2}(1 + \cos 2\phi \cos 2\psi + \sin 2\phi \sin 2\psi), \quad (163)$$

$$(\cos \phi \cos \psi + \sin \phi \sin \psi)(\cos \phi \cos \psi - \sin \phi \sin \psi) = \frac{1}{2}(\cos 2\psi + \cos 2\phi), \quad (164)$$

$$(\sin \phi \cos \psi + \cos \phi \sin \psi)(\sin \phi \sin \psi + \cos \phi \cos \psi) = \frac{1}{2}(\sin 2\psi + \sin 2\phi). \quad (165)$$

First, we compute  $\hat{T}_1$ . From Eq. (154) and Eq. (135), we have

$$\hat{T}_1 = \frac{i^2 \mathbf{a} \cdot \mathbf{k}}{k^2} \left( 2k_x \hat{f}_x + 2k_y \hat{f}_y + \mathbf{k} \cdot \hat{\mathbf{f}} \left( -(\nu^{\text{IS}} + 1) \frac{k_x k_x + k_y k_y}{k^2} + \nu^{\text{IS}} (\delta_{xx} + \delta_{yy}) \right) \right) \quad (166)$$

$$= -\frac{\mathbf{a} \cdot \mathbf{k}(\mathbf{k} \cdot \hat{\mathbf{f}})}{k^2} (2 + (-(\nu^{\text{IS}} + 1) + 2\nu^{\text{IS}})) = -\frac{\mathbf{a} \cdot \mathbf{k}(\mathbf{k} \cdot \hat{\mathbf{f}})}{k^2} (\nu^{\text{IS}} + 1). \quad (167)$$

Also note that

$$\mathbf{a} \cdot \mathbf{k}(\mathbf{k} \cdot \hat{\mathbf{f}}) = afk^2 (\cos \phi \cos \psi + \sin \phi \sin \psi)^2 \quad (168)$$

$$= \frac{afk^2}{2} (1 + \cos 2\phi \cos 2\psi + \sin 2\phi \sin 2\psi) \quad (169)$$

where the second line is obtained by substituting the first trigonometric identity Eq. (163) into the first line. Using Eq. (169),  $\hat{T}_1$  is reduced to

$$\hat{T}_1 = -\frac{afk^2}{k^2} \frac{\nu^{\text{IS}} + 1}{2} (1 + \cos 2\phi \cos 2\psi + \sin 2\phi \sin 2\psi) \quad (170)$$

$$= af \left[ -\left( \frac{\nu^{\text{IS}} + 1}{2} \right) - \left( \frac{\nu^{\text{IS}} + 1}{2} \cos 2\phi \right) \cos 2\psi + \left( -\frac{\nu^{\text{IS}} + 1}{2} \sin 2\phi \right) \sin 2\psi \right]. \quad (171)$$

Equation (171) can now be compared with the first row of Eq. (162) to give us

$$\hat{G}_{11} = \frac{\nu^{\text{IS}} + 1}{2}; \quad \hat{G}_{12} = \frac{\nu^{\text{IS}} + 1}{2} \cos 2\phi; \quad \hat{G}_{13} = -\frac{\nu^{\text{IS}} + 1}{2} \sin 2\phi. \quad (172)$$

Next, we compute  $\hat{T}_2$  using Eq. (155) and Eq. (135) as

$$\hat{T}_2 = -i \mathbf{a} \cdot \mathbf{k} \frac{i}{k^2} \left( 2k_y \hat{f}_y - 2k_x \hat{f}_x + \mathbf{k} \cdot \hat{\mathbf{f}} \left( -(\nu^{\text{IS}} + 1) \frac{k_y k_y - k_x k_x}{k^2} + \nu^{\text{IS}} (\delta_{yy} - \delta_{xx}) \right) \right) \quad (173)$$

$$= \frac{\mathbf{a} \cdot \mathbf{k}}{k^2} \left( 2(k_y \hat{f}_y - k_x \hat{f}_x) + \mathbf{k} \cdot \hat{\mathbf{f}} \left( -(\nu^{\text{IS}} + 1) \frac{k_y k_y - k_x k_x}{k^2} \right) \right). \quad (174)$$

Note that  $\frac{k_y k_y - k_x k_x}{k^2} = \sin^2 \phi - \cos^2 \phi = -\cos 2\phi$  and,

$$\mathbf{a} \cdot \mathbf{k} (k_y \hat{f}_y - k_x \hat{f}_x) = akf^2 (\cos \phi \cos \psi + \sin \phi \sin \psi) (\sin \phi \sin \psi - \cos \phi \cos \psi) \quad (175)$$

$$= -\frac{akf^2}{2} (\cos 2\phi + \cos 2\psi) \quad (176)$$

where the second equality is obtained by using the second trigonometric identity Eq. (164). Combining Eq. (176) with Eq. (169), we can further reduce  $\hat{T}_2$  into

$$\hat{T}_2 = \frac{afk^2}{k^2} \left( -\cos 2\phi - \cos 2\psi + \frac{(\nu^{\text{IS}} + 1)}{2} (1 + \cos 2\phi \cos 2\psi + \sin 2\phi \sin 2\psi) \cos 2\phi \right) \quad (177)$$

$$= af \left( \frac{\nu^{\text{IS}} - 1}{2} \cos 2\phi - \left( 1 - \frac{\nu^{\text{IS}} + 1}{2} (\cos^2 2\phi) \right) \cos 2\psi + \frac{\nu^{\text{IS}} + 1}{2} \sin 2\phi \cos 2\phi \sin 2\psi \right) \quad (178)$$

$$= af \left( \frac{\nu^{\text{IS}} - 1}{2} \cos 2\phi - \left( 1 - \frac{\nu^{\text{IS}} + 1}{4} (1 + \cos 4\phi) \right) \cos 2\psi + \frac{\nu^{\text{IS}} + 1}{4} \sin 4\phi \sin 2\psi \right) \quad (179)$$

$$= af \left( -\left( -\frac{\nu^{\text{IS}} - 1}{2} \cos 2\phi \right) - \left( \frac{3 - \nu^{\text{IS}}}{4} - \frac{\nu^{\text{IS}} + 1}{4} \cos 4\phi \right) \cos 2\psi + \left( \frac{\nu^{\text{IS}} + 1}{4} \sin 4\phi \right) \sin 2\psi \right). \quad (180)$$

The last line can be compared with the second row of Eq. (162) to give us

$$\hat{\mathcal{G}}_{21} = -\frac{\nu^{\text{IS}} - 1}{2} \cos 2\phi; \quad \hat{\mathcal{G}}_{22} = \frac{3 - \nu^{\text{IS}}}{4} - \frac{\nu^{\text{IS}} + 1}{4} \cos 4\phi; \quad \hat{\mathcal{G}}_{23} = \frac{\nu^{\text{IS}} + 1}{4} \sin 4\phi. \quad (181)$$

Finally, we compute  $\hat{T}_3$ . Using Eq. (156) and Eq. (135),

$$\hat{T}_3 = -2i\mathbf{a} \cdot \mathbf{k} \frac{i}{k^2} \left( k_x \hat{f}_y + k_y \hat{f}_x + \mathbf{k} \cdot \hat{\mathbf{f}} \left( -(\nu^{\text{IS}} + 1) \frac{k_x k_y}{k^2} + \nu^{\text{IS}} \delta_{xy} \right) \right) \quad (182)$$

$$= \frac{2\mathbf{a} \cdot \mathbf{k}}{k^2} \left( k_x \hat{f}_y + k_y \hat{f}_x - \mathbf{k} \cdot \hat{\mathbf{f}} (\nu^{\text{IS}} + 1) \frac{k_x k_y}{k^2} \right). \quad (183)$$

Note that  $\frac{k_x k_y}{k^2} = \cos \phi \sin \phi = \frac{1}{2} \sin 2\phi$  and,

$$\mathbf{a} \cdot \mathbf{k} \left( k_x \hat{f}_y + k_y \hat{f}_x \right) = akf^2 (\cos \phi \cos \psi + \sin \phi \sin \psi) (\cos \phi \sin \psi + \sin \phi \cos \psi) \quad (184)$$

$$= \frac{akf^2}{2} (\sin 2\phi + \sin 2\psi) \quad (185)$$

where the second equality is obtained by substituting Eq. (165) into the first equality. Using Eq. (185) with Eq. (169), we can further reduce  $\hat{T}_3$  into

$$\hat{T}_3 = \frac{2afk^2}{k^2} \left( \frac{1}{2} (\sin 2\psi + \sin 2\phi) + \frac{1}{2} (1 + \cos 2\phi \cos 2\psi + \sin 2\phi \sin 2\psi) \left( -\frac{\nu^{\text{IS}} + 1}{2} \sin 2\phi \right) \right) \quad (186)$$

$$= af \left( (\sin 2\psi + \sin 2\phi) + (1 + \cos 2\phi \cos 2\psi + \sin 2\phi \sin 2\psi) \left( -\frac{\nu^{\text{IS}} + 1}{2} \sin 2\phi \right) \right) \quad (187)$$

$$= af \left( (\sin 2\psi + \sin 2\phi) - \frac{\nu^{\text{IS}} + 1}{2} \left( \sin 2\phi + \frac{1}{2} \sin 4\phi \cos 2\psi + \frac{1}{2} (1 - \cos 4\phi) \sin 2\psi \right) \right) \quad (188)$$

$$= af \left( -\left( \frac{\nu^{\text{IS}} - 1}{2} \sin 2\phi \right) - \left( \frac{\nu^{\text{IS}} + 1}{4} \sin 4\phi \right) \cos 2\psi + \left( \frac{3 - \nu^{\text{IS}}}{4} + \frac{\nu^{\text{IS}} + 1}{4} \cos 4\phi \right) \sin 2\psi \right). \quad (189)$$

The last line can be compared with Eq. (162) to give us

$$\hat{\mathcal{G}}_{31} = \frac{\nu^{\text{IS}} - 1}{2} \sin 2\phi; \quad \hat{\mathcal{G}}_{32} = \frac{\nu^{\text{IS}} + 1}{4} \sin 4\phi; \quad \hat{\mathcal{G}}_{33} = \frac{3 - \nu^{\text{IS}}}{4} + \frac{\nu^{\text{IS}} + 1}{4} \cos 4\phi. \quad (190)$$

Combining Eqs. (172), (181) and (190) together, the Green's function  $\hat{\mathcal{G}}$  relating the principal components of stress and dipole tensors is given by

$$\hat{\mathcal{G}} = \begin{bmatrix} \frac{\nu^{\text{IS}} + 1}{2} & \frac{\nu^{\text{IS}} + 1}{2} \cos 2\phi & -\frac{\nu^{\text{IS}} + 1}{2} \sin 2\phi \\ -\frac{\nu^{\text{IS}} - 1}{2} \cos 2\phi & \frac{3 - \nu^{\text{IS}}}{4} - \frac{\nu^{\text{IS}} + 1}{4} \cos 4\phi & \frac{\nu^{\text{IS}} + 1}{4} \sin 4\phi \\ \frac{\nu^{\text{IS}} - 1}{2} \sin 2\phi & \frac{\nu^{\text{IS}} + 1}{4} \sin 4\phi & \frac{3 - \nu^{\text{IS}}}{4} + \frac{\nu^{\text{IS}} + 1}{4} \cos 4\phi \end{bmatrix}. \quad (191)$$

To convert it to real-space polar coordinates  $(r, \theta)$ , the following identities for the 2D inverse Fourier transform are used [8]:

$$\int \frac{d^2 \mathbf{k}}{(2\pi)^2} f(k) \cos(2m\phi) e^{i\mathbf{k} \cdot \mathbf{x}} = (-1)^m \cos(2m\theta) \int_0^\infty \frac{dk}{2\pi} k f(k) J_{2m}(kr), \quad (192)$$

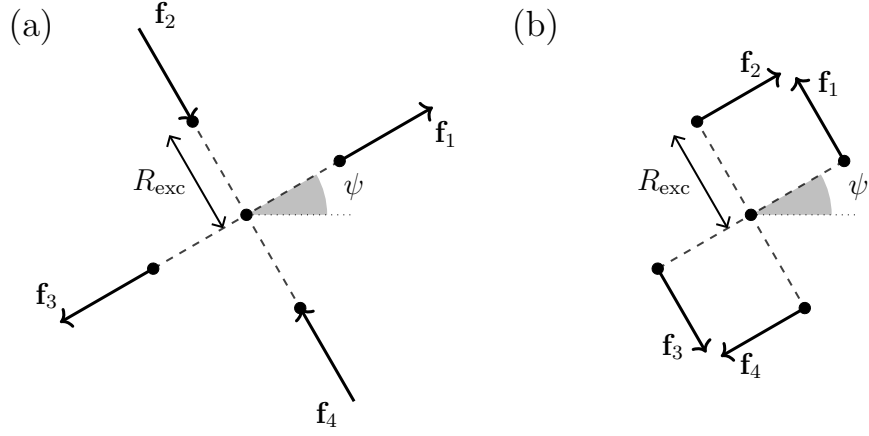

Figure S.3: An illustration of two force-dipole configurations that induce pure shear inside a region of radius  $R_{\text{exc}}$ . The two only differ by how the forces would be applied to some material element, but are related by an orientation of  $45^\circ$ .

$$\int \frac{d^2\mathbf{k}}{(2\pi)^2} f(k) \sin(2m\phi) e^{i\mathbf{k}\cdot\mathbf{x}} = (-1)^m \sin(2m\theta) \int_0^\infty \frac{dk}{2\pi} k f(k) J_{2m}(kr), \quad (193)$$

$$\frac{m}{r^2} = \int_0^\infty dk k J_m(kr) \quad (194)$$

where  $m$  is any positive integer and  $J_m(s)$  is the  $m$ -th order Bessel function of the first kind. Applying them to Eq. (191), we obtain

$$\mathcal{G} = \begin{bmatrix} \frac{\nu^{\text{IS}} + 1}{2} \delta(r) & -\frac{\nu^{\text{IS}} + 1}{2\pi r^2} \cos 2\theta & \frac{\nu^{\text{IS}} + 1}{2\pi r^2} \sin 2\theta \\ \frac{\nu^{\text{IS}} - 1}{2\pi r^2} \cos 2\theta & \frac{3 - \nu^{\text{IS}}}{4} \delta(r) - \frac{\nu^{\text{IS}} + 1}{2\pi r^2} \cos 4\theta & \frac{\nu^{\text{IS}} + 1}{2\pi r^2} \sin 4\theta \\ \frac{1 - \nu^{\text{IS}}}{2\pi r^2} \sin 2\theta & \frac{\nu^{\text{IS}} + 1}{2\pi r^2} \sin 4\theta & \frac{3 - \nu^{\text{IS}}}{4} \delta(r) + \frac{\nu^{\text{IS}} + 1}{2\pi r^2} \cos 4\theta \end{bmatrix}. \quad (195)$$

Equation (195) along with Eq. (150) can be used to compute the stress response of any force dipole configuration, including the ones that model an STZ. This computation is performed in the next section.

## 2.2 Computing the Energy Barrier for a Configuration of Force Dipoles

Let the elastic stress induced by an STZ be  $T_{ij}^\dagger$  and its principal components written as  $[T_1^\dagger, T_2^\dagger, T_3^\dagger]$ . Given the force-dipole configuration in Fig. S.3a, the position and force vectors can be written as

$$\mathbf{a}_1 = R_{\text{exc}}[\cos \psi, \sin \psi]; \quad \mathbf{f}_1 = f^\dagger[\cos \psi, \sin \psi]; \quad (196)$$

$$\mathbf{a}_2 = R_{\text{exc}}[-\sin \psi, \cos \psi]; \quad \mathbf{f}_2 = f^\dagger[\sin \psi, -\cos \psi]; \quad (197)$$

$$\mathbf{a}_3 = -\mathbf{a}_1; \quad \mathbf{f}_3 = -\mathbf{f}_1; \quad (198)$$

$$\mathbf{a}_4 = -\mathbf{a}_2; \quad \mathbf{f}_4 = -\mathbf{f}_2. \quad (199)$$

The dipole tensor for the configuration in Fig. S.3a can be computed as follows

$$P_{ij} \mathbf{e}_i \otimes \mathbf{e}_j = \sum_{q=1}^4 \mathbf{f}_q \otimes \mathbf{a}_q = 2\mathbf{f}_1 \otimes \mathbf{a}_1 + 2\mathbf{f}_2 \otimes \mathbf{a}_2 \quad (200)$$

$$= 2f^\ddagger R_{\text{exc}} \begin{bmatrix} \cos^2 \psi & \cos \psi \sin \psi \\ \cos \psi \sin \psi & \sin^2 \psi \end{bmatrix} + 2f^\ddagger R_{\text{exc}} \begin{bmatrix} -\sin^2 \psi & \cos \psi \sin \psi \\ \cos \psi \sin \psi & -\cos^2 \psi \end{bmatrix} \quad (201)$$

$$= 2f^\ddagger R_{\text{exc}} \begin{bmatrix} \cos 2\psi & \sin 2\psi \\ \sin 2\psi & -\cos 2\psi \end{bmatrix}. \quad (202)$$

Using the definition of the principal components of  $P_{ij}$ , we obtain

$$P_1 = 0; \quad P_2 = -2f^\ddagger R_{\text{exc}} \cos 2\psi; \quad P_3 = 2f^\ddagger R_{\text{exc}} \sin 2\psi. \quad (203)$$

With the dipole tensor computed, we proceed with computing the stresses using Eq. (195):

$$T_1^\ddagger(r, \theta) = f^\ddagger R_{\text{exc}} \left[ \frac{\nu^{\text{IS}} + 1}{\pi r^2} (\cos 2\theta \cos 2\psi + \sin 2\theta \sin 2\psi) \right] \quad (204)$$

$$= f^\ddagger R_{\text{exc}} \frac{\nu^{\text{IS}} + 1}{\pi r^2} \cos(2\theta - 2\psi), \quad (205)$$

$$T_2^\ddagger(r, \theta) = f^\ddagger R_{\text{exc}} \left[ -\frac{3 - \nu^{\text{IS}}}{2} \cos 2\psi \delta(r) + \frac{\nu^{\text{IS}} + 1}{\pi r^2} (\cos 4\theta \cos 2\psi + \sin 4\theta \sin 2\psi) \right] \quad (206)$$

$$= f^\ddagger R_{\text{exc}} \left[ -\frac{3 - \nu^{\text{IS}}}{2} \cos 2\psi \delta(r) + \frac{\nu^{\text{IS}} + 1}{\pi r^2} \cos(4\theta - 2\psi) \right], \quad (207)$$

$$T_3^\ddagger(r, \theta) = f^\ddagger R_{\text{exc}} \left[ \frac{3 - \nu^{\text{IS}}}{2} \sin 2\psi \delta(r) + \frac{\nu^{\text{IS}} + 1}{\pi r^2} (\cos 4\theta \sin 2\psi - \sin 4\theta \cos 2\psi) \right] \quad (208)$$

$$= f^\ddagger R_{\text{exc}} \left[ \frac{3 - \nu^{\text{IS}}}{2} \sin 2\psi \delta(r) - \frac{\nu^{\text{IS}} + 1}{\pi r^2} \sin(4\theta - 2\psi) \right], \quad (209)$$

To compute the TST energy barrier  $\Delta F^\ddagger$ , one must determine the reaction coordinate  $q$ . As discussed in Section V of the main text, we can set  $q$  to be the second principal invariant  $J_2$  of the deviatoric stress tensor  $S_{ij} = T_{ij} - \frac{1}{d}\delta_{ij}T_{kk}$  which is given by

$$J_2 = \frac{1}{2}S_{ij}S_{ij} = \frac{1}{2} \left[ T_{ij}T_{ij} - \frac{1}{d}T_{ii}T_{kk} \right]. \quad (210)$$

The invariant  $J_2$  is proportional to the shear part of the elastic strain energy in Eq. (54), also known as the deviatoric strain energy. To see this, recall from Section 1.1 that the elastic strain energy for inherent states in 2D is given by

$$\Delta F = \int d^2\mathbf{x} \left( \frac{1}{2B^{\text{IS}}} (T_1)^2 + \frac{1}{2G^{\text{IS}}} \left[ (T_2)^2 + (T_3)^2 \right] \right). \quad (211)$$

The term multiplied by  $1/G^{\text{IS}}$  is the deviatoric strain energy denoted by

$$\Delta F_d = \frac{1}{2G^{\text{IS}}} \int d^2\mathbf{x} \left[ (T_2)^2 + (T_3)^2 \right], \quad (212)$$

where the integrand of  $\Delta F_d$  can be written in terms of  $J_2$  by expanding Eq. (210) as

$$J_2 = \frac{1}{2} \left( T_{xx}^2 + T_{yy}^2 + 2T_{xy}^2 - \frac{1}{2} (T_{xx}^2 + T_{yy}^2 + 2T_{xx}T_{yy}) \right) \quad (213)$$

$$= \frac{1}{2} \left( \frac{1}{2} (T_{xx}^2 + T_{yy}^2 - 2T_{xx}T_{yy}) + 2T_{xy}^2 \right) \quad (214)$$

$$= \left( \frac{T_{yy} - T_{xx}}{2} \right)^2 + T_{xy}^2 = (T_2)^2 + (T_3)^2, \quad (215)$$

which implies that  $\Delta F_d = \frac{1}{2G^{\text{IS}}} \int d^2\mathbf{x} J_2$ .

Let us choose the reaction coordinate to be

$$q = \sqrt{\int d^2\mathbf{x} J_2}. \quad (216)$$

Then,  $\Delta F_d$  describes a harmonic 1D energy well for shear deformations

$$\Delta F_d(q) = \frac{1}{2} k q^2 \quad (217)$$

where  $k = 1/G^{\text{IS}}$ . Equation (217) can now be used as a basis for TST calculation. Assuming the transition state corresponds to the dipole configuration in Fig. S.3a, and using the STZ stresses in Eqs. (205), (207) and (209), the transition state value of  $q$  can be computed as

$$q^\ddagger = \sqrt{\int d^2\mathbf{x} (T_2^\ddagger)^2 + (T_3^\ddagger)^2}. \quad (218)$$

If the integration is taken over the full domain, then the integral will diverge due the singularity of the stress. Since deformation is elastic only up to  $R_{\text{exc}}$ , we may use it as a short-distance cut off in Eq. (218) to yield

$$q^\ddagger = \sqrt{\int_{R_{\text{exc}}}^\infty dr r \int_0^{2\pi} d\theta \left( \frac{f^\ddagger R_{\text{exc}} (\nu^{\text{IS}} + 1)}{\pi r^2} \right)^2 [\cos^2(4\theta - 2\psi) + \sin^2(4\theta - 2\psi)]} \quad (219)$$

$$= \frac{f^\ddagger R_{\text{exc}} (\nu^{\text{IS}} + 1)}{\pi} \sqrt{\int_{R_{\text{exc}}}^\infty dr \frac{2\pi}{r^3}} = \frac{f^\ddagger (\nu^{\text{IS}} + 1)}{\sqrt{\pi}}. \quad (220)$$

Setting  $\Delta F^\ddagger \equiv \Delta F_d(q^\ddagger)$  and combining Eq. (220) with Eq. (212), we finally obtain the following expression for the energy barrier

$$\Delta F^\ddagger = \frac{(f^\ddagger)^2 (\nu^{\text{IS}} + 1)^2}{2G^{\text{IS}}\pi}. \quad (221)$$

### 3 Connecting Excitations to Local Structure

The TST energy barrier  $\Delta F^\ddagger$  has one last remaining unknown  $f^\ddagger$ , which is the force magnitude needed to induce a localized inelastic pure shear. A solution for  $f^\ddagger$  comes in three steps:

1. Express  $f^\ddagger$  in terms of the local shear strain experienced inside the STZ, which we will denote as the eigenstrain  $\epsilon_c$ .
2. Paramaterize the local deformation by assuming that the excitation can be modeled as a T1 transition, and express  $\epsilon_c$  in terms of the displacement  $u^\ddagger$  of a particle participating in the T1 transition.
3. Express  $u^\ddagger$  as the minimum displacement needed to break an elastic bond, which is set by the inherent-state radial distribution function (RDF).

The first and second steps are detailed in Section 3.1, and the third step is provided in Section 3.2.

### 3.1 The Eigenstrain and T1 Transition

Although the force magnitude  $f^\ddagger$  dictates the extent of inelastic deformation, it must also be calibrated to the elastic strain at the boundary of the STZ, i.e.,  $r = R_{\text{exc}}$ . Let us denote the local shear strain experienced inside the STZ as the eigenstrain  $\epsilon_c$  and assume it to be uniform. The stress  $T_c$  induced by the eigenstrain  $\epsilon_c$  can be determined by the linear constitutive law in Eq. (41) as  $T_c = 2G^{\text{IS}}\epsilon_c$ . The deviatoric strain energy density  $f_d$  of the STZ can then be written as

$$f_d(r = R_{\text{exc}}) \equiv \frac{1}{2}T_c\epsilon_c = \frac{1}{4G^{\text{IS}}}T_c^2 = G^{\text{IS}}\epsilon_c^2. \quad (222)$$

Note that  $f_d(r = R_{\text{exc}})$  can be computed from the STZ stress profile given by Eqs. (207) and (209),

$$f_d(r = R_{\text{exc}}) = \frac{1}{2G^{\text{IS}}} \left[ \left(T_2^\ddagger\right)^2 + \left(T_3^\ddagger\right)^2 \right] = \frac{(f^\ddagger)^2(1 + \nu^{\text{IS}})^2}{2G^{\text{IS}}\pi^2 R_{\text{exc}}^2} \quad (223)$$

Assuming energy continuity at the interface between the STZ and surroundings, we can equate Eq. (222) with Eq. (223) and obtain an expression for  $f^\ddagger$ ,

$$G^{\text{IS}}\epsilon_c^2 = \frac{(f^\ddagger)^2(1 + \nu^{\text{IS}})^2}{2G^{\text{IS}}\pi^2 R_{\text{exc}}^2} \rightarrow f^\ddagger = \frac{\sqrt{2}\pi R_{\text{exc}} G^{\text{IS}}\epsilon_c}{1 + \nu^{\text{IS}}}. \quad (224)$$

Inserting this to the TST energy barrier formula given in Eq. (221), we obtain

$$\Delta F^\ddagger = \frac{(f^\ddagger)^2(1 + \nu^{\text{IS}})^2}{2G^{\text{IS}}\pi} = G^{\text{IS}}\pi(R_{\text{exc}}\epsilon_c)^2 \quad (225)$$

Alternatively, one may assume that the energy required to deform the STZ is equal to the reorganization energy of the surroundings. This assumption, which is physically plausible, then yields

$$G^{\text{IS}}\epsilon_c^2(\pi R_{\text{exc}}^2) = \Delta F^\ddagger, \quad (226)$$

which is equivalent to Eq. (225).

The size of an excitation  $R_{\text{exc}} \sim O(\sigma)$  and thus, the localized pure shear must be a result of the collective action of very few particles. The simplest candidate for such a pure shear at the particle-scale is a T1 transition. Recall that a T1 transition is an exchange of bonds between four neighboring cells in some tessellated network illustrated in Fig. S.4a. Given some configuration of particles, one can construct a Voronoi network so that a T1 transition proceeds from the concerted motion of four particles shown in Fig. S.4b. Upon triangulation of the particle configuration shown in Fig. S.4c, we see that a T1 transition corresponds to applying a pure shear to a polygonal cell. This cell has an internal bond, which is broken during T1 transition to make room for another bond to form at the final state.

The polygonal cell can be used as a basis for computing  $\epsilon_c$  in terms of particle displacements. To compute the displacement under the T1 transition path, we can parametrize the geometry as shown in Fig. S.5. Let us denote the magnitude of the displacement in node ① to obtain the transition state  $u^\ddagger = |\mathbf{u}_1|$ , so that  $\mathbf{u}_1 = [0, u^\ddagger]^T$ . By symmetry,  $\mathbf{u}_3 = -\mathbf{u}_1$  and  $\mathbf{u}_4 = -\mathbf{u}_2$ . Furthermore,  $\mathbf{u}_2$  is constrained by  $u^\ddagger$ , as node ② must move in such a way that the cell area  $A = \frac{1}{2}\sqrt{3}\sigma^2$  is constant during a pure shear. To determine  $\mathbf{u}_2$  as a function of  $u^\ddagger$ , let us compute the length between nodes ① and ③, denoted as  $\ell_{13}$ , as well as the length between nodes ② and ④, denoted as  $\ell_{24}$ :

$$\ell_{13} = 2 \times \left( \frac{\sigma}{2} + |\mathbf{u}_1| \right) = \sigma + 2u^\ddagger, \quad (227)$$

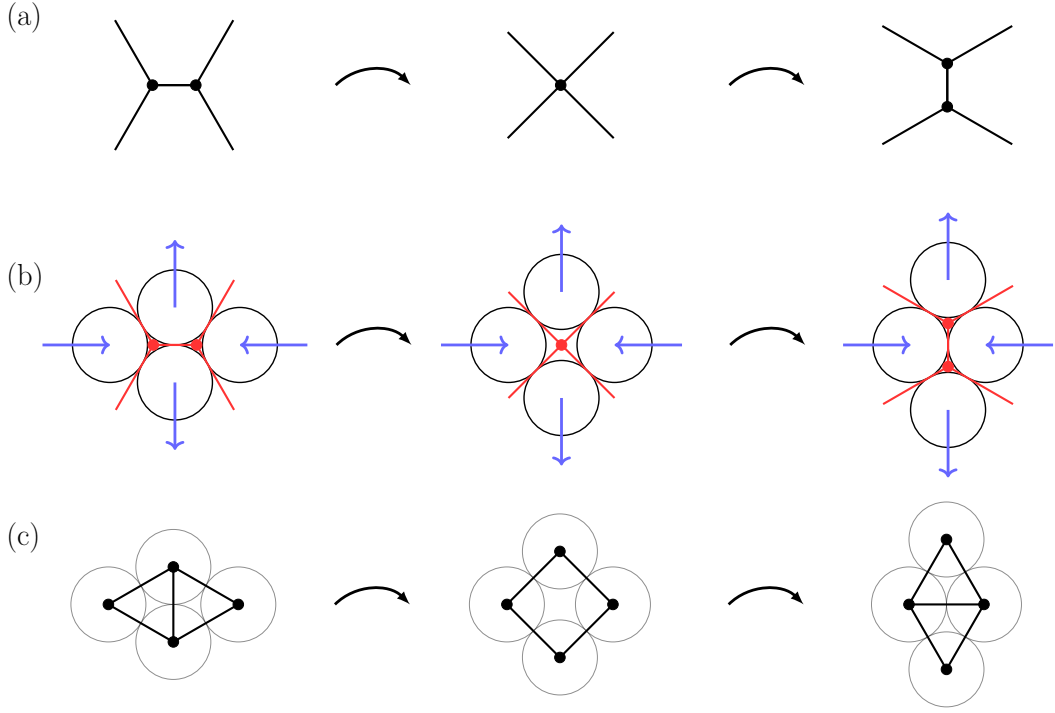

Figure S.4: (a) A T1 transition illustrated by the participating edges that belong to a larger Voronoi network. (b) A four-particle configuration reproducing a T1 transition, overlaid with the edges drawn in (a). Blue arrows are the applied forces, which conform with the force-dipole configuration in Fig. S.3a. (c) The triangulation of the particle configuration. Note that the T1 transition produces a bond-breaking event at its center, followed by a bond-formation event.

$$\ell_{24} = 2 \times \left( \frac{1}{2} \sqrt{3} \sigma - |\mathbf{u}_2| \right) = \sqrt{3} \sigma - 2|\mathbf{u}_2|. \quad (228)$$

In terms of these lengths, the area of the cell is  $A = \frac{1}{2} \ell_{24} \ell_{13}$  which, upon combining it with the cell area  $A = \frac{1}{2} \sqrt{3} \sigma^2$ , gives us an equation to solve for the magnitude of  $\mathbf{u}_2$ :

$$\frac{1}{2} \sqrt{3} \sigma^2 = \frac{1}{2} (\sqrt{3} \sigma - 2|\mathbf{u}_2|) (\sigma + 2u^\dagger) \quad (229)$$

$$\Rightarrow \frac{|\mathbf{u}_2|}{\sigma} = \frac{\sqrt{3}}{2} \left( 1 - \frac{1}{1 + 2u^\dagger/\sigma} \right) = \frac{\sqrt{3} u^\dagger/\sigma}{1 + 2u^\dagger/\sigma}. \quad (230)$$

In summary, the displacements of all four nodes are now given by

$$\mathbf{u}_1 = [0, u^\dagger]^T; \quad \mathbf{u}_2 = \left[ \frac{\sqrt{3} u^\dagger}{1 + 2u^\dagger/\sigma}, 0 \right]^T; \quad \mathbf{u}_3 = -\mathbf{u}_1; \quad \mathbf{u}_4 = -\mathbf{u}_2 \quad (231)$$

Next, a formula for  $\epsilon_c$  is derived as a function of  $u^\dagger$ . Recall that computing strain requires continuous displacement fields but we only have discrete node variables. Despite the discrete nature, a spatially-averaged strain can still be computed through Gauss' theorem:

$$\bar{\epsilon}_{ij} = \frac{1}{V} \int d^d \mathbf{x} \epsilon_{ij} = \frac{1}{2V} \int d^d \mathbf{x} (u_{i,j} + u_{j,i}) = \frac{1}{2V} \int dS (u_i n_j + u_j n_i) \quad (232)$$

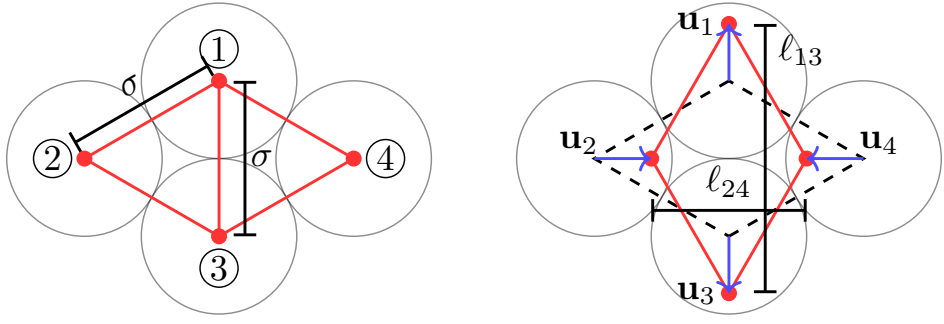

Figure S.5: The geometry of the T1 transition both at rest (left) and during deformation (right).

where the third equality can be discretized according to the cell geometry in Fig. S.5. This provides a formula assigning a unique strain value to the entire cell, i.e.,

$$\bar{\epsilon}_{ij} \mathbf{e}_i \otimes \mathbf{e}_j \approx \frac{\sigma}{2A} \sum_{k=1}^4 [\langle \mathbf{u} \rangle_k \otimes \mathbf{n}_k + \mathbf{n}_k \otimes \langle \mathbf{u} \rangle_k] \quad (233)$$

where  $k$  denotes the index of the  $k$ -th outer edge of the cell. Here,  $\mathbf{n}_k$  is the normal vector of the  $k$ -th edge, and  $\langle \mathbf{u} \rangle_k$  is the average displacement of the  $k$ -th edge, as computed from the displacement at the two nodes given by

$$\langle \mathbf{u} \rangle_1 = \frac{1}{2} (\mathbf{u}_1 + \mathbf{u}_2) = \left[ \frac{\sqrt{3}u^\dagger}{2(1+2u^\dagger/\sigma)}, \frac{u^\dagger}{2} \right]^T; \quad \mathbf{n}_1 = \frac{\left[ -\frac{\sigma}{2}, \frac{\sqrt{3}\sigma}{2} \right]^T}{\sqrt{(\frac{\sigma}{2})^2 + (\frac{\sqrt{3}\sigma}{2})^2}} = \left[ -1/2, \sqrt{3}/2 \right]^T, \quad (234)$$

$$\langle \mathbf{u} \rangle_2 = \frac{1}{2} (\mathbf{u}_2 + \mathbf{u}_3) = \frac{1}{2} (\mathbf{u}_2 - \mathbf{u}_1) = \left[ \frac{\sqrt{3}u^\dagger}{2(1+2u^\dagger/\sigma)}, -\frac{u^\dagger}{2} \right]^T; \quad \mathbf{n}_2 = \left[ -1/2, -\sqrt{3}/2 \right]^T, \quad (235)$$

$$\langle \mathbf{u} \rangle_3 = \frac{1}{2} (\mathbf{u}_3 + \mathbf{u}_4) = -\frac{1}{2} (\mathbf{u}_1 + \mathbf{u}_2) = -\langle \mathbf{u} \rangle_1; \quad \mathbf{n}_3 = -\mathbf{n}_1, \quad (236)$$

$$\langle \mathbf{u} \rangle_4 = \frac{1}{2} (\mathbf{u}_4 + \mathbf{u}_1) = -\frac{1}{2} (\mathbf{u}_2 - \mathbf{u}_1) = -\langle \mathbf{u} \rangle_2; \quad \mathbf{n}_4 = -\mathbf{n}_2. \quad (237)$$

Using Eqs. (234) to (237), the spatially-averaged strain can be obtained as

$$\bar{\epsilon}_{ij} \mathbf{e}_i \otimes \mathbf{e}_j = \begin{bmatrix} -\frac{2u^\dagger/\sigma}{1+2u^\dagger/\sigma} & 0 \\ 0 & \frac{2u^\dagger}{\sigma} \end{bmatrix}. \quad (238)$$

The eigenstrain  $\epsilon_c$  can be computed from  $\bar{\epsilon}_{ij}$  by noting from Eq. (52) that the deviatoric strain energy density  $f_d$  can also be written in terms of all strain components, i.e.,

$$f_d = G^{\text{IS}} \left( \frac{1}{2} (\epsilon_{yy} - \epsilon_{xx})^2 + 2\epsilon_{xy}^2 \right). \quad (239)$$

Combining this with Eq. (222), we obtain a new expression for  $\epsilon_c$ :

$$\epsilon_c = \sqrt{\frac{1}{2} (\bar{\epsilon}_{yy} - \bar{\epsilon}_{xx})^2 + 2\bar{\epsilon}_{xy}^2} = \sqrt{\frac{1}{2} \left( \frac{4(1+u^\dagger/\sigma)u^\dagger/\sigma}{1+2u^\dagger/\sigma} \right)^2} \quad (240)$$

$$= 2\sqrt{2} \frac{(1 + u^\ddagger/\sigma)u^\ddagger/\sigma}{1 + 2u^\ddagger/\sigma}. \quad (241)$$

Letting  $u^\ddagger/\sigma = \tilde{u}^\ddagger$  to be the dimensionless displacement, the energy barrier in Eq. (225) becomes

$$\Delta F^\ddagger = G^{\text{IS}} \pi (R_{\text{exc}} \epsilon_c)^2 = 8G^{\text{IS}} \pi R_{\text{exc}}^2 \frac{(1 + \tilde{u}^\ddagger)^2 (\tilde{u}^\ddagger)^2}{(1 + 2\tilde{u}^\ddagger)^2}. \quad (242)$$

To compute  $R_{\text{exc}}$ , recall that  $R_{\text{exc}}$  must encompass the entire T1 transition region during deformation. For this purpose, its value can be set to either  $\ell_{13}$  or  $\ell_{24}$ . If the transition state is reached prior to the bond-breaking event between nodes ① and ③ then  $\ell_{13} < \ell_{24}$  and thus,  $\ell_{24}$  can be used to compute  $R_{\text{exc}}$  as follows,

$$R_{\text{exc}} \equiv \frac{\ell_{24}}{2} = \frac{1}{2} \sqrt{3} \sigma - |\mathbf{u}_2| = \frac{1}{2} \sqrt{3} \sigma \left( 1 - \frac{2u^\ddagger/\sigma}{1 + 2u^\ddagger/\sigma} \right) = \frac{\sqrt{3} \sigma}{2(1 + 2\tilde{u}^\ddagger)}. \quad (243)$$

This also implies that there exists an upper theoretical limit  $u_{\text{max}}^\ddagger$  set by the condition  $\ell_{13} = \ell_{24}$ . Upon solving this for  $u_{\text{max}}^\ddagger$ , we obtain

$$u_{\text{max}}^\ddagger = \frac{1}{2} \sigma (-1 + 3^{1/4}) \approx 0.158 \sigma. \quad (244)$$

This theoretical limit will be useful when discussing the limitations of the T1 transition state model. Combining this with Eq. (242), we obtain

$$\Delta F^\ddagger = 6\pi G^{\text{IS}} \sigma^2 \frac{(\tilde{u}^\ddagger)^2 (1 + \tilde{u}^\ddagger)^2}{(1 + 2\tilde{u}^\ddagger)^4}. \quad (245)$$

### 3.2 Determining $u^\ddagger$ from Radial Distribution Functions

The scalar variable  $u^\ddagger$  sets the amount of displacement experienced by the bond-breaking particles. These bonds can be determined by the radial distribution function  $g(r)$  (RDF), since a bond-breaking event corresponds to re-organization of the first solvation shell. From the RDF, one may also compute the potential of mean force (PMF)  $w(r) = -k_B T \ln g(r)$ , which sets both the equilibrium length and stretching limit of an elastic bond. However, most glass formers are multi-component systems and there exist as many RDFs as pairs of distinguishable particles. A question arises as to how does one average these RDFs to obtain a PMF consistent with an equivalent single-component picture of the T1 transition?

To answer this question, let us first investigate how RDFs enter into the thermodynamic properties, such as the virial pressure. If a consistently averaged RDF exists, then it should be one that can compute the virial pressure of a multi-component system. Furthermore, the formula should resemble the RDF integration formulas that one would find in single-component systems [9]. In light of the continuous poly-disperse systems studied in this work, let us write the potential energy as

$$U = \sum_{\alpha, \beta} \phi(r^{\alpha\beta} / \sigma_{\alpha\beta}) \quad (246)$$

where  $\sigma_{\alpha\beta}$  sets the microscopic length-scale of pair interactions and is computable from the average diameter between  $\alpha$ -th and  $\beta$ -th particle. The virial pressure in  $d$ -dimensions, from the Irving-Kirkwood procedure [10] is given by

$$P = \frac{1}{dV} \left\langle \sum_{\alpha, \beta} \mathbf{F}^{\alpha\beta} \cdot \mathbf{r}^{\alpha\beta} \right\rangle = -\frac{1}{dV} \left\langle \sum_{\alpha, \beta} \phi_r^{\alpha\beta} r^{\alpha\beta} \right\rangle = -\frac{1}{dV} \sum_{\alpha, \beta} \left\langle \phi_r^{\alpha\beta} r^{\alpha\beta} \right\rangle \quad (247)$$

$$= -\frac{1}{dV} \sum_{\alpha,\beta} \int d^d \mathbf{r}^\alpha \int d^d \mathbf{r}^\beta \int \prod_{\kappa \neq \alpha,\beta} d^d \mathbf{r}^\kappa \phi_r^{\alpha\beta} r^{\alpha\beta} \rho(\mathbf{r}^\alpha, \mathbf{r}^\beta, \{\mathbf{r}^\kappa\}_{\kappa \neq \alpha,\beta}). \quad (248)$$

where  $\phi_r^{\alpha\beta} = \phi_r(r^{\alpha\beta}/\sigma_{\alpha\beta})$  and in the second line, the ensemble average is expanded and the integration on  $\mathbf{r}^\alpha$  and  $\mathbf{r}^\beta$  variables are separated out.

Equation (248) can be further simplified using the partial pair distribution function  $g_{\alpha\beta}(\mathbf{x}, \mathbf{x}')$ , which is derived for a continuous poly-disperse system from the definition of  $g_{\alpha\beta}(\mathbf{x}, \mathbf{x}')$  for a multi-component system,

$$g_{\alpha\beta}(\mathbf{x}, \mathbf{x}') \equiv \frac{N_\alpha N_\beta}{\rho_\alpha \rho_\beta} \langle \delta(\mathbf{x} - \mathbf{r}^\alpha) \delta(\mathbf{x}' - \mathbf{r}^\beta) \rangle \quad (249)$$

where  $\alpha$  and  $\beta$  denote the  $\alpha$ -th and  $\beta$ -th component,  $N_\alpha$  is the number of particles in the  $\alpha$ -th component and  $\rho_\alpha$  is the corresponding number density. In a continuous poly-disperse system, every particle is its own chemical species ( $N_\alpha = 1, \rho_\alpha = 1/V$ ) and thus,

$$g_{\alpha\beta}(\mathbf{x}, \mathbf{x}') = V^2 \langle \delta(\mathbf{x} - \mathbf{r}^\alpha) \delta(\mathbf{x}' - \mathbf{r}^\beta) \rangle, \quad (250)$$

and the ensemble average of the delta functions are given by

$$\langle \delta(\mathbf{x} - \mathbf{r}^\alpha) \delta(\mathbf{x}' - \mathbf{r}^\beta) \rangle = \int \prod_{\kappa=1}^N d^d \mathbf{r}^\kappa \rho(\{\mathbf{r}^\kappa\}) \delta(\mathbf{x} - \mathbf{r}^\alpha) \delta(\mathbf{x}' - \mathbf{r}^\beta) \quad (251)$$

$$= \int d^d \mathbf{r}^\alpha \int d^d \mathbf{r}^\beta \int \prod_{\kappa \neq \alpha,\beta} d^d \mathbf{r}^\kappa \rho(\mathbf{r}^\alpha, \mathbf{r}^\beta, \{\mathbf{r}^\kappa\}_{\kappa \neq \alpha,\beta}) \delta(\mathbf{x} - \mathbf{r}^\alpha) \delta(\mathbf{x}' - \mathbf{r}^\beta). \quad (252)$$

Note that the delta functions are defined so that  $\int d^d \mathbf{r}^\alpha \delta(\mathbf{x} - \mathbf{r}^\alpha) f(\mathbf{r}^\alpha) = f(\mathbf{x})$  and  $\int d^d \mathbf{r}^\beta \delta(\mathbf{x}' - \mathbf{r}^\beta) f(\mathbf{r}^\beta) = f(\mathbf{x}')$  for any arbitrary function  $f$ , simplifying the last line into

$$\langle \delta(\mathbf{x} - \mathbf{r}^\alpha) \delta(\mathbf{x}' - \mathbf{r}^\beta) \rangle = \int \prod_{\kappa \neq \alpha,\beta} d^d \mathbf{r}^\kappa \rho(\mathbf{x}, \mathbf{x}', \{\mathbf{r}^\kappa\}_{\kappa \neq \alpha,\beta}). \quad (253)$$

One could see that Eq. (253) enters into Eq. (248) if  $\mathbf{r}^\alpha$  and  $\mathbf{r}^\beta$  variables were exchanged with  $\mathbf{x}$  and  $\mathbf{x}'$ . This change of variables is possible because  $\mathbf{r}^\alpha$  and  $\mathbf{r}^\beta$  act as dummy integrating variables. Thus, upon switching  $\mathbf{r}^\alpha \rightarrow \mathbf{x}$  and  $\mathbf{r}^\beta \rightarrow \mathbf{x}'$  in Eq. (248), we have  $r^{\alpha\beta} = |\mathbf{x} - \mathbf{x}'|$ , and

$$\phi_r^{\alpha\beta} = \frac{d\phi(r^{\alpha\beta}/\sigma_{\alpha\beta})}{dr} = \frac{d\phi(|\mathbf{x} - \mathbf{x}'|/\sigma_{\alpha\beta})}{dr} \equiv \phi_r(|\mathbf{x} - \mathbf{x}'|/\sigma_{\alpha\beta}), \quad (254)$$

which then reduces Eq. (248) to

$$P = -\frac{1}{dV} \sum_{\alpha,\beta} \int d^d \mathbf{x} \int d^d \mathbf{x}' \int \prod_{\kappa \neq \alpha,\beta} d^d \mathbf{r}^\kappa \phi_r(|\mathbf{x} - \mathbf{x}'|/\sigma_{\alpha\beta}) |\mathbf{x} - \mathbf{x}'| \rho(\mathbf{x}, \mathbf{x}', \{\mathbf{r}^\kappa\}_{\kappa \neq \alpha,\beta}) \quad (255)$$

$$= -\frac{1}{dV} \sum_{\alpha,\beta} \int d^d \mathbf{x} \int d^d \mathbf{x}' \phi_r(|\mathbf{x} - \mathbf{x}'|/\sigma_{\alpha\beta}) |\mathbf{x} - \mathbf{x}'| \frac{1}{V^2} g_{\alpha\beta}(\mathbf{x}, \mathbf{x}'). \quad (256)$$

Let us make an additional change of variables into  $\mathbf{r} = \mathbf{x} - \mathbf{x}'$  and  $\mathbf{R} = \frac{1}{2}(\mathbf{x} + \mathbf{x}')$ . The determinant of this mapping's Jacobian is unity so that the integration element  $d^d \mathbf{x} d^d \mathbf{x}' = d^d \mathbf{r} d^d \mathbf{R}$ , which further reduces Eq. (256) to

$$P = -\frac{1}{dV} \sum_{\alpha,\beta} \int d^d \mathbf{r} \int d^d \mathbf{R} \phi_r(r/\sigma_{\alpha\beta}) r \frac{g_{\alpha\beta}(\mathbf{r}, \mathbf{R})}{V^2} \quad (257)$$

$$= -\frac{1}{dV^2} \sum_{\alpha,\beta} \int d^d \mathbf{r} \, r \phi_r(r/\sigma_{\alpha\beta}) \left[ \frac{1}{V} \int d^d \mathbf{R} \, g_{\alpha\beta}(\mathbf{r}, \mathbf{R}) \right] \quad (258)$$

where  $r = |\mathbf{r}|$ . Letting  $g_{\alpha\beta}(\mathbf{r}) \equiv \frac{1}{V} \int d^d \mathbf{R} \, g_{\alpha\beta}(\mathbf{r}, \mathbf{R})$ , the virial pressure becomes

$$P = -\frac{1}{dV^2} \sum_{\alpha,\beta} \int d^d \mathbf{r} \, r \phi_r(r/\sigma_{\alpha\beta}) g_{\alpha\beta}(\mathbf{r}). \quad (259)$$

In 2D, one may use the polar coordinates and express the partial RDF as the angular average of  $g_{\alpha\beta}(\mathbf{r}) = g_{\alpha\beta}(r, \theta)$ , i.e.,

$$g_{\alpha\beta}(r) = \frac{1}{2\pi} \int_0^{2\pi} d\theta \, g_{\alpha\beta}(r, \theta), \quad (260)$$

which reduces Eq. (259) to

$$P = -\frac{1}{2V^2} \sum_{\alpha,\beta} \int_0^\infty dr \int_0^{2\pi} d\theta \, r^2 \phi_r(r/\sigma_{\alpha\beta}) g_{\alpha\beta}(r, \theta) \quad (261)$$

$$= -\frac{1}{2V^2} \sum_{\alpha,\beta} \int_0^\infty dr \, r^2 \phi_r(r/\sigma_{\alpha\beta}) 2\pi \left[ \frac{1}{2\pi} \int_0^{2\pi} d\theta g_{\alpha\beta}(r, \theta) \right] \quad (262)$$

$$= -\frac{\pi}{V^2} \sum_{\alpha,\beta} \int_0^\infty dr \, r^2 \phi_r(r/\sigma_{\alpha\beta}) g_{\alpha\beta}(r). \quad (263)$$

At this stage, the pair potential is still dependent on the details of the  $\alpha$ -th and  $\beta$ -th particle through  $\sigma_{\alpha\beta}$ . To eliminate it, choosing  $\tilde{r} = r/\sigma_{\alpha\beta}$ , the pair potential can be non-dimensionalized as

$$\phi_r(r/\sigma_{\alpha\beta}) = \frac{d\tilde{r}}{dr} \frac{d\phi(\tilde{r})}{d\tilde{r}} = \frac{1}{\sigma_{\alpha\beta}} \phi_{\tilde{r}}(\tilde{r}). \quad (264)$$

The partial RDF can be non-dimensionalized once the pair distance  $r^{\alpha\beta}$  entering the delta function is also non-dimensionalized

$$g_{\alpha\beta}(r) = \frac{1}{2\pi} \int_0^{2\pi} d\theta \frac{1}{V} \int d\mathbf{R} \, g_{\alpha\beta}(\mathbf{r}, \mathbf{R}) = \frac{V}{2\pi r} \langle \delta(r - r^{\alpha\beta}) \rangle = \frac{V}{2\pi \sigma_{\alpha\beta} \tilde{r}} \langle \delta(\sigma_{\alpha\beta}(\tilde{r} - \tilde{r}^{\alpha\beta})) \rangle \quad (265)$$

$$= \frac{1}{(\sigma_{\alpha\beta})^2} \frac{V}{2\pi \tilde{r}} \langle \delta(\tilde{r} - \tilde{r}^{\alpha\beta}) \rangle = \frac{1}{(\sigma_{\alpha\beta})^2} \tilde{g}_{\alpha\beta}(\tilde{r}) \quad (266)$$

where  $\tilde{g}_{\alpha\beta}(\tilde{r})$  is the partial RDFs computed from the dimensionless pair distance  $\tilde{r}^{\alpha\beta} = r^{\alpha\beta}/\sigma_{\alpha\beta}$ . Substituting Eq. (264) and Eq. (266) into Eq. (263),

$$P = -\frac{\pi}{V^2} \sum_{\alpha,\beta} \int_0^\infty dr \, r^2 \frac{1}{(\sigma_{\alpha\beta})^3} \phi_{\tilde{r}}(\tilde{r}) \tilde{g}_{\alpha\beta}(\tilde{r}) = -\frac{\pi}{V^2} \int_0^\infty d\tilde{r} \, \tilde{r}^2 \phi_{\tilde{r}}(\tilde{r}) \sum_{\alpha,\beta} \tilde{g}_{\alpha\beta}(\tilde{r}). \quad (267)$$

Defining an averaged RDF as

$$\tilde{g}(\tilde{r}) \equiv \frac{1}{N(N-1)/2} \sum_{\alpha,\beta} \tilde{g}_{\alpha\beta}(\tilde{r}) \quad (268)$$

and substituting it into Eq. (267), we arrive at a formula for the virial pressure of a poly-disperse system that resembles the formula for a mono-disperse system:

$$P = -\frac{\pi N(N-1)}{2V^2} \int_0^\infty d\tilde{r} \, \tilde{r}^2 \phi_{\tilde{r}}(\tilde{r}) \tilde{g}(\tilde{r}) \approx -\frac{\pi \rho^2}{2} \int_0^\infty d\tilde{r} \, \tilde{r}^2 \phi_{\tilde{r}}(\tilde{r}) \tilde{g}(\tilde{r}) \quad (269)$$

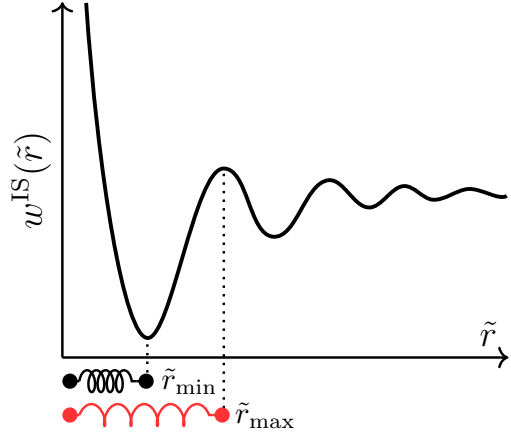

Figure S.6: An illustration of the inherent-state potential of mean force (PMF)  $w^{\text{IS}}(\tilde{r}) = -k_{\text{B}}T \ln g(\tilde{r})$  and the elastic bond at equilibrium (black) and onset of bond-breaking event (red).

where the approximation  $N(N-1) \approx N^2$  for large  $N$  is used in the second equality.

Note that this derivation works without prior assumptions about the distribution and thus, it can be used to compute virial pressure of inherent states sampled at thermal equilibrium,

$$P^{\text{IS}} \approx -\frac{\pi\rho^2}{2} \int_0^\infty d\tilde{r} \tilde{r}^2 \phi_{\tilde{r}}(\tilde{r}) \tilde{g}^{\text{IS}}(\tilde{r}). \quad (270)$$

where  $\tilde{g}^{\text{IS}}(\tilde{r})$  is computed from binning the dimensionless pair distances  $\tilde{R}^{\alpha\beta} \equiv R^{\alpha\beta}/\sigma_{\alpha\beta}$  obtained from sampled inherent states. Since  $\tilde{g}^{\text{IS}}(\tilde{r})$  gives the consistent averaged picture of the local structure, we can use its corresponding PMF, denoted as  $\tilde{w}^{\text{IS}}(\tilde{r}) \equiv -k_{\text{B}}T \ln \tilde{g}^{\text{IS}}(\tilde{r})$ , to compute  $\tilde{u}^\ddagger$ . As illustrated in Fig. S.6, the location of the first minimum  $\tilde{r}_{\text{min}}$  sets the average pair contact distance between two particles, which implies that  $\sigma \equiv \langle \sigma \rangle \tilde{r}_{\text{min}}$ . To break an elastic bond, the particle in the first energy well must be moved to the nearest saddle point located at  $\tilde{r}_{\text{max}}$ , which implies that

$$\tilde{u}^\ddagger = \frac{1}{2}(\tilde{r}_{\text{max}} - \tilde{r}_{\text{min}}) \quad (271)$$

where the factor of  $1/2$  exists because  $u^\ddagger$  is measured from the center of the elastic bond throughout the deformation.

Using Eq. (271), the final formula for  $\Delta F^\ddagger$  can be summarized as follows

$$\Delta F^\ddagger = 6\pi G^{\text{IS}} \sigma^2 \frac{(\tilde{u}^\ddagger)^2 (1 + \tilde{u}^\ddagger)^2}{(1 + 2\tilde{u}^\ddagger)^4}; \quad \tilde{u}^\ddagger = \frac{1}{2}(\tilde{r}_{\text{max}} - \tilde{r}_{\text{min}}); \quad (272)$$

As discussed in Section V of the main text, the excitation energy barrier  $J_\sigma$  corresponds to the the zero-temperature limit of  $\Delta F^\ddagger$ , leading to

$$J_\sigma = \lim_{T \rightarrow 0} \left[ 6\pi G^{\text{IS}} \sigma^2 \frac{(\tilde{u}^\ddagger)^2 (1 + \tilde{u}^\ddagger)^2}{(1 + 2\tilde{u}^\ddagger)^4} \right] \quad (273)$$

where temperature dependence arises from both  $G^{\text{IS}} = G^{\text{IS}}(T)$ ,  $\tilde{u}^\ddagger = \tilde{u}^\ddagger(T)$ , and  $\sigma = \langle \sigma \rangle \tilde{r}_{\text{min}}(T)$ . Recall also from Section V of the main text that  $\Delta F^\ddagger$  must be at most linear in temperature. Since local structure changes very little with respect to temperature, the linearity of  $\Delta F^\ddagger$  should arise mostly from  $G^{\text{IS}}$ . This linearity of  $G^{\text{IS}}$  with respect to temperature is verified in Section 4.

Table 1: List of poly-disperse models studied in this work. A model with repulsive-interaction exponent  $m$  and interactive-interaction  $n$  is named Poly- $(m, n)$ .

| Model       | $m$ | $n$ | $\varepsilon$ | $\tilde{r}_c$ |
|-------------|-----|-----|---------------|---------------|
| Poly-(12,0) | 12  | 0   | 0.2           | 1.25          |
| Poly-(12,6) | 12  | 6   | 0.2           | 2.5           |
| Poly-(18,0) | 18  | 0   | 0.0           | 1.25          |
|             | 18  | 0   | 0.2           | 1.25          |
| Poly-(10,6) | 10  | 6   | 0.1           | 2.5           |
|             | 10  | 6   | 0.2           | 2.5           |

## 4 Testing the Theory and Computational Methods

The theory presented in the main text and the prediction for  $J_\sigma$  is tested against one from DF theory analysis [1] on a class of continuous poly-disperse systems studied in [11], where the pair potential is given by

$$\phi(r/\sigma_{\alpha\beta}) = \begin{cases} v_0 \left[ \left( \frac{\sigma_{\alpha\beta}}{r} \right)^m - \left( \frac{\sigma_{\alpha\beta}}{r} \right)^n \right] + F(r/\sigma_{\alpha\beta}) & r/\sigma_{\alpha\beta} \leq \tilde{r}_c \\ 0 & \text{otherwise} \end{cases}, \quad (274)$$

$$\sigma_{\alpha\beta} = \frac{1}{2} (\sigma_\alpha + \sigma_\beta) (1 - \varepsilon |\sigma_\alpha - \sigma_\beta|), \quad (275)$$

the function  $F(r) = c_0 + c_1 r^2 + c_2 r^4$  is an even polynomial that ensures continuity of the pair potential at  $r = \tilde{r}_c$  up to second-order derivative, and  $\varepsilon$  is the non-additive parameter. The particle size distribution is given by a power law  $P(\sigma) = C/\sigma^3$  for  $\sigma_{\min} < \sigma < \sigma_{\max}$  and zero otherwise, where  $C$  is some normalizing constant.

As listed in Table 1, six poly-disperse systems were chosen by varying  $m$ ,  $n$ ,  $\varepsilon$ , and  $\tilde{r}_c$ . The rest of the model parameters are standardized:  $v_0 = 1$ ,  $\sigma_{\min}$ ,  $\sigma_{\max}$  and  $C$  are chosen so that  $\langle \sigma \rangle = \int d\sigma P(\sigma) \sigma = 1$  and  $\sigma_{\min}/\sigma_{\max} = 0.45$ , mass is unity,  $k_B = 1$ , density  $\rho = 1.01$ , and system size is  $N = 32^2$  particles. All computations are reported in reduced units of mass  $m^* = 1$ , length  $\sigma^* = \langle \sigma \rangle = 1$ , and energy  $\varepsilon^* = v_0 = 1$ . The computational workflow for testing our theory is as follows:

1. *Swap Monte Carlo (MC) Simulation*: poly-disperse models are equilibrated to extremely low temperatures using a parallel version of swap MC algorithm [11], implemented in HOOMD-blue's hard-particle Monte Carlo (HPMC) code [12].
2. *Inherent-State Sampling*: from equilibrated configurations  $\{\mathbf{r}_\alpha\}$ , inherent-state configurations  $\{\mathbf{R}_\alpha\}$  were obtained by local energy minimizations.
3. *Shear Modulus Calculation*: for every inherent state, its shear modulus is computed according to Eq. (121), with the non-affine part computed using a parallel eigensolver SLEPc [13].
4. *Inherent-State RDF Calculation*:  $\tilde{g}^{\text{IS}}(\tilde{r})$  is computed from binning dimensionless inherent-state pair distances  $\tilde{R}^{\alpha\beta} = R^{\alpha\beta}/\sigma_{\alpha\beta}$ . We also confirm the validity of the virial pressure formula in Eq. (270). After completing steps 3 and 4, we compute  $\Delta F^\ddagger(T)$  using Eq. (272) and estimate  $J_\sigma$  from extrapolating  $\Delta F^\ddagger(T)$  to its zero-temperature value.
5. *MD Simulations and  $\tau_{\text{eq}}$  Calculation*: the same poly-disperse models are then equilibrated with MD NVT simulation. Subsequent NVE runs were then used to compute  $\tau_{\text{eq}}$  from the

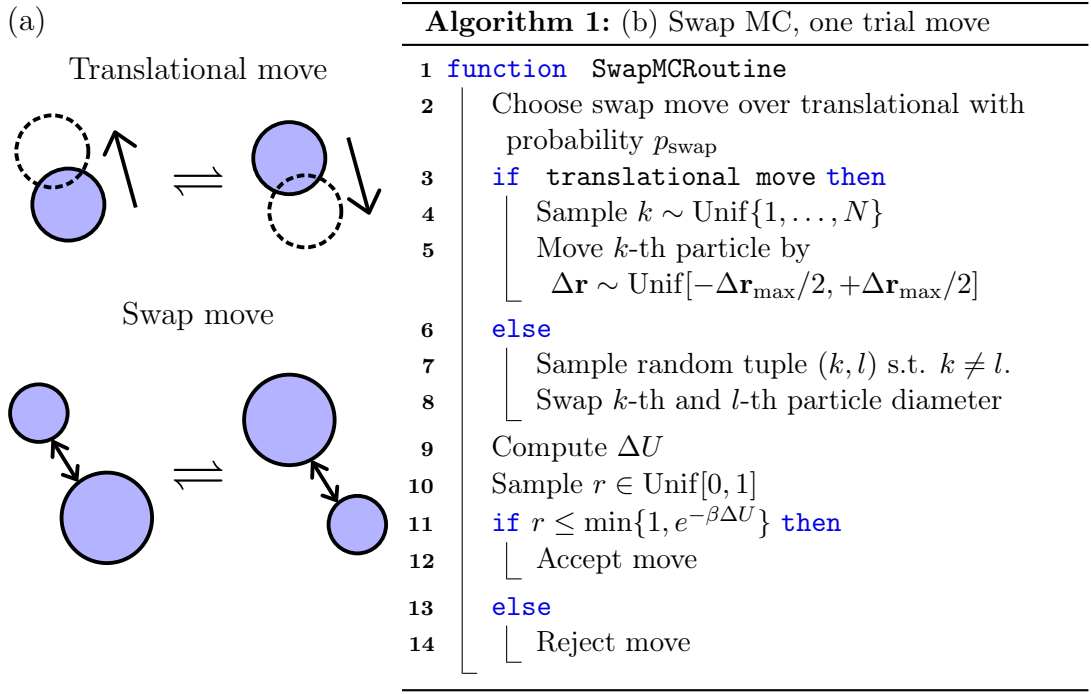

Figure S.7: (a) Illustration of translational move vs. swap move. Note that swap move can be interpreted as swapping diameter or position. (b) Pythonic pseudo-code for swap MC, following [11].

self-part of the intermediate scattering function  $F_s(\mathbf{k}, t)$  at temperatures below and above onset temperature  $T_0$ .

6. *DF Theory Trajectory Analysis*: a select range of temperatures below  $T_0$  is used to generate short-time trajectories. Following the procedure in [1], we compute  $J_\sigma$  independently by DF theory analysis, and compare it against our theory.

Relevant benchmark results and details of each step will be presented below.

#### 4.1 Swap Monte Carlo Simulation

Swap MC is a Metropolis-Hastings MC algorithm, whose trial moves are split between translational and swap moves, where each move is illustrated in Fig. S.7a. Adding swap moves allows us to equilibrate the poly-disperse systems we study to extremely low temperatures [11], making swap MC suitable for our theory. The pseudo-code for one trial move can be written as in Fig. S.7b. In this work, a parallelized version is implemented, following HOOMD-blue’s domain decomposition scheme [12], which is a simpler variant of the checkerboard scheme applied in [14]. As illustrated in Fig. S.7c, the system is broken into  $N_{\text{cell}}$ -many cells called active domains. In a multi-CPU simulation, each active domain is held by one CPU process, and swap MC proceeds normally with the added constraint that translational moves are always rejected if they bring particles outside of the active domain. After one Monte Carlo sweep (MCS), the cells’ position are randomly shifted by  $d_{\text{max}}$  to allow moves inside the inactive domain.

The pseudo-code for the parallel swap MC is given in Fig. S.8, with its details varying depending on choice of neighbor list and parallelization scheme, i.e., multi-CPU vs. GPUs. In this work, we

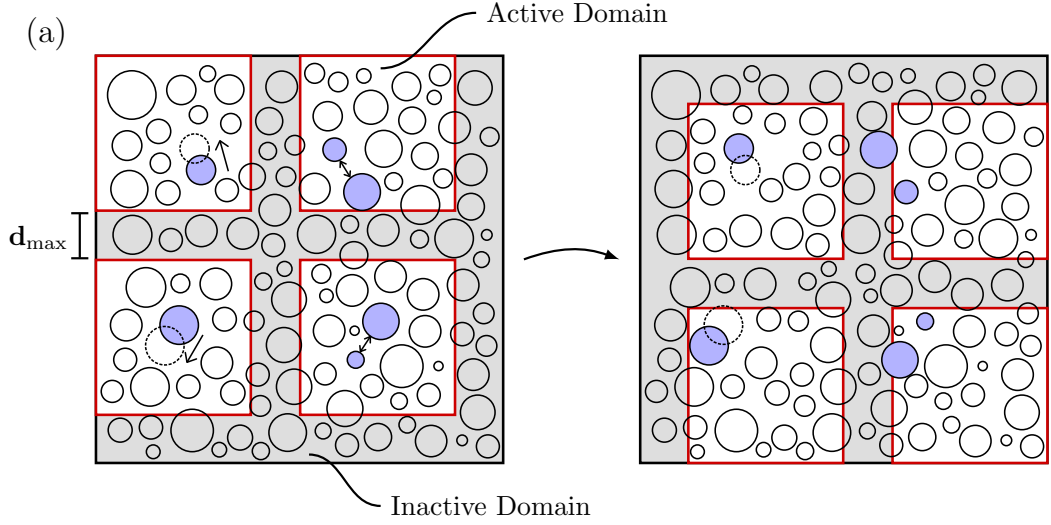


---

**Algorithm 2:** (b) Swap MC in parallel for one Monte Carlo Sweep (MCS).

---

```

1 function ParallelSwapMC
2   for  $\alpha = \{1, \dots, N_{\text{cell}}\}$  in parallel do
3     ShuffledOrder  $\leftarrow$  List of shuffled particle order  $\{1, \dots, N(\alpha)\}$ 
4     for  $i \in \text{ShuffledOrder}$  do
5       Choose swap move over translational with probability  $p_{\text{swap}}$ 
6       if translational move then
7         Move  $i$ -th particle by  $\Delta \mathbf{r} \sim \text{Unif}[-\Delta \mathbf{r}_{\max}/2, +\Delta \mathbf{r}_{\max}/2]$ 
8         if  $\mathbf{r}_i$  is outside of  $\alpha$ -th cell then
9           Reject move
10          continue
11        else
12          Sample  $j \sim \text{Unif}\{1, \dots, i-1, i+1, \dots, N(\alpha)\}$ 
13          Swap  $i$ -th and  $j$ -th particle diameter (or position)
14        Compute  $\Delta U$ 
15        Sample  $r \sim \text{Unif}[0, 1]$ 
16        if  $r \leq \min\{1, e^{-\beta \Delta U}\}$  then
17          Accept move
18        else
19          Reject move
20      Move and update cell center position by  $\Delta \mathbf{r} \sim \text{Unif}[-\mathbf{d}_{\max}/2, +\mathbf{d}_{\max}/2]$ 
21      Update particles assignment to their new cells.

```

---

Figure S.8: (a) An illustration of parallel swap MC on four active domains. Note that no moves can proceed in the inactive domain and cells' overall position is randomly shifted up to  $\mathbf{d}_{\max}$  prior to the next sweep. (b) Pythonic pseudo-code for parallel swap MC. The primary difference between `ParallelSwapMC` and HOOMD-blue's HPMC code is in Line 11-13, where a new swap move is added. Note that Line 20 and 21 requires the collective communication between  $N_{\text{cell}}$ -many processes and energy computation in Line 14 is contingent upon choice of neighbor list.

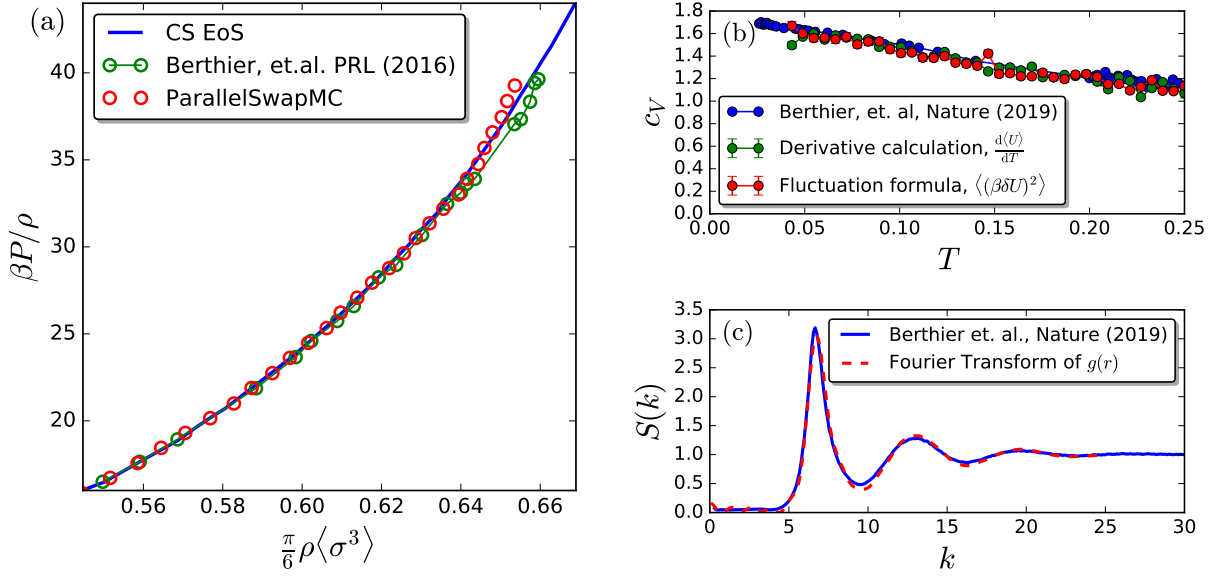

Figure S.9: (a) Equation of state calculation in 3D poly-disperse hard spheres as well as (b) specific heat capacity  $c_v$  and (c) Structure factor  $S(k)$  calculation for 2D poly-disperse soft disks.

implement the routine as a plug-in<sup>†</sup> for HOOMD-blue’s HPMC code, which runs in multi-CPU and gives us access to MC simulations in NPT ensemble used to confirm agreement with the Carnahan-Stirling equation of state for hard-spheres in 3D. For more detailed description of the scheme and neighbor list as implemented by HOOMD-blue, see [12] and relevant software documentation.

To ensure correct sampling, the code was tested on two previously studied polydisperse systems:

1. 3D poly-disperse hard spheres of [15]: we computed its equation of state (EoS) in NPT ensemble and compared it with the multi-component version of the Carnahan-Stirling EoS [16] and the data from [15].
2. 2D soft poly-disperse of [17]: we computed the specific heat capacity  $c_v$  as a function of temperature as well as the structure factor  $S(k)$  at a chosen reference temperature.

As shown in Fig. S.9, all replication studies show excellent agreement with reference data.

For equilibration of systems listed in Table 1, we prepared 40 independent trajectories per temperature and initially started with a temperature range of  $T \in [0.25, 0.025]$ . The range is then lowered or increased on a case-by-case basis. For the same range, we run simulations from  $10^4$  MCS to  $10^8$  MCS, where the latter is roughly near the maximum in which HOOMD-blue can be run un-interrupted. Probability to choose a swap move is set  $p_{\text{swap}} = 0.2$  and the number of CPU processes vary between four to six depending on available computing resources.

## 4.2 Inherent-State Sampling

After sampling a series of equilibrated configurations  $\{\mathbf{r}_\alpha\}$ , we obtain a series of inherent-state configurations  $\{\mathbf{R}_\alpha\}$  by local-energy minimization of every  $\{\mathbf{r}_\alpha\}$ . The FIRE algorithm was used with the settings recommended in Ref. [18], and happens to be the default setting in HOOMD-blue,

<sup>†</sup><https://github.com/mandadapu-group/parallel-swap-mc>

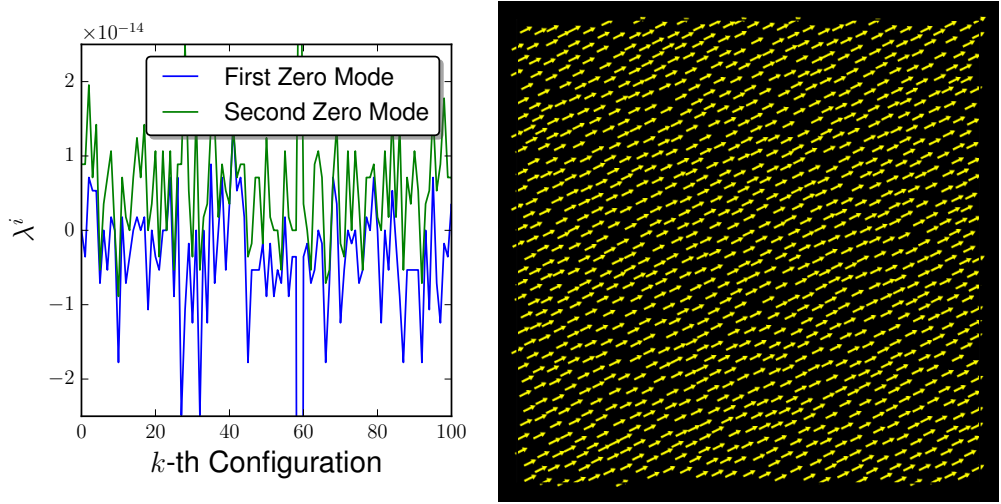

Figure S.10: (Left) The first two eigenvalues of sampled inherent states, showing that they belong to (numerically) zero modes. (Right) a typical zero eigenvector overlaid on the inherent-state configuration. Note that the eigenvector corresponds to a uniform translational shift, which is expected for zero modes arising from translational invariance.

but with the initial/maximum timestep changed to  $\Delta t_i = 0.05$  to  $0.075$ . Energy minimum is reached when

$$\frac{\sum_{\alpha=1}^N |\mathbf{F}_\alpha|}{N} \leq 10^{-6}; \quad \frac{|\Delta U|}{N} \leq 10^{-7} \quad (276)$$

where  $\Delta U$  is the change in potential energy every iteration. These tolerances are sufficient for the next set of calculations and there exist ways to check their sufficiency, as shown in the next section.

### 4.3 Shear Modulus Calculation

Let the shear modulus  $G^{\text{IS}} = C_{xyxy}^{\text{IS}}$ . Recall that there are two components for  $C_{ijkl}$

1. The Born part  $C_{ijkl}^B$  consists of pair-wise sum that can be easily computed inside a for-loop.
2. The non-affine part  $C_{ijkl}^{\text{NA}}$  consists of a calculation of  $\Xi_{ijk}^\alpha$ , which can be done in a simple for-loop, and the pseudo-inverse  $\mathbf{H}^+$ . From linear algebra, we know that  $\mathbf{H}^+$  for a symmetric real matrix like the Hessian  $\mathbf{H}$  is given by its eigendecomposition

$$\mathbf{H}^+ = \sum_{i=d+1}^{dN} \frac{\mathbf{v}^i \otimes \mathbf{v}^i}{\lambda^i}; \quad \lambda^i > 0. \quad (277)$$

Note that the sum starts at  $i = d + 1$  to exclude  $d$ -many zero modes ( $\lambda^i = 0$ ) that arise from translational invariance of the potential energy and no negative eigenvalues exist since inherent states are locally stable.

To obtain fast eigendecomposition analysis, we use code developed in-house\* and SLEPc [13] to achieve some degree of parallelization. Parallelized eigendecomposition is performed by the spectrum slicing method [19], where one can set a range  $[\lambda_{\min}, \lambda_{\max}]$  to compute eigenvalues, and each CPU process computes all eigenmodes within an independent portion of that range. We set

\*<https://github.com/mandadapu-group/pyglasstools>

$\lambda_{\min} = -1$  and  $\lambda_{\max} = 1.1 \times (\text{max. eigenvalue of } \mathbf{H})$ , and the latter is fast to compute prior to spectrum slicing. This range is used to confirm that inherent-state sampling is performed correctly, and that the solver can retrieve all zero eigenvalues (within tolerance) with no negative eigenvalues. An example of calculated zero modes is shown in Fig. S.10.

Empirically, we find that the smallest positive eigenvalues are larger than  $O(10^{-3})$  and thus, we set the tolerance for detecting zero eigenvalues as  $10^{-6}$ . Convergence for the  $i$ -th eigenmode is based on the 2-norm absolute error

$$\|\mathbf{H}\mathbf{v}^i - \lambda^i \mathbf{v}^i\|_2 < 10^{-6}. \quad (278)$$

Lower tolerance value ( $10^{-10}$ ) is also used with no changes to the results. Once all eigenmodes are obtained, one can compute the pseudo-inverse and thus, the non-affine part of  $C_{ijkl}$ . Before averaging the instantaneous shear modulus  $G = C_{xyxy}(\{\mathbf{R}_\alpha\})$  over all inherent-state configurations, the time-series of  $G$  is de-correlated through a sub-sampling scheme in [20], which is already implemented in the Python package `pymbar`. Following this scheme, 8000 to 10000 uncorrelated samples are available for averaging at every temperature. Fig. S.11 shows  $G^{\text{IS}}$  for all poly-disperse systems showcasing their linearity at low temperatures and thus, confirming a main assumption of the theory for matching  $\Delta F^\ddagger$  with  $J_\sigma$ .

The behavior of  $G^{\text{IS}}$  in Fig. S.11 in terms of linear behaviors at low temperatures crossing over to a plateau value at higher temperatures for all poly-disperse models motivates the following data-collapse procedure:

1. *Identify the high-temperature "plateau" regime* by using the RANSAC algorithm [21], which is implemented in the Python package `sklearn`. The RANSAC algorithm automatically detects the high-temperature regime by fitting a constant function  $f(T) = G_\infty^{\text{IS}}$  where  $G_\infty^{\text{IS}}$  is the plateau value of the shear modulus. The algorithm identifies an initial value for  $G_\infty^{\text{IS}}$  corresponding to an initial random subset of the data, and obtains the best fit by iteratively updating the subset. The final subset corresponds to all datapoints which are best described by a constant plateau value. This algorithm is useful in separating the plateau regime from the linear behavior at low temperatures.
2. *Fit the low-temperature regime and non-dimensionalize.* The low-temperature regime is identified again by the RANSAC algorithm using a linear function  $g(T) = a_-T + b_-$  for fitting. The shear modulus data can then be non-dimensionalized by defining

$$\Delta \tilde{G}^{\text{IS}} := \frac{G^{\text{IS}}(T) - G_\infty^{\text{IS}}}{G^{\text{IS}}(0) - G_\infty^{\text{IS}}}; \quad \tilde{T} := \frac{T}{T_p} \quad (279)$$

where  $G^{\text{IS}}(0) = b_-$  and  $T_p = -\frac{b_-}{a_-}$  is a cross-over temperature.

The result of this procedure is shown in Fig. S.12 where the shear modulus data for all poly-disperse models is collapsed with the following function

$$\Delta \tilde{G}^{\text{IS}}(\tilde{T}) = \begin{cases} 1 - \tilde{T} & \tilde{T} \leq 1 \\ 0 & \tilde{T} > 1. \end{cases} \quad (280)$$

Since  $\Delta F^\ddagger(T) \sim G^{\text{IS}}(T)$ , this result shows that energy barriers for excitation grows as temperature is being decreased below  $T_p$ . Note that  $T_p < T_o$  where  $T_o$  is the onset temperature. The cross-over temperature  $T_p$  identified from the shear modulus is similar to another cross-over temperature  $T_{\text{cross}}$  previously identified in an older study [22] using the mean-squared distance between the liquid configuration and its corresponding inherent state. Investigating the connection between  $T_p$  and  $T_{\text{cross}}$  and the physical meaning behind the cross-over behavior will be part of future work.

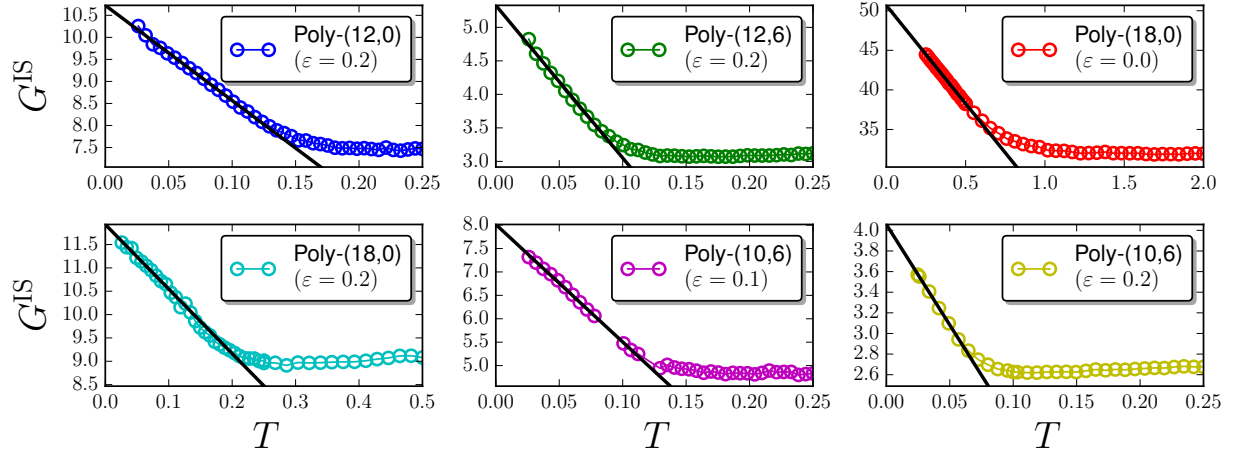

Figure S.11: Plot of inherent-state shear modulus  $G^{\text{IS}}$  as a function of temperature  $T$ . Black line is a linear fit to the low- $T$  portion of the data. Note that  $G^{\text{IS}}$  exhibits a high- $T$  plateau-like regime.

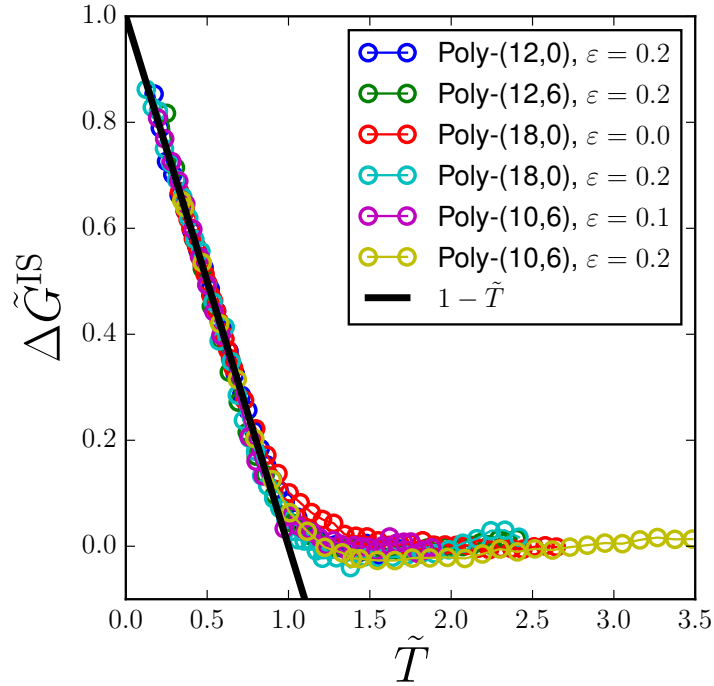

Figure S.12: The result of the data collapse procedure, confirming the linearity with respect to temperatures for  $T \leq T_p$  and the plateau regime for  $T > T_p$ . Note that  $T_p < T_o$  for all models considered in this work.

#### 4.4 Inherent-State RDF Calculation

For every discrete value of  $\tilde{r}_i$ , i.e., the center of the  $i$ -th binning window of size  $\delta r$ , the inherent-state RDF can be computed as

$$\tilde{g}^{\text{IS}}(\tilde{r}_i) \approx \frac{h(i)}{2\pi\rho\tilde{r}_i\Delta r N_{\text{conf}}N} \quad (281)$$

where  $h(i)$  is the histogram of binned pair distances  $\tilde{R}^{\alpha\beta} = R^{\alpha\beta}/\sigma_{\alpha\beta}$  at range  $[\tilde{r}_i - \Delta r/2, \tilde{r}_i + \Delta r/2]$  and  $N_{\text{conf}}$  is the number of inherent-state configurations used. The inherent-state RDFs for all models at different temperatures are shown in Fig. S.13. Due to the cut-off radius  $\tilde{r}_c$ , the virial pressure from Eq. (270) turns into

$$P^{\text{IS}} = -\frac{\pi\rho^2}{2} \int_0^\infty d\tilde{r} \tilde{r}^2 \phi_{\tilde{r}}(\tilde{r}) \tilde{g}^{\text{IS}}(\tilde{r}) = -\frac{\pi\rho^2}{2} \int_0^{\tilde{r}_c} d\tilde{r} \tilde{r}^2 [v_0 (\tilde{r}^{-m} - \tilde{r}^{-n}) + F(\tilde{r})] \tilde{g}^{\text{IS}}(\tilde{r}) \quad (282)$$

where the integration in the second equality is done through composite Simpson's rule. This calculation is then compared with one computed directly from averaging the inherent state averaged virial pressure

$$P^{\text{IS}} = \frac{1}{N_{\text{conf}}} \sum_{i=0}^{N_{\text{conf}}} \sum_{\alpha,\beta} \mathbf{F}_i^{\alpha\beta}(\mathbf{R}_i^{\alpha\beta}) \cdot \mathbf{R}_i^{\alpha\beta} \quad (283)$$

where the lower index  $i$  denotes the  $i$ -th sampled inherent-state configuration. As shown in Fig. S.14, excellent agreement can be found between both calculations.

From  $\tilde{g}^{\text{IS}}(\tilde{r})$ , the location of the PMF's first energy well and saddle point,  $\tilde{r}_{\text{min}}$  and  $\tilde{r}_{\text{max}}$ , were identified using Python function `scipy.signal.find_peaks`, followed by a high-order interpolating polynomial fit to the local region centered at the initial detected peaks. The peaks of these polynomials were then used for our final estimate of  $\tilde{r}_{\text{min}}$  and  $\tilde{r}_{\text{max}}$ . The result of the fitting process is shown for one sample PMF in Fig. S.15a. Note that local structure changes very little with respect to temperature and thus, the computed  $\tilde{u}^\dagger$  stays relatively constant, as shown in Fig. S.15b for Poly-(12,0). Together with  $G^{\text{IS}}$ , we compute  $\Delta F^\dagger(T)$  using Eq. (272) and fit the low-temperature calculation with a straight line  $a + bT$ . The intercept  $a$  is then used as the estimated  $J_\sigma$  of the current theory.

#### 4.5 MD Simulations and $\tau_{\text{eq}}(T)$ calculation

To compute the equilibrium relaxation time  $\tau_{\text{eq}}(T)$ , 40 independent MD simulations are performed under the NVT ensemble to equilibrate configurations and momenta using a plugin<sup>||</sup> implemented in HOOMD-blue. An initial temperature range of  $T \in [0.5, 0.1]$  is always used, which can be increased or decreased on a case-by-case basis. NVT is based on Nose-Hoover thermostat with timestep  $\Delta t = 0.0075$  and coupling constant  $\tau = \sqrt{\frac{Q}{gk_B T}} = 50\Delta t$ , where  $Q$  is the Nose mass and  $g = dN$  is the number of degrees of freedom. Subsequent NVE production runs with timestep  $\Delta t = 0.0075$  were used to compute equilibrium relaxation time  $\tau_{\text{eq}}$  from the self-part of intermediate scattering function,

$$F_s(\mathbf{k}, t) = \frac{1}{N} \left\langle \sum_{\alpha=1}^N \exp(i\mathbf{k} \cdot [\mathbf{r}_\alpha(t) - \mathbf{r}_\alpha(0)]) \right\rangle. \quad (284)$$

Letting  $\mathbf{k} = (k, \phi)$  and  $F_s(k, t) = \frac{1}{2\pi} \int_0^{2\pi} d\phi F_s((k, \phi), t)$ ,  $\tau_{\text{eq}}$  is defined such that  $F_s(k = \frac{2\pi}{\langle \sigma \rangle}, \tau_{\text{eq}}) = 0.1$ . Note that the length of time and temperature range for both equilibration and production runs

<sup>||</sup><https://github.com/mandadapu-group/polydisperse-md>

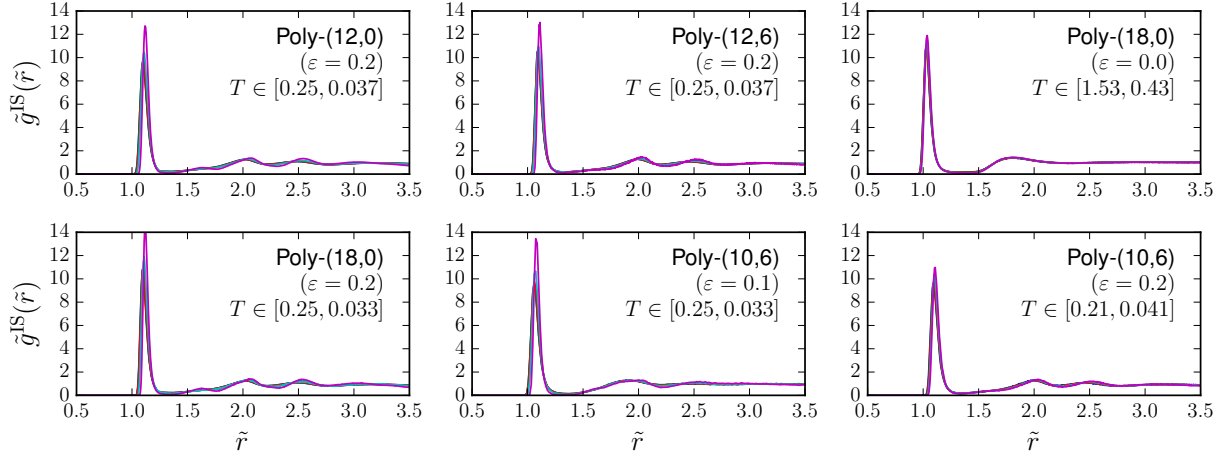

Figure S.13: Plot of inherent-state radial distribution functions for all models as computed by Eq. (281).

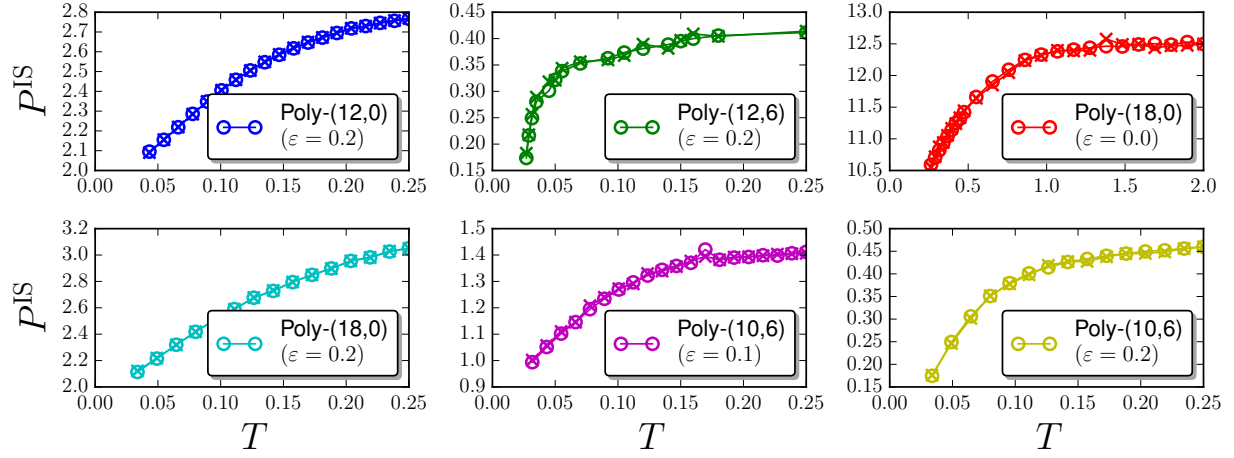

Figure S.14: Plot of inherent-state virial pressure for all models as computed by Eq. (282) ( $\circ$  marker) and Eq. (283) ( $\times$  marker).

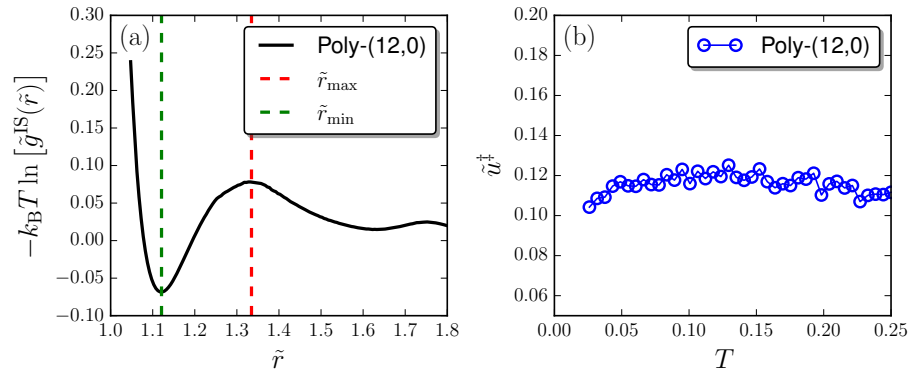

Figure S.15: (a) The PMF of Poly-(12,0) at  $T = 0.026$ , along with the location of the first energy well and saddle point. Note that  $\tilde{r}_{\min} \neq \langle \sigma \rangle = 1$ . (b) The computed  $\tilde{u}^\ddagger = \frac{1}{2}(\tilde{r}_{\max} - \tilde{r}_{\min})$  in Poly-(12,0) shows little change with temperature.

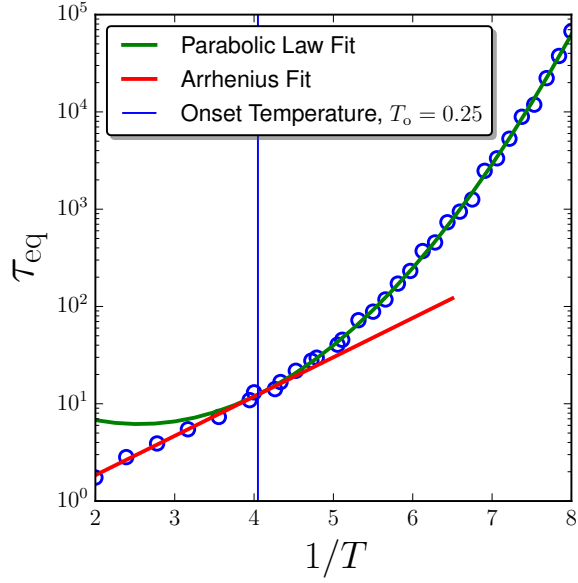

Figure S.16: A parabolic law fit to the equilibrium relaxation time data of Poly-(12,0).

are set by the  $\tau_{\text{eq}}(T)$  data: (1) NVT equilibration is run up to  $20\tau_{\text{eq}}$  to  $25\tau_{\text{eq}}$ , (2) NVE production is run up to  $5\tau_{\text{eq}}$ , to ensure accurate time-averaged estimate of  $F_s(k, t) = 0.1$ , and (3) temperature range is set so that we have measured  $\tau_{\text{eq}}$  roughly from  $10^{-1}$  to  $10^4$  orders in magnitude relative to  $\tau_{\text{eq}}(T = T_o)$ , where  $T_o$  is the onset temperature. Thus, two or three batches of MD simulations are needed to obtain  $\tau_{\text{eq}}(T)$  accurately within the desired temperature range.

The onset temperature  $T_o$  is estimated from fitting the parabolic law,

$$\ln \left[ \frac{\tau_{\text{eq}}}{\tau_o} \right] = \begin{cases} J^2(\beta - \beta_o)^2 + (\beta - \beta_o)E_a & \beta \geq \beta_o \\ (\beta - \beta_o)E_a & \beta < \beta_o \end{cases}, \quad (285)$$

to the equilibrium relaxation time  $\tau_{\text{eq}}(T)$  data. The fitting procedure is done by first fitting the high-temperature data with the Arrhenius term, fixing the fitted Arrhenius parameters, and then fitting the low-temperature data with the parabolic term in Eq. (285). High-temperature portion of the data is determined statistically, i.e., it is the number of high-temperature data points needed to maximize the  $R^2$  value of the low-temperature fitting. The typical result of such fitting procedure is shown in Fig. S.16.

From the parabolic law fitting, we also obtain  $J = \sqrt{\gamma/d_f} J_\sigma$ . Since  $d_f \approx 1.8$  in 2D, we could provide an alternative estimate for  $J_\sigma$ , once  $\gamma$  is determined through DF theory's trajectory analysis, as detailed in the next section.

#### 4.6 DF Theory Trajectory Analysis

We follow the procedure in [1], summarized in Section II of the main text, to compute  $J_\sigma$  from short-time particle trajectories. First, 250 independent trajectories are prepared from equilibrated MD simulations with step-size  $\Delta t = 0.002$  at a temperature range below  $T_o$ . We chose the range of temperatures below a temperature corresponding to a  $\tau_{\text{eq}}$  that is at least ten times higher than  $\tau_{\text{eq}}$

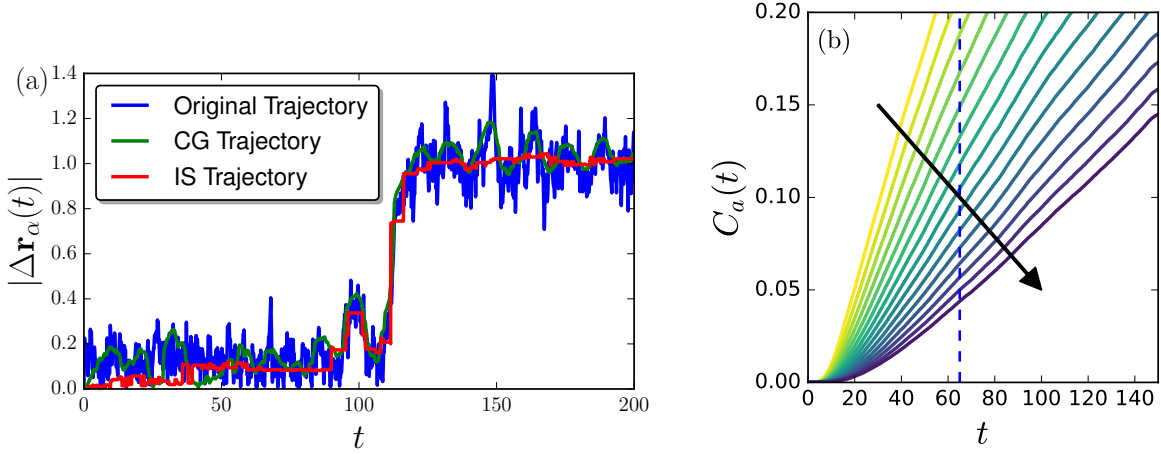

Figure S.17: (a) The trajectory of a single particle at  $T = 0.137 < T_o$  for Poly-(12,0) compared with its coarse-grained (CG) and inherent-state (IS) trajectory. (b) The dynamic observable  $C_a(t)$  for Poly-(12,0) computed at  $T = 0.239$ . Black arrow shows the progression in increasing  $a$ , and the vertical line indicates the chosen observation time  $t_a$  for this system.

at onset temperature  $T_o$ . Excitation statistics are probed using the dynamic observable

$$C_a(t) = \left\langle \frac{1}{N} \sum_{\alpha=0}^N \Theta(|\bar{\mathbf{r}}_{\alpha}(t) - \bar{\mathbf{r}}_{\alpha}(0)| - a) \right\rangle \quad (286)$$

where  $N$  is the number of particles,  $\langle \dots \rangle$  is equilibrium ensemble average,  $\bar{\mathbf{r}}_{\alpha}(t)$  is the position of the  $\alpha$ -th particle coarse-grained over a small time window  $\delta t$ , and  $\Theta(x) = 1$  if  $x > 0$  and zero otherwise.  $C_a$  is always computed at a range of  $a \in [0.2, 1.0]$  with final time  $t_f = 150$ . Coarse-graining in time is done through a median filter, i.e., a low-pass filter that can preserve step changes in a signal, with the time window set to  $\delta t = 5$ . A range of time windows  $\delta t \in [2, 12]$  have also been tried with little to no change in the result.

The rate of excitation events at temperature  $T$  is computed as  $c_a(T) = C_a(t_a; T)/t_a$ , where  $C_a(t; T)$  is the dynamic observable computed per Eq. (286) at temperature  $T$ , and  $t_a$  is an observation time that lies within the linear regime of  $C_a(t)$ . The energy barrier  $J_a$  computed from  $c_a(T)$  is insensitive to the choice of  $t_a$  so long that it is within the linear regime of  $C_a(t)$ , which is demonstrated in Fig. S.17 for Poly-(12,0). The typical values of chosen  $t_a \in [25, 80]$  for all models. In Ref. [1], the quantity  $C_a(t_a)/t_a$  is equivalent to Eq. (6) of Sec. B, and the linearity of  $C_a(t)$  with respect to time  $t$  was measured through a function  $R(t)$ , which measures the slope of  $C_a(t)$ ; see Fig. 2 of Ref. [1] where the linear regime is reflected as a constant plateau in  $R(t)$ . The function  $R(t)$  also measures the excitation event at an individual-particle level, in contrast to the averaging over all particles in  $C_a(t)$ . Thus, if there exists a range of timescales for which a constant plateau is observed in  $R(t)$ , then separation of timescales exists at the level of a single particle, and particle displacements form rare hopping events. In such a case, the computed energy barrier  $J_a$  is insensitive to the choice of  $t_a$  so long that  $t_a$  is chosen within the linear regime of  $C_a(t)$ .

Figure S.18 confirms the Arrhenius behavior of  $c_a$  in all poly-disperse models. From the computed  $J_a$  at every  $a$ , its logarithmic relation

$$J_a - J_{\sigma} = \gamma J_{\sigma} \ln(a/\sigma) \quad (287)$$

is also confirmed in Fig. S.19a, where we collapse the data for all poly-disperse systems using the

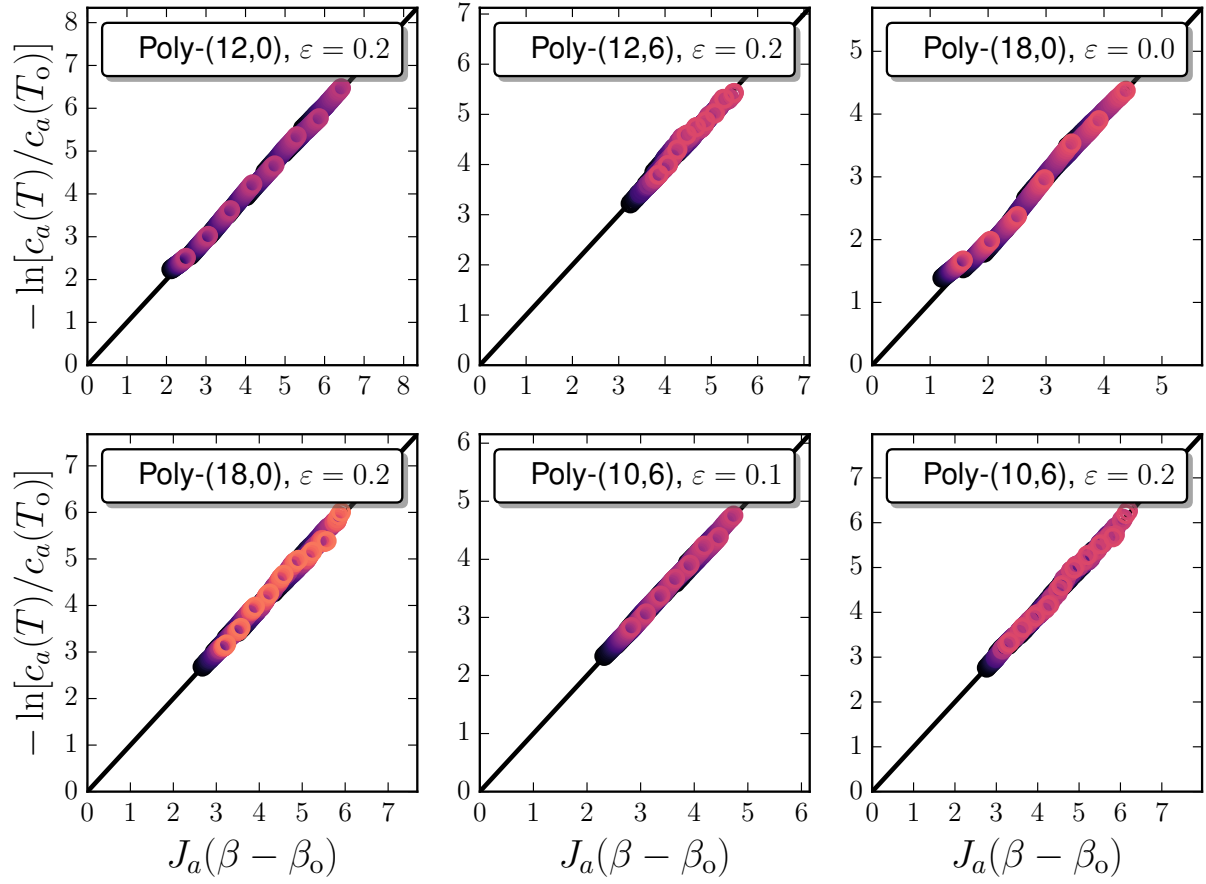

Figure S.18: Plot of  $-\ln[c_a]$  vs.  $\beta = 1/k_B T$  for all  $a$ . The data is collapsed using the onset temperature  $\beta_o = 1/k_B T_o$  and fitting the slope  $J_a$  using Arrhenius formula for the concentration of excitations [1]. Light-to-dark indicates small-to-large values in displacement magnitude  $a$ .

$J_\sigma$  and  $\gamma$  values obtained by fitting procedures. Lastly, the computed  $J_\sigma$  and  $\gamma$  is used to collapse the relaxation time data, as shown in Fig. S.19b. The estimated  $J_\sigma$  from fitting the logarithmic relation can be compared with one from parabolic law fitting and the current theory; see Table 2 of the main text.

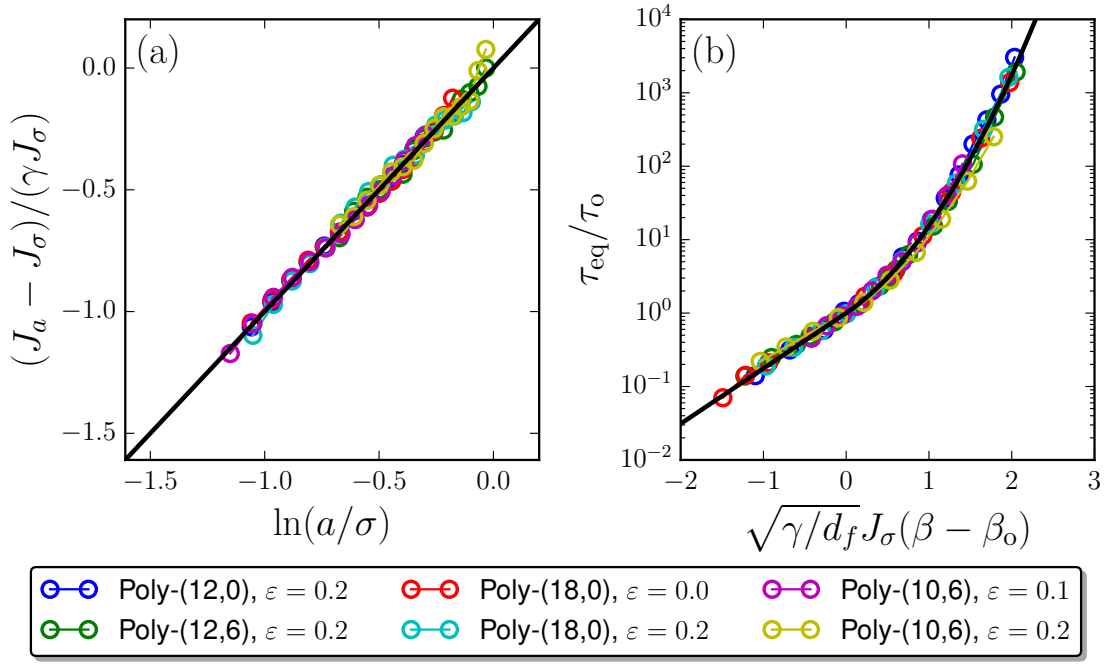

Figure S.19: (a) A plot of  $J_a$  vs. displacement magnitude  $a$ , which is collapsed according to the logarithmic relation in Eq. (287). (b) An Arrhenius plot of equilibrium relaxation time  $\tau_{\text{eq}}$ , where all data are collapsed according to the parabolic law (Eq. (285)). Note that the  $J_\sigma$  and  $\gamma$  used for collapsing  $\tau_{\text{eq}}$  are computed from data shown in Fig. S.18 and (a).

## References

- [1] Keys, A. S., Hedges, L. O., Garrahan, J. P., Glotzer, S. C. & Chandler, D. Excitations are localized and relaxation is hierarchical in glass-forming liquids. *Phys. Rev. X* **1**, 021013 (2011).
- [2] Stillinger, F. H. & Weber, T. A. Hidden structure in liquids. *Phys. Rev. A* **25**, 978 (1982).
- [3] Torres-Sánchez, A., Vanegas, J. M. & Arroyo, M. Geometric derivation of the microscopic stress: A covariant central force decomposition. *J. Mech. Phys. Solids* **93**, 224–239 (2016).
- [4] Karmakar, S., Lerner, E. & Procaccia, I. Athermal nonlinear elastic constants of amorphous solids. *Physical Review E* **82**, 026105 (2010).
- [5] Lutsko, J. Generalized expressions for the calculation of elastic constants by computer simulation. *J. App. Phys.* **65**, 2991–2997 (1989).
- [6] Balluffi, R. W. *Introduction to Elasticity Theory for Crystal Defects* (Cambridge University Press, 2012).
- [7] Lemaître, A. Structural relaxation is a scale-free process. *Phys. Rev. Lett.* **113**, 245702 (2014).
- [8] Gradshteyn, I. S. & Ryzhik, I. M. *Table of Integrals, Series, and Products* (Academic press, 2014).
- [9] Hansen, J.-P. & McDonald, I. R. *Theory of Simple Liquids* (Academic Press, 2005).
- [10] Irving, J. & Kirkwood, J. G. The statistical mechanical theory of transport processes. IV. The equations of hydrodynamics. *J. Chem. Phys.* **18**, 817–829 (1950).
- [11] Ninarello, A., Berthier, L. & Coslovich, D. Models and algorithms for the next generation of glass transition studies. *Phys. Rev. X* **7**, 021039 (2017).
- [12] Anderson, J. A., Irrgang, M. E. & Glotzer, S. C. Scalable Metropolis Monte Carlo for simulation of hard shapes. *Comput. Phys. Commun.* **204**, 21–30 (2016).
- [13] Hernandez, V., Roman, J. E. & Vidal, V. SLEPc: A scalable and flexible toolkit for the solution of eigenvalue problems. *ACM Trans. Math. Softw.* **31**, 351–362 (2005).
- [14] Anderson, J. A., Jankowski, E., Grubb, T. L., Engel, M. & Glotzer, S. C. Massively parallel Monte Carlo for many-particle simulations on GPUs. *J. Comput. Phys.* **254**, 27–38 (2013).
- [15] Berthier, L., Coslovich, D., Ninarello, A. & Ozawa, M. Equilibrium sampling of hard spheres up to the jamming density and beyond. *Phys. Rev. Lett.* **116**, 238002 (2016).
- [16] Mansoori, G. A., Carnahan, N. F., Starling, K. E. & Leland, T. W. Equilibrium thermodynamic properties of the mixture of hard spheres. *J. Chem. Phys.* **54**, 1523–1525 (1971).
- [17] Berthier, L., Charbonneau, P., Ninarello, A., Ozawa, M. & Yaida, S. Zero-temperature glass transition in two dimensions. *Nat. Comm.* **10**, 1508 (2019).
- [18] Bitzek, E., Koskinen, P., Gähler, F., Moseler, M. & Gumbusch, P. Structural relaxation made simple. *Phys. Rev. Lett.* **97**, 170201 (2006).
- [19] Romero, E. & Roman, J. E. A parallel implementation of Davidson methods for large-scale eigenvalue problems in SLEPc. *ACM Trans. Math. Software* **40**, 13:1–13:29 (2014).

- [20] Chodera, J. D., Swope, W. C., Pitera, J. W., Seok, C. & Dill, K. A. Use of the weighted histogram analysis method for the analysis of simulated and parallel tempering simulations. *J. Chem. Theory Comput.* **3**, 26–41 (2007).
- [21] Fischler, M. A. & Bolles, R. C. Random sample consensus: a paradigm for model fitting with applications to image analysis and automated cartography. *Commun. ACM* **24**, 381–395 (1981).
- [22] Sastry, S., Debenedetti, P. G. & Stillinger, F. H. Signatures of distinct dynamical regimes in the energy landscape of a glass-forming liquid. *Nature* **393**, 554–557 (1998).
